# Supplementary material for: Federated Multi-Sequence Stochastic Approximation with Local Hypergradient Estimation
Source: arXiv:2306.01648 source file (2023-06-02)
Supplement: Supplementary file 2 [file supp_compos.tex]

\section{Proof for Federated MSA}\label{sec:app:msa}
The deviation of $\m{h}_r$ from  $\nabla f(\m{x}_r, \m{Z}_r)$  can be bounded by
the following lemma.

\subsection{Main Sequence Analysis}
\begin{lemma}[\textbf{Descent Lemma}]\label{lem:dec}
Suppose Assumptions~\ref{assum:lip:y*}--\ref{assum:lipmaps} hold. Then, for client $\tilde{m}$ sampled at $k$--th local iteration, Algorithm~\ref{alg:fedmsa} guarantees: 
\begin{equation}\label{eqn0:lem:dec}
 \begin{aligned}
f(\m{x}_{r+1,k+1}^{\tilde{m}})-f(\m{x}_{r+1,k}^{\tilde{m}}) \leq
 &-  \frac{3 \alpha_k} {4} \left(1- 2\alpha_k L_{\m{h}}\right) \left\| \m{h} (\m{x}_{r+1,k}^{\tilde{m}}) \right\|^2 \\
  &+ \frac{\alpha_k}{2} \left(2+  3\alpha_k L_{\m{h}}\right)  \left\| \m{h}^{\tilde{m}}_{r,k}- \m{h} (\m{x}_{r+1,k}^{\tilde{m}}, \m{Z}_{r+1,k}^{\tilde{m}} ) \right\|^2 \\
  % &  3\alpha_k^2 \left(  \left\| \m{h}^{\tilde{m}}_{r,k}- \nabla f (\m{x}_{r+1,k}^{\tilde{m}}, \m{Z}_{r+1,k}^{\tilde{m}} ) \right\|^2+ \left\| \nabla f  (\m{x}_{r+1,k}^{\tilde{m}}) \right\|^2 \right)\\
    &+ \frac{ \alpha_k L_{\m{h},\m{z}}^2 N}{2} \left(2+ 3\alpha_k L_{\m{h}}\right) \sum_{n=1}^N L^2_{\m{z}}(n) \left\|\m{z}_{r+1,k}^{m,n}-\m{z}^{n,*}(\m{z}_{r+1,k}^{m,n-1})\right\|^2.
\end{aligned}
\end{equation}
\end{lemma}
\begin{proof}
From  Algorithm~\ref{alg:fedmsa} and 
% , and
%  \begin{align}\label{eqn1:lem:dec}
%      \m{x}_{r+1}&=\m{x}_{r}- \frac{\alpha}{M} \sum\limits_{m=1}^{M}  \sum\limits_{k=0}^{K-1} \m{h}^{\tilde{m}}_{r,k}
%  \end{align}
% Now, using 
the Lipschitz property of $\m{h}(\m{x})$, we have
\begin{equation} \label{eqn1:lem:dec}
\begin{aligned}
f(\m{x}_{r+1,k}^{\tilde{m}}) 
    & \leq  f(\m{x}_{r,k}^{\tilde{m}})+ \left\langle \m{x}_{r+1,k+1}^{\tilde{m}} - \m{x}_{r+1,k}^{\tilde{m}}, \m{h}(\m{x}_{r+1,k}^{\tilde{m}}) \right \rangle + \frac{\alpha^2 L_{\m{h}}}{2} \left\|\m{h}_{r,k}^{\tilde{m}}\right\|^2\\
    & \leq  f(\m{x}_{r,k}^{\tilde{m}})+ \left\langle \m{h}_{r,k}^{\tilde{m}}, \m{h}(\m{x}_{r+1,k}^{\tilde{m}}) \right \rangle + \frac{\alpha^2 L_{\m{h}}}{2} \left\|\m{h}_{r,k}^{\tilde{m}}\right\|^2.
    %\\
   % & = + \mb{E}\left[ \left\langle \frac{\alpha}{M}\sum\limits_{m=1}^{M} \sum\limits_{k=0}^{K-1} \m{h}^m(\m{x}^m_{k}, \m{y}^m_{k}, \m{z}^m_{k}) , \nabla f(\m{x}) \right\rangle \right]\\
    %&+ \frac{L_f}{2}  \mb{E}\left[ \left\| \frac{\alpha}{M}\sum\limits_{m=1}^{M} \sum\limits_{k=0}^{K-1} \m{h}^m(\m{x}^m_{k}, \m{y}^m_{k},\m{z}^m_{k})\right\|^2\right].
\\
&\leq f(\m{x}_{r,k})-\frac\alpha2\|\nabla f(\m{x}_{r,k})\|^2 - \frac\alpha2\|\m{h}_{r,k}^{\tilde{m}}\|^2 + \frac\alpha2 \|\nabla f(\m{x}_{r,k})-\m{h}_{t,k}^{\tilde{m}}\|^2 + \alpha^2 \frac{L^h}2\|\m{h}_{r,k}\|^2\\
        &\leq f(x^{t,k}) - \frac\alpha2\|\nabla f(\m{x}_{r,k})\|^2 - \frac\alpha2\|\m{h}_{r,k}^{\tilde{m}}\|^2 + \alpha \|\nabla f(x_{r,k})-\m{h}(\m{u}_{r,k})\|^2 \\\nonumber
        &\qquad + \alpha \|\m{h}(\m{u}_{r,k}^{\tilde{m}})-\m{h}_{r,k}^{\tilde{m}}\|^2 + \alpha^2 \frac{L^h}2\|\m{h}_{r,k}^{\tilde{m}}\|^2\enspace.
    \end{aligned}
%\label{eqn2:lem:dec}
\end{equation}
Now, Assumption~\ref{assum:lipmaps} implies
\begin{equation} \label{eqn2:lem:dec}
\begin{aligned}
f(\m{x}_{r+1,k}^{\tilde{m}}) 
    % & \leq f(\m{x}_{r,k}) - \frac\alpha2\|\nabla f(\m{x}_{r,k})\|^2 - \frac\alpha2\|\m{h}_{r,k}^m\|^2 + \alpha \|\nabla f(x_{r,k})-\m{h}(\m{u}_{r,k})\|^2 \\\nonumber
    %     &\qquad + \alpha \|\m{h}(\m{u}^{t,k})-\m{h}_{r,k}^m\|^2 + \alpha^2 \frac{L^h}2\|\m{h}_{r,k}^m\|^2\enspace.
    %     \\
        & \leq f(\m{x}_{r,k}^{\tilde{m}})  - \frac\alpha2\|\nabla f(\m{x}_{r,k}^{\tilde{m}})\|^2 +\alpha L_x^2(\mb{E}[\|\m{z}_{r,k}^{\tilde{m}} - \m{z}^*(\m{x}_{r,k}^{\tilde{m}})\|^2] + \mb{E}[\|\m{w}_{r,k}^{\tilde{m}} -\m{w}^*(\m{x}_{r,k}^{\tilde{m}})\|^2]) \\
        &+ \alpha \mb{E}[\|\m{h}(\m{u}_{t,k}^{\tilde{m}})-\m{h}_{r,k}^{\tilde{m}}\|^2]- \frac\alpha2\left(1-L^h\alpha\right) \mb{E}[\|\m{h}_{r,k}^{\tilde{m}}\|^2]\enspace.
    \end{aligned}
%\label{eqn2:lem:dec}
\end{equation}
Taking expectations and using  $\alpha \leq 1/L^h$, we get the final result. 

In the following, we bound each term on the right hand side (RHS) of~\eqref{eqn1:lem:dec}. Let 
\begin{equation*}%\label{eq}
\m{a}^{\tilde{m}}_{r,k}:=\m{h}^{\tilde{m}}_{r,k}- \m{h}(\m{x}_{r+1,k}^{\tilde{m}}, \m{Z}_{r+1,k}^{\tilde{m}} ) + \m{h} (\m{x}_{r+1,k}^{\tilde{m}}, \m{Z}_{r+1,k}^{\tilde{m}} ) - \m{h}(\m{x}_{r+1,k}^{\tilde{m}}) + \m{h} (\m{x}_{r+1,k}^{\tilde{m}}).
\end{equation*}
For the first term on the RHS of~\eqref{eqn1:lem:dec}, we have 
%$\m{x}_{r+1,k}^m - \m{x}_{r,k}^m =  \m{h}^m_{r,k} $ w
% Not that by our Assumption, we have $ \m{h}^m (\m{x}_{r+1,k}^m, \m{Z}_{r+1,k}^m ) =  \nabla f^m (\m{x}_{r+1,k}^m, \m{Z}_{r+1,k}^m )+ \xi_{r,k}^m$. 
%For the first term, we have $\m{x}_{r+1,k}^m - \m{x}_{r,k}^m =  \m{h}^m_{r,k} + $
%Further, for the second term in RHS of \eqref{eqn3:lem:dec}, we have
\begin{equation}\label{eqn2:lem:dec}
\begin{aligned}
 \left\langle \m{x}_{r+1,k+1}^{\tilde{m}} - \m{x}_{r,k}^{\tilde{m}}, \m{h}(\m{x}_{r+1,k}^{\tilde{m}}) \right\rangle &= - \alpha_k \left\langle \m{a}^{\tilde{m}}_{r,k}, \m{h}  (\m{x}_{r+1,k}^{\tilde{m}}) \right\rangle \\
  &\leq  \alpha_k \left\| \m{h}^{\tilde{m}}_{r,k}- \m{h}(\m{x}_{r+1,k}^{\tilde{m}}, \m{Z}_{r+1,k}^{\tilde{m}} ) \right\|^2\\
  &+  \alpha_k \left\|\m{h}(\m{x}_{r+1,k}^{\tilde{m}}, \m{Z}_{r+1,k}^{\tilde{m}} )- \m{h} (\m{x}_{r+1,k}^{\tilde{m}}) \right\|^2- \frac{3\alpha_k}{4} \left\| \m{h}  (\m{x}_{r+1,k}^{\tilde{m}})\right\|^2 
% &=\alpha_k \left\| \m{h}^m_{r,k}- \m{h}(\m{x}_{r+1,k}^m, \m{Z}_{r+1,k}^m ) \right\|^2 \\
 %&+   L_{\m{h,z}}^2 N  \alpha_k \sum_{n=1}^N L^2_z(n) \left\|\m{z}_{r,k}^{m,n} - \m{z}_{r}^{n,*}\right\|^2 -\frac{3\alpha_k}{4}  \left\|\m{h}(\m{x}_{r+1,k}^m) \right\|^2 .
\end{aligned}
%\label{eqn5:lem:dec}
\end{equation}
\ps{Maybe $-\alpha_k/2$ rather than $-3\alpha_k/4$ in last term?}
Following \citep[Lemma~8]{shen2022single}, we get
\begin{align}\label{eqn:lem:dec:lip}
    \left\|\m{h}(\m{x}_{r+1,k}^{\tilde{m}},\m{Z}_{r+1,k}^{\tilde{m}})- \m{h}(\m{x}_{r+1,k}^{\tilde{m}})\right\|\leq L_{\m{h,z}} \sum_{n=1}^N L_{\m{z}}(n) \left\|\m{z}_{r+1,k}^{\tilde{m},n}-\m{z}^{n,*}(\m{z}_{r+1,k}^{\tilde{m},n-1})\right\|.
\end{align}
where $L_\m{z}(n):=  \sum_{i=n}^{N} L_{\m{z},i-1} L_{\m{z},i-2}\dots L_{\m{z},n} $ with $L_{\m{z},n-1} L_{\m{z},n-2}\dots L_{\m{z},n} = 1$ for any $n \in [N]$. 

This together with \eqref{eqn2:lem:dec} implies that 
\begin{equation}\label{eqn20:lem:dec}
\begin{aligned}
 \left\langle \m{x}_{r+1,k+1}^{\tilde{m}} - \m{x}_{r,k}^{\tilde{m}}, \m{h}(\m{x}_{r+1,k}^{\tilde{m}}) \right\rangle &\leq \alpha_k \left\| \m{h}^{\tilde{m}}_{r,k}- \m{h}(\m{x}_{r+1,k}^{\tilde{m}}, \m{Z}_{r+1,k}^{\tilde{m}} ) \right\|^2 \\
 &+   L_{\m{h,z}}^2 N  \alpha_k \sum_{n=1}^N L^2_z(n) \left\|\m{z}_{r+1,k}^{m,n} -\m{z}^{n,*}(\m{z}_{r+1,k}^{m,n-1})\right\|^2 -\frac{3\alpha_k}{4}  \left\|\m{h}(\m{x}_{r+1,k}^{\tilde{m}}) \right\|^2 .
\end{aligned}
%\label{eqn5:lem:dec}
\end{equation}\
% For the first term, we have
% %Further, for the second term in RHS of \eqref{eqn3:lem:dec}, we have
% \begin{equation}%\label{lemma12:eqn7}
% \begin{aligned}
%  &\left\langle \frac{\alpha}{M}\sum\limits_{m=1}^{M} \sum\limits_{k=0}^{K-1}  \m{h}^m(\m{x}^m_{k},\m{Z}^m_{k}), \m{h}(\m{x}) \right\rangle \\
%  &\geq \frac{\alpha}{MK}\sum\limits_{m=1}^{M}  \sum\limits_{k=0}^{K-1} \left\langle \m{h}^m(\m{x}^m_{k}, \m{y}^m_{k},\m{z}^m_{k}) -\m{h}(\m{x}), \m{h}(\m{x}) \right\rangle +  \alpha\left\|\nabla f(\m{x})\right\|^2 \\
%  &\leq  \frac{\alpha}{MK}\sum\limits_{m=1}^{M} \sum\limits_{k=0}^{K-1}  L_{h}\left\|\nabla f(\m{x}) \right\|   \left( L_y\left\| \m{y}^m_{k}-  \m{y}^*\right\| + L_z\left\|\m{z}^m_{k}- \m{z}^*\right\| \right) - \alpha\left\|\nabla f(\m{x})\right\|^2 \\
%  &=-\frac{3\alpha}{4}  \left\|\nabla f(\m{x}) \right\|^2 +  \frac{\alpha}{MK}\sum\limits_{m=1}^{M} \sum\limits_{k=0}^{K-1}  L_h\left(L_y\left\| \m{y}^m_{k}-  \m{y}^*\right\| + L_z\left\|\m{z}^m_{k}- \m{z}^*\right\| \right)
% \end{aligned}
% \label{eqn5:lem:dec}
% \end{equation}
% Further, we have 
% \begin{equation}
%  \begin{aligned}
%  - \mb{E}\left\langle \nabla f(\m{x}_{r+1,k}^{\tilde{m}}) , \alpha_k \xi_{r,k}^{\tilde{m}} \right\rangle \leq \frac{\alpha^2_k}{4}\mb{E}\left\| \nabla f(\m{x}_{r+1,k}^{\tilde{m}}) \right\| + \alpha^2_k \tilde{\sigma}_f^2,
%     \end{aligned}
% \label{eqn6:lem:dec}
% \end{equation}
%
%
Similarly, for the second term on the RHS of~\eqref{eqn2:lem:dec}, we have
\begin{equation}\label{eqn3:lem:dec}
\begin{aligned}
\left\|\m{x}_{r+1,k+1}^{\tilde{m}} - \m{x}_{r+1,k}^{\tilde{m}}\right\|^2  &\leq 3\alpha_k^2 \left(  \left\| \m{h}^{\tilde{m}}_{r,k}- \m{h}(\m{x}_{r+1,k}^{\tilde{m}}, \m{Z}_{r+1,k}^{\tilde{m}} ) \right\|^2+ \left\| \m{h} (\m{x}_{r+1,k}^{\tilde{m}}) \right\|^2 \right)\\
    & +3\alpha_k^2 \left\|\m{h}(\m{x}_{r+1,k}^{\tilde{m}}, \m{Z}_{r+1,k}^{\tilde{m}} )- \m{h} (\m{x}_{r+1,k}^{\tilde{m}}) \right\|^2\\ 
        & \leq 3\alpha_k^2\left(  \left\| \m{h}^{\tilde{m}}_{r,k}- \m{h}(\m{x}_{r+1,k}^{\tilde{m}}, \m{Z}_{r+1,k}^{\tilde{m}} ) \right\|^2+ \left\| \m{h} (\m{x}_{r+1,k}^{\tilde{m}}) \right\|^2 \right)\\
        &+ 3\alpha_k^2 L_{\m{h},\m{z}}^2 N \sum_{n=1}^N L^2_z(n) \left\|\m{z}_{r+1,k}^{\tilde{m},n}-\m{z}^{n,*}(\m{z}_{r+1,k}^{\tilde{m},n-1})\right\|^2.
    \end{aligned}
\end{equation}

Plugging \eqref{eqn3:lem:dec} and \eqref{eqn2:lem:dec} into \eqref{eqn1:lem:dec} completes the proof.
\end{proof}

%\subsection{Proof of Theorem~\ref{thm:fednest}}
%\subsection{Drifting Errors  }

The following lemma provides a bound on the \textit{drift} of each $(\m{x}^{\tilde{m}}_{r+1,k}, \m{Z}_{r+1,k}^{\tilde{m}})$ from $(\m{x}_{r+1}, \m{Z}_{r})$ for stochastic MSA problems. 

\begin{lemma}[\textbf{Drifting Error}]\label{lem:drift:fedmsa}
Suppose Assumptions~ \ref{assum:lip:y*}--\ref{assum:stmonot:g} hold. %Further, assume $K \geq 1$ and $ \alpha^{m}_k\leq 1/(5M_fK), \forall m \in \mathcal{S}$. 
Then, for each $m \in [M]$ and $ k \in [K]$,  Algorithm~\ref{alg:fedmsa} guarantees:
\begin{equation}
\begin{aligned}\label{eqn1:lem:drift:fedmsa}
\left\|\m{x}^{m}_{r+1,k}-\m{x}_r\right\|^2 & \leq  2 e \alpha_k^2 (1+K) \sum\limits_{k=1}^{K-1}  \left\| \m{h}^m_{r,k}- \m{h} (\m{x}_{r+1,k}^m, \m{Z}_{r+1,k}^m) \right\|^2\\
       &+ 2 e \alpha_k^2 (1+K) \sum\limits_{k=1}^{K-1} \left\| \m{h} (\m{x}_{r+1,k}^m, \m{Z}_{r+1,k}^m ) \right\|^2,
%2 e K^2 \alpha_k^2 \mb{E} \left\| \m{h}_r- \m{h}(\m{x}_r, \m{Z}_{r})\right\|^2+\frac{10 e K \alpha_k^2 }{6} \sum_{k=1}^K \mb{E}\left\| \m{h}(\m{x}_{r+1,k}^m, \m{Z}_{r+1,k}^m)\right\|.
\end{aligned} 
\end{equation}
where $e:=\exp(1)$.
\end{lemma}
\begin{proof}
From  Algorithm~\ref{alg:fedmsa}, we have that $\forall m\in [M]$,
\begin{equation}
\label{eqn2:lem:drift:fedmsa}
\begin{aligned}
 \left\|\m{x}^{m}_{r+1,k}-\m{x}_r\right\|^2 &\leq  \left(1+\frac{1}{K}\right)\|\m{x}_{r+1,k-1}^m-\m{x}_r\|^2+ (K+1)\alpha_k^2 \left\|\m{h}_{r,k-1}^m\right\|^2\\
        & \leq  \left(1+\frac{1}{K}\right)\|\m{x}_{r+1,k-1}^m-\m{x}_r\|^2
        \\
        &+  2\alpha_k^2 (1+K)  \left\|\m{h}(\m{x}_{r+1,k-1}^m, \m{Z}_{r+1,k-1}^m ) \right\|^2
        %+ 3\alpha_k^2 (1+K)  L_{\m{h},\m{z}}^2 N \sum_{n=1}^N L^2_z(n)\|\m{z}_{r+1,k-1}^{m,n}-\m{z}_{r}^{n,*}\|^2
        \\
       &+ 2\alpha_k^2 (1+K)  \left\| \m{h}^m_{r,k-1}- \m{h} (\m{x}_{r+1,k-1}^m, \m{Z}_{r+1,k-1}^m ) \right\|^2
    \end{aligned}
\end{equation}
where the last inequality uses \eqref{eqn3:lem:dec}.

Now, iterating equation \eqref{eqn2:lem:drift:fedmsa} and using $  \m{x}^{m}_{r+1,1}=\m{x}^{m}_{r+1,0}=\m{x}_r ~~\forall m\in [M]$, we obtain
\begin{equation}
\label{eqn3:lem:drift:fedmsa}
\begin{aligned}
 \left\|\m{x}^{m}_{r+1,k}-\m{x}_r\right\|^2
% leq  \left(1+\frac{1}{K}\right)\|\m{x}_{r+1,k-1}^m-\m{x}_r\|^2+ (K+1)\alpha_k^2 \left\|\m{v}_{r,k-1}^m\right\|^2\\
%&\leq  \left(1+\frac{1}{K}\right)\|\m{x}_{r+1,k}^m-\m{x}_r\|^2\\
%&+ 3 \alpha_k^2 (1+K) \left\|\m{h} (\m{x}_{r+1,k}^m, \m{Z}_{r+1,k}^m )- \m{h}  (\m{x}_{r+1,k}^m) \right\|^2\\ 
      %  & \leq  %3\alpha_k^2 (1+K) \sum\limits_{j=2}^{k} \left(1+\frac{1}{K+1}\right)^j  L_{\m{h},\m{z}}^2 N \sum_{n=1}^N L^2_z(n)\|\m{z}_{r+1,j-1}^{m,n}-\m{z}^{n,*}\|^2
       % \\
       &\leq  2\alpha_k^2 (1+K) \sum\limits_{j=2}^{k} \left(1+\frac{1}{K+1}\right)^j  \left\| \m{h}^m_{r,j-1}- \m{h} (\m{x}_{r+1,j-1}^m, \m{Z}_{r+1,j-1}^m) \right\|^2\\
       &+ 2\alpha_k^2 (1+K) \sum\limits_{j=2}^{k} \left(1+\frac{1}{K+1}\right)^j \left\| \m{h} (\m{x}_{r+1,j-1}^m, \m{Z}_{r+1,j-1}^m)  
       \right\|^2. 
\end{aligned}
\end{equation}
Since $\sum\limits_{j=2}^{k} \left(1+\frac{1}{K+1}\right)^j \leq  \exp(1)$. We have 
\begin{equation}
\label{eqn4:lem:drift:fedmsa}
\begin{aligned}
 \left\|\m{x}^{m}_{r+1,k}-\m{x}_r\right\|^2
% leq  \left(1+\frac{1}{K}\right)\|\m{x}_{r+1,k-1}^m-\m{x}_r\|^2+ (K+1)\alpha_k^2 \left\|\m{v}_{r,k-1}^m\right\|^2\\
%&\leq  \left(1+\frac{1}{K}\right)\|\m{x}_{r+1,k}^m-\m{x}_r\|^2\\
%&+ 3 \alpha_k^2 (1+K) \left\|\m{h} (\m{x}_{r+1,k}^m, \m{Z}_{r+1,k}^m )- \m{h}  (\m{x}_{r+1,k}^m) \right\|^2\\ 
  %& \leq % 3 \exp(1) \alpha_k^2 (1+K) \sum\limits_{k=2}^{K}  L_{\m{h},\m{z}}^2 N \sum_{n=1}^N L^2_z(n)\|\m{z}_{r+1,k-1}^{m,n}-\m{z}^{n,*}\|^2
  %      \\
       &\leq 2 \exp(1)\alpha_k^2 (1+K) \sum\limits_{k=2}^{K}  \left\| \m{h}^m_{r,k-1}- \m{h} (\m{x}_{r+1,k-1}^m, \m{Z}_{r+1,k-1}^m) \right\|^2\\
       &+ 2 \exp(1) \alpha_k^2 (1+K) \sum\limits_{k=2}^{K} \left\| \m{h} (\m{x}_{r+1,k-1}^m, \m{Z}_{r+1,k-1}^m )\right\|^2 \\
         %& \leq  3 \exp(1)\alpha_k^2 (1+K) \sum\limits_{k=1}^{K-1}  L_{\m{h},\m{z}}^2 N \sum_{n=1}^N L^2_z(n)\|\m{z}_{r+1,k}^{m,n}-\m{z}^{n,*}\|^2
        %\\
       &\leq + 2 \exp(1)\alpha_k^2 (1+K) \sum\limits_{k=1}^{K-1}  \left\| \m{h}^m_{r,k}- \m{h} (\m{x}_{r+1,k}^m, \m{Z}_{r+1,k}^m) \right\|^2\\
       &+ 2 \exp(1) \alpha_k^2 (1+K) \sum\limits_{k=1}^{K-1} \left\| \m{h} (\m{x}_{r+1,k}^m, \m{Z}_{r+1,k}^m ) \right\|^2.
\end{aligned}
\end{equation}
\end{proof}

The following lemma bounds the deviation of $\m{h}^m_{r,k}$
from $\nabla f (\m{x}_{r+1,k}^m, \m{Z}_{r+1,k}^m )$.

\begin{lemma}\label{lem:drift:fedmsa2}
Suppose Assumptions~ \ref{assum:lip:y*}--\ref{assum:stmonot:g} hold. Further, assume $K \geq 1$ and $ \alpha^{m}_k\leq 1/(5M_fK), \forall m \in \mathcal{S}$. Then, for each $m \in [M]$ and $ k \in [K]$,  Algorithm~\ref{alg:fedmsa} guarantees:
\begin{equation}\label{eqn7:lem:drift:fedmsa}
\begin{aligned}
\frac{1}{K}\sum_{k=1}^K\mb{E}\left\|\m{h}^m_{r,k}-  \m{h} (\m{x}_{r+1,k}^m, \m{Z}_{r+1,k}^m )\right\|^2&\leq \frac{1}{K} \sum_{k=1}^K \mb{E} \left\|\m{h} (\m{x}_{r+1,k}^m, \m{Z}_{r+1,k}^m)\right\|^2\\
&+ 2 \exp(1) \sum_{k=1}^K \mb{E} \left\|\m{h}_{r}-\m{h} (\m{x}_{r+1}, \m{Z}_{r+1})\right\|^2,
\end{aligned}
\end{equation}
where $e=\exp(1)$.
\end{lemma}
\begin{proof}
% Here, the first inequality follows from Lemma~\ref{lem:trig}; the second inequality uses Lemma~\ref{lem:Jens}; and the third and last inequalities follow from \eqref{eqn3a:lemm:drift} and \eqref{eqn3c:lemm:drift}.
% \begin{subequations}
% \begin{equation}
% \label{eqn3c:lemm:drift}
% \begin{aligned}
% \mb{E}\left\|\m{a}^{r,k}\right\|^2 & \leq  \left(1+\frac{1}{K}\right)\mb{E}\left[\|\m{v}_{r+1,k-1}^m- \nabla f (\m{x}_{r+1, k-1}^m)\|^2\right] \\
% &+ \left(K+1\right)\mb{E}\left\|  \nabla f^m(\m{x}^{m}_{r,k}, \m{Z}_{r,k})-\nabla f^m(\m{x}^{m}_{r,k-1}, \m{Z}_{r,k-1})+ \nabla f(\m{x}^{m}_{r,k-1}, \m{Z}_{r,k-1})-\nabla f(\m{x}^{m}_{r,k}, \m{Z}_{r,k})\right\|^2 \\
% %&+\left\| \nabla f(\m{x}^{m}_{r,k-1}, \m{Z}_{r,k-1}) - \nabla f(\m{x})\right\|^2+ \left\| \nabla f(\m{x}^{m}_{r,k}, \m{Z}_{r,k}) - \nabla f(\m{x})\right\|^2\\
% & \leq  \exp (3) \mb{E} \left\|\m{v}_{r,0}^m- \nabla f (\m{x}_{r+1, 0}^m)\right\|^2 +\exp(3) \tau_1  \left(K+1\right) \mb{E}\left\| (\m{x}^{m}_{r,k}, \m{Z}_{r,k}^m)-(\m{x}^{m}_{r,k-1}, \m{Z}_{r,k-1}^m)\right\|^2 \\
% \end{aligned}
% \end{equation}
% \end{subequations}
% where the last inequality uses Assumption~\ref{assum:heter:f}.

%%%%
Let
\begin{equation}\label{eqn5:lem:drift:fedmsa}
\begin{aligned}
%\m{a}_{i,\nu}&:= \bar{\m{h}}_i(\m{x}_{i,\nu}, \m{y}^+)- \bar{\nabla} f_i(\m{x}_{i,\nu}, \m{y}^+)- \bar{\m{h}}_i(\m{x},\m{y}^+) \\
%& +\bar{\nabla} f_i(\m{x}, \m{y}^+) +\bar{\m{h}}(\m{x},\m{y}^+) -\bar{\nabla} f(\m{x}, \m{y}^+),\\
\m{a}_{r,k}^m &:= \m{h}^m_{r,k-1} -\m{h} (\m{x}_{r+1,k-1}^m, \m{Z}_{r+1,k-1}^m)\\
 & +\m{h}^m(\m{x}_{r+1,k}^m, \m{Z}_{r+1,k}^m) -\m{h}  (\m{x}_{r+1,k}^m, \m{Z}_{r+1,k}^m ) -\m{h}^m  (\m{x}_{r+1,k-1}^m,  \m{Z}_{r+1,k-1}^m) +\m{h}  (\m{x}_{r+1,k-1}^m,\m{Z}_{r+1,k-1}^m)\\
\m{b}^{m}_{r,k}&:=\m{h}^m(\m{x}^{m}_{r+1,k}, \m{Z}_{r+1,k}^m)-\m{h}^m(\m{x}^{m}_{r+1,k}, \m{Z}_{r+1,k}^m) \\
&+\m{h}^m(\m{x}^{m}_{r+1,k-1}, \m{Z}_{r+1,k-1}^m)- \m{h}^m(\m{x}^{m}_{r+1,k}, \m{Z}_{r+1,k-1}^m).\\
%\m{a}^{m}_{r,k}&:= \m{v}_{r,k-1}^m+ \nabla f^m(\m{x}^{m}_{r,k}, \m{Z}_{r,k})-\nabla f^m(\m{x}^{m}_{r,k}, \m{Z}_{r,k})+ \nabla f(\m{x}^{m}_{r,k-1}, \m{Z}_{r,k-1}) - \nabla f(\m{x}_r) + \nabla  f(\m{x}_r).
\end{aligned}
\end{equation}
%Recall the definition of  
One will notice that  %$\m{a}^{m}_{r,k} +  \m{b}^{m}_{r,k} =  \m{v}_{r,k-1}^m$. 
% Hence, from Algorithm~\ref{alg:fedmsa}, for each $m\in\mathcal{S}$, we have
% \begin{equation*}
% \begin{aligned}
%      \m{x}^{m}_{r+1,k}-\m{x}_r &=\m{x}^{m}_{r+1,k}-\m{x}_r-\alpha_k \left(\m{a}^{m}_{r,k} +  \m{b}^{m}_{r,k}\right),
%     \end{aligned}
% \end{equation*}
% which implies that 
% \begin{equation}\label{eqn3:lemm:drift:fedmsa}
% \begin{aligned}
% \mb{E}\left[\|\m{x}^{m}_{r+1,k}-\m{x}_r\|^2\right]
% &=\mb{E}\left[\|\m{x}^{m}_{r+1,k}-\m{x}_r-\alpha_k \m{a}^{m}_{r,k} \|^2\right]+\alpha_k^2\mb{E}\left[\| \m{b}^{m}_{r,k}\|^2\right]\\&-2\mb{E}\left[\mb{E}\left[\langle \m{x}^{m}_{r,k}-\m{x}_{r}-\alpha_k \m{a}^{m}_{r,k},\alpha_k \m{b}_{r,k} \rangle\mid\mathcal{F}_{r,k}^m\right]\right] \\ 
% &= \mb{E}\left[\|\m{x}^{m}_{r+1,k}-\m{x}_r-\alpha_k \m{a}_{r,k}\|^2\right]+\alpha_k^2\mb{E}\left[\|\m{b}_{r,k}^m\|^2\right].
% \end{aligned}
% \end{equation}
% Here, the last equality uses Lemma~\ref{lem:rand:zer} since  $\mb{E}[\m{b}_{r,k}^m|\mathcal{F}_{r,k}^m]=0$, {by definition}.
\begin{equation}\label{eqn6:lem:drift:fedmsa}
\begin{aligned}
\mb{E}\left\|\m{h}^m_{r,k}-\m{h}(\m{x}_{r+1,k}^m, \m{Z}_{r+1,k}^m )\right\|^2
% &=\m{h}^m_{r,k-1} - \nabla f (\m{x}_{r+1,k-1}^m, \m{Z}_{r+1,k-1}^m )\\
% &+ \m{h}^m(\m{x}^{m}_{r+1,k}, \m{Z}_{r+1,k}^m)- \nabla f^m(\m{x}^{m}_{r+1,k}, \m{Z}_{r+1,k}^m) +\m{h}^m(\m{x}^{m}_{r+1,k-1}, \m{Z}_{r+1,k-1}^m)-  \nabla f^m(\m{x}^{m}_{r+1,k-}, \m{Z}_{r+1,k-1}^m)  \\
% & + \nabla f^m(\m{x}_{r+1,k}^m, \m{Z}_{r+1,k}^m) - \nabla f  (\m{x}_{r+1,k}^m, \m{Z}_{r+1,k}^m ) -\nabla f^m  (\m{x}_{r+1,k-1}^m,  \m{Z}_{r+1,k-1}^m) + \nabla f  (\m{x}_{r+1,k-1}^m,\m{Z}_{r+1,k-1}^m)\\
&= \mb{E}\left\|\m{a}^{m}_{r,k} +  \m{b}^{m}_{r,k}\right\|^2= \mb{E}\left\|\m{a}^{m}_{r,k} \right\|^2+  \mb{E}\left\| \m{b}^{m}_{r,k}\right\|^2.
% &=\m{h}^m_{r,k-1} - \nabla f (\m{x}_{r+1,k-1}^m, \m{Z}_{r+1,k-1}^m )\\
% &+ \left\|\m{h}^m(\m{x}^{m}_{r+1,k}, \m{Z}_{r+1,k}^m)- \nabla f^m(\m{x}^{m}_{r+1,k}, \m{Z}_{r+1,k}^m) +\m{h}^m(\m{x}^{m}_{r+1,k-1}, \m{Z}_{r+1,k-1}^m)-  \nabla f^m(\m{x}^{m}_{r+1,k-}, \m{Z}_{r+1,k-1}^m)\right\|  \\
% & + \nabla f^m(\m{x}_{r+1,k}^m, \m{Z}_{r+1,k}^m) - \nabla f  (\m{x}_{r+1,k}^m, \m{Z}_{r+1,k}^m ) -\nabla f^m  (\m{x}_{r+1,k-1}^m,  \m{Z}_{r+1,k-1}^m) + \nabla f  (\m{x}_{r+1,k-1}^m,\m{Z}_{r+1,k-1}^m)
    \end{aligned}
\end{equation}
Here, the last equality uses Lemma~\ref{lem:rand:zer} since  $\mb{E}[\m{b}_{r,k}^m|\mathcal{F}_{r,k}^m]=0$, {by definition}.

%From Lemmas~\ref{lem:Jens}, \ref{lem:neum:bias}, and \ref{lem:lips},  for $\m{a}_{r,k}^m$ and $\m{b}_{r,k}^m$ defined in \eqref{eqn2:lem:drift:fedmsa},
From Assumption~\ref{assum:bias}, we have 
\begin{subequations}
\label{eqn7:lem:drift:fedmsa}
\begin{align}
\left\|\m{b}_{r,k}^m \right\|^2 &\leq  \frac{M_f^2}{b} \left\|\left(\m{x}^{m}_{r+1,k},\m{Z}_{r+1,k}^m\right)-\left(\m{x}^{m}_{r+1,k-1}, \m{Z}_{r+1,k-1}^m\right)\right\|^2.
    \end{align}
Further, 
\begin{equation}
\begin{aligned}
\left\|\m{a}_{r,k}^m \right\|^2 &\leq  \left(1+ \frac{1}{K}\right) \left\|\m{h}^m_{r,k-1} - \m{h} (\m{x}_{r+1,k-1}^m, \m{Z}_{r+1,k-1}^m)\right\|^2\\
 & + \left(1+K\right) \big\|\m{h}^m(\m{x}_{r+1,k}^m, \m{Z}_{r+1,k}^m) - \m{h}  (\m{x}_{r+1,k}^m, \m{Z}_{r+1,k}^m ) \\
 &-\m{h}^m  (\m{x}_{r+1,k-1}^m,  \m{Z}_{r+1,k-1}^m) + \m{h}  (\m{x}_{r+1,k-1}^m,\m{Z}_{r+1,k-1}^m)\big\|^2\\
 &  \leq  \left(1+ \frac{1}{K}\right) \left\|\m{h}^m_{r,k-1} - \m{h} (\m{x}_{r+1,k-1}^m, \m{Z}_{r+1,k-1}^m)\right\|^2\\
 & +2 \tau^2 \left(1+K\right)  \left\|(\m{x}^{m}_{r+1,k}, \m{Z}_{r+1,k}^m)-(\m{x}^{m}_{r+1,k-1},\m{Z}_{r+1,k-1}^m)\right\|^2.
%\m{b}^{m}_{r,k}&:=\m{h}^m(\m{x}^{m}_{r+1,k}, \m{Z}_{r+1,k}^m)- \m{h}^m(\m{x}^{m}_{r+1,k}, \m{Z}_{r+1,k}^m) 
    \end{aligned}
\end{equation}
\end{subequations}
Now, iterating equation \eqref{eqn7:lem:drift:fedmsa} and using $  \m{h}^{m}_{r+1,0}=\m{h}_{r}, ~~\forall m\in [M]$, we obtain
\begin{equation}\label{eqn6:lem:drift:fedmsa}
\begin{aligned}
&~~~~~~\mb{E}\left\|\m{h}^m_{r,k}-  \m{h} (\m{x}_{r+1,k}^m, \m{Z}_{r+1,k}^m )\right\|^2
% &=\m{h}^m_{r,k-1} - \m{h} (\m{x}_{r+1,k-1}^m, \m{Z}_{r+1,k-1}^m )\\
% &+ \m{h}^m(\m{x}^{m}_{r+1,k}, \m{Z}_{r+1,k}^m)- \m{h}^m(\m{x}^{m}_{r+1,k}, \m{Z}_{r+1,k}^m) +\m{h}^m(\m{x}^{m}_{r+1,k-1}, \m{Z}_{r+1,k-1}^m)-  \m{h}^m(\m{x}^{m}_{r+1,k-}, \m{Z}_{r+1,k-1}^m)  \\
% & + \m{h}^m(\m{x}_{r+1,k}^m, \m{Z}_{r+1,k}^m) - \m{h}  (\m{x}_{r+1,k}^m, \m{Z}_{r+1,k}^m ) -\m{h}^m  (\m{x}_{r+1,k-1}^m,  \m{Z}_{r+1,k-1}^m) + \m{h}  (\m{x}_{r+1,k-1}^m,\m{Z}_{r+1,k-1}^m)\\
\\
&= \exp(1) \mb{E} \left\|\m{h}^m_{r,0}-  \m{h} (\m{x}_{r+1,0}^m, \m{Z}_{r+1,0}^m )\right\|^2 \\
%&+    \frac{  \exp(1) M_f^2}{b} \left\|\m{x}^{m}_{r+1,k}-\m{x}^{m}_{r+1,k-1}\right\|^2\\
&+\left( \frac{  \exp(1) M_f^2}{b}+2 \tau^2 \left(1+K\right) \right) \sum_{k=1}^K \mb{E}  \left\|(\m{x}^{m}_{r+1,k}, \m{Z}_{r+1,k}^m)-(\m{x}^{m}_{r+1,k-1},\m{Z}_{r+1,k-1}^m)\right\|^2.\\
& \leq \exp(1) \mb{E} \left\|\m{h}^m_{r,0}-  \m{h} (\m{x}_{r+1,0}^m, \m{Z}_{r+1,0}^m )\right\|^2 \\
%&+    \frac{  \exp(1) M_f^2}{b} \left\|\m{x}^{m}_{r+1,k}-\m{x}^{m}_{r+1,k-1}\right\|^2\\
&+\left( \frac{  \exp(1) M_f^2}{b}+2 \tau^2 \left(1+K\right) \right) \sum_{k=1}^K \mb{E} \left\|(\m{x}^{m}_{r+1,k}, \m{Z}_{r+1,k}^m)-(\m{x}^{m}_{r+1,k-1},\m{Z}_{r+1,k-1}^m)\right\|^2\\
& \leq \exp(1) \mb{E} \left\|\m{h}^m_{r,0}-  \m{h} (\m{x}_{r+1,0}^m, \m{Z}_{r+1,0}^m )\right\|^2 \\
%&+    \frac{  \exp(1) M_f^2}{b} \left\|\m{x}^{m}_{r+1,k}-\m{x}^{m}_{r+1,k-1}\right\|^2\\
&+2\alpha_k^2\left( \frac{  \exp(1) M_f^2}{b}+2 \tau^2 \left(1+K\right) \right) \sum_{k=1}^K \mb{E} \left\|\m{h} (\m{x}_{r+1,k-1}^m, \m{Z}_{r+1,k-1}^m)\right\|^2\\
&+ 2\alpha_k^2 \left( \frac{  \exp(1) M_f^2}{b}+2 \tau^2 \left(1+K\right) \right) \sum_{k=1}^K \mb{E} \left\|\m{h}^m_{r,k-1}-\m{h} (\m{x}_{r+1,k-1}^m, \m{Z}_{r+1,k-1}^m)\right\|^2
\end{aligned}
\end{equation}
From our assumption on $\alpha_k $ and using the fact that  $  (\m{x}^{m}_{r+1,1},\m{Z}^{m}_{r+1,1})=(\m{x}^{m}_{r+1,0},\m{Z}^{m}_{r+1,0})= (\m{x}_r,\m{Z}_r), ~~\forall m\in [M]$, we obtain \eqref{eqn7:lem:drift:fedmsa}.

Combining \eqref{eqn4:lem:drift:fedmsa} and \eqref{eqn7:lem:drift:fedmsa} and using our gives the desired result.
%
%where the last inequality uses Lemma~\ref{lem:lips}.
\end{proof}
%

%\section{Multi-Level and ...}

%
\begin{lemma}\label{thm:fedin} 
Suppose Assumptions~\ref{assum:lip:y*}--\ref{assum:stmonot:g} hold. 
%Further, assume 
% \begin{equation*}
% \tau_i \geq 1,~~~~\alpha_i=\frac{\alpha}{\tau_i},~~~~\beta_i=\frac{\beta}{\tau_i},~~~~\forall i \in \mathcal{S},    
% \end{equation*}
% where  
%$\beta_{k,n} <  \min\big(1/(6\ell_{g,1}),1\big)$.
%and $\alpha$ is some positive constant. 
Then, for each $ k \in [K]$,  Algorithm~\ref{alg:fedmsa} guarantees:
\begin{align}\label{eqn:err:fedin2}
\nonumber
\left\|\m{z}_{k+1}^{1}\!\!-\m{z}^{1,*}_{k+1}\right\|^2 &\leq  a_{0}(\alpha_{k}) \left\|\m{z}_{k+1}^1-\m{z}^{1,\star}_k\right\| ^2 + a_{1}(\alpha_{k})\sum_{n=1}^N L^2_z(n) \left\|\m{z}^{n}_{k+1}\!\!-\m{z}^{n,\star}(\m{x}_{k+1})\right\|^2\\
\nonumber
&+\frac{1}{8}\alpha_k \|\m{h}(\m{x}_{k})\|^2+ \frac{1}{8}\alpha_k (1+ \alpha_k L_{\m{h},\m{z}})\left\|\m{h}_k-\m{h}(\m{x}_{k}, \m{Z}_{k})\right\|^2,    
\\
\nonumber
% \nonumber
     % &+ \frac{\lambda_{n-1}}{8} \beta_{k,n-1}\|\m{z}_k^{n-1}-\m{z}_k^{n-1,*}\|^2 + \frac{\lambda_{n-1}}{8} \beta_{k,n-1} \left\| \m{q}_k^n- \m{q}^{n-1}(\m{z}_k^{n-2},\m{z}_k^{n-1})\right\|^2 \\
\left\|\m{z}_{k+1}^{n,*}-\m{z}_{k+1}^n\right\|^2 &\leq a_2(\beta_{k,n-1})  \| \m{z}_k^{n,*}-\m{z}_{k+1}^n\|^2+ \frac{\lambda_{n-1}}{8} \beta_{k,n-1}\|\m{z}_k^{n-1}-\m{z}_k^{n-1,*}\|^2 \\
      &+ \frac{\lambda_{n-1}}{8} \beta_{k,n-1} \left\| \m{q}_k^n- \m{q}^{n-1}(\m{z}_k^{n-2},\m{z}_k^{n-1})\right\|^2, 
\end{align}
where
\begin{align*}
a_{0}(\alpha_{k})&:=1+ L_{\m{z},1} \left(1+\frac{L_{h,z}}{2}+4 L_{\m{z}} \right) \alpha_k \\
a_{1}(\alpha_{k}) &:=\left(\frac{L_{z}L_{z,h} N}{2}  + 4  L_{\m{z},1}^2  L_{\m{h},\m{z}}^2 N \alpha_k\right) \alpha_k 
\\
a_2(\beta_{k,n-1}) &:=1+ \frac{ 4 L_{\m{z},n}^2 L_{\m{q},n-1}^2}{\lambda_{n-1}}\beta_{k,n-1}.     
\end{align*}
 \end{lemma}
 \begin{proof}
Note that 
\begin{align}\label{eqn-1z1:dec:inner}
\nonumber 
\|\m{z}^{n}_{k+1}-\m{z}^{n,*}_{k+1}\|^2 =& \|\m{z}^{n}_{k+1}-\m{z}^{n,*}_{k}\|^2  + \|\m{z}^{n,*}_{k}-\m{z}^{n,*}_{k+1}\|^2\\
+&2 \left\langle \m{z}^{n,*}_{k}- \m{z}^{n}_{k+1} ,  \m{z}^{n,*}_{k+1}-\m{z}^{n,*}_{k}\rangle\right.
\end{align} 
Let   $\hat{\m{x}}_{k+1}=a\m{x}_{k} + (1-a)\m{x}_{k+1}, a \in [0,1]$. We have that 
\begin{subequations}
\begin{align}
\label{eqn-1z0:dec:inner}
\left\langle \m{z}_{k+1}^1-{\m{z}^{*}_{k}}^1, {\m{z}^{*}_{k}}^1-{\m{z}^{*}_{k+1}}^1\right\rangle &= -\left\langle \m{z}_{k+1}^1-{\m{z}^{1,*}_{k}}^1, \nabla \m{z}^{1,\star}(\hat{\m{x}}_{k+1})(\m{x}_{k+1}-\m{x}_{k})\right\rangle\\
\label{eqn-1z2:dec:inner}
&=-\left\langle\m{z}_{k+1}^{1}-\m{z}^{1,\star}(\m{x}_{k+1}),\alpha_k \nabla \m{z}^{1,\star}(\hat{\m{x}}_{k+1})^\top \m{h}(\m{x}_{k}) \right \rangle\\
\label{eqn-1z3:dec:inner}
&~~-\left\langle\m{z}_{k+1}^{1}-\m{z}^{1,\star}(\m{x}_{k+1}),\alpha_k \nabla \m{z}^{1,\star}(\hat{\m{x}}_{k+1})^\top \left(\m{h}_k-\m{h}(\m{x}_{k})\right) \right \rangle.
\end{align}
\end{subequations}
% , the second term in \eqref{eq:yk+1-yk+1*c} can be rewritten as
For the first term on the R.H.S. of the above equality, we have
\begin{equation}\label{eqn-1z2:bound:dec:inner}
    \begin{aligned}
    \eqref{eqn-1z2:dec:inner}
%&=-\left\langle\m{z}_{k+1}^{1}-\m{z}^{1,\star}(\m{x}_{k+1}),\alpha_k \nabla \m{z}^{1,\star}(\hat{\m{x}}_{k+1})^\top \m{h}(\m{x}_{k+1}, \m{Z}_{k+1}) \right \rangle\\
%  \leq &\left\|\m{z}_{k+1}\!\!-\m{z}^\star(\m{x})\right\| \alpha_k \m{h}(\m{x}^{m}_{r+1,k+1})  \left\|\right\|\\
%& \leq \alpha_k   L_{\m{z},1}\left\|\m{z}_{k+1}^1-\m{z}^{1,\star}(\m{x}_{k+1})\right\|  \left\| \m{h}_k- \m{h} (\m{x}_{k+1}, \m{Z}_{k+1}) \right\|\\
& \leq \alpha_k  L_{\m{z},1}\left\|\m{z}_{k+1}^1-\m{z}^{1,\star}(\m{x}_{k+1})\right\|  \left\| \m{h} (\m{x}_{k}, \m{Z}_{k}) \right\|\\
    &\leq  L_{\m{z},1} \big(\frac{L_{h,z}}{2}+4 L_{\m{z}} \big) \alpha_k \left\|\m{z}_{k+1}^1-\m{z}^{1,\star}(\m{x}_{k+1})\right\| ^2\\
    &+\frac{L_{z}L_{z,h} N}{2} \alpha_k\sum_{n=1}^N L^2_z(n) \left\|\m{z}^{n}_{k+1}\!\!-\m{z}^{n,\star}(\m{x}_{k+1})\right\|^2 +\! \frac{1}{8}\alpha_k\|\m{h}(\m{x}_{k})\|^2, 
  % +  \alpha_k  \left\| \m{h}_k- \m{h} (\m{x}_{k+1}, \m{Z}_{k+1}) \right\|^2,
\end{aligned}
\end{equation}
where the first inequlaity follows from 
\begin{align*}%\label{eq:vk}
    \| \m{h}(\m{x}_k,\m{Z}_k)\| 
    &\leq \|  \m{h}(\m{x}_k,\m{z}_K) -  \m{h}(\m{x}_k)+ \m{h}(\m{x}_k)\| \nonumber\\
   % &\leq \| \m{h}(\m{x}_k,\m{z}_k^{1:N}) - \m{h}(\m{x}_k)\| + \| \m{h}(\m{x}_k)\| \nonumber\\
    &\leq L_{\m{h},\m{z}} \sum_{n=1}^N L_\m{z} (n)\|\m{z}_k^n - \m{z}_k^{n,*}\| +  \|\m{h}(\m{x}_k)\|.
\end{align*}
%where the first inequality follows from Assumption \ref{assumption:vglip} and the last inequality follows from Lemma \ref{lemma:yk+1n-yn*dots}; 
Similarly, we have 
%and (b) follows from Young's inequality:
\begin{align}\label{eqn-1z3:bound:dec:inner}
    \eqref{eqn-1z3:dec:inner}
    &\leq  L_{\m{z},1} \alpha_k \left\|\m{z}_{k+1}^1-\m{z}^{1,\star}(\m{x}_{k+1})\right\| ^2+ \frac{1}{8}\alpha_k\left\|\m{h}_k-\m{h}(\m{x}_{k}, \m{Z}_{k})\right\|^2,
\end{align}
where the last inequality is obtained from the Young's inequality.% such that $ab\leq 2\gamma a^2+\frac{b^2}{8\gamma}$.
\begin{align}\label{eqn-1z0:bound:dec:inner} 
\eqref{eqn-1z0:dec:inner} 
&\leq L_{\m{z},1} \big(1+\frac{L_{h,z}}{2}+4 L_{\m{z}} \big) \alpha_k \left\|\m{z}_{k+1}^1-\m{z}^{1,\star}(\m{x}_{k+1})\right\| ^2\\
\nonumber 
    &+\frac{L_{z}L_{z,h} N}{2} \alpha_k\sum_{n=1}^N L^2_z(n) \left\|\m{z}^{n}_{k+1}\!\!-\m{z}^{n,\star}(\m{x}_{k+1})\right\|^2 +\! \frac{1}{8}\alpha_k\|\m{h}(\m{x}_{k})\|^2 +\frac{1}{8}\alpha_k\left\|\m{h}_k-\m{h}(\m{x}_{k}, \m{Z}_{k})\right\|^2.
\end{align}

The last term in \eqref{eqn-1z1:dec:inner} can be bounded as
\begin{align}\label{eqn-1z4:bound:dec:inner}
\|\m{z}_k^{1,*}-\m{z}_{k+1}^{1,*}\|^2 &\leq L_{\m{z},1}^2 \alpha_k^2 \|\m{h}(x_k,\m{Z}_{k})+\m{h}_k-\m{h}(\m{x}_{k}, \m{Z}_{k})\|^2 \nonumber\\
    &\leq  2 L_{\m{z},1}^2 \alpha_k^2 \|\m{h}(x_k,\m{Z}_{k})\|^2 + 2 L_{\m{z},1}^2 \alpha_k^2 \|\m{h}_k-\m{h}(\m{x}_{k}, \m{Z}_{k})\|^2 \nonumber\\
    &\stackrel{\eqref{eqn-1z3:bound:dec:inner}}{\leq} 4  L_{\m{z},1}^2  L_{\m{h},\m{z}}^2 N \alpha_k^2 \left(\sum_{n=1}^N L_{\m{z}}(n)^2\|\m{z}_k^n-\m{z}_k^{n,*}\|^2 \!+\! L_\m{h}^2\|\m{x}_k-\m{x}^*\|^2\right) \! \nonumber\\
    &+\! 2 L_{\m{z},1}^2  \alpha_k^2\|\m{h}_k-\m{h}(\m{x}_{k}, \m{Z}_{k})\|^2.
\end{align}
Now, from \eqref{eqn-1z2:bound:dec:inner}--\eqref{eqn-1z4:bound:dec:inner}, we get \eqref{eqn:err:fedin2}.
% \begin{align}
% \nonumber
% \left\|\m{z}_{k+1}^{1}\!\!-\m{z}^{1,*}_{k+1}\right\|^2 &\leq  L_{\m{z},1} \big(1+\frac{L_{h,z}}{2}+4 L_{\m{z}} \big) \alpha_k \left\|\m{z}_{k+1}^1-\m{z}^{1,\star}_k\right\| ^2\\
% \nonumber
% &+\left(\frac{L_{z}L_{z,h} N}{2} \alpha_k  + 4  L_{\m{z},1}^2  L_{\m{h},\m{z}}^2 N \alpha_k^2 \right) \sum_{n=1}^N L^2_z(n) \left\|\m{z}^{n}_{k+1}\!\!-\m{z}^{n,\star}(\m{x}_{k+1})\right\|^2\\
% &+\frac{1}{8}\alpha_k \|\m{h}(\m{x}_{k})\|^2 + \frac{1}{8}\alpha_k (1+ \alpha_k L_{\m{h},\m{z}})\left\|\m{h}_k-\m{h}(\m{x}_{k}, \m{Z}_{k})\right\|^2    
% \end{align}
%
By the mean-value theorem, for some $\hat{\m{z}}_{k+1}^{n-1}=a \m{z}_k^{n-1} + (1-a) \m{z}_{k+1}^{n-1}, a \in [0,1]$, the second term can be rewritten as
\begin{subequations}
\begin{align}
\label{eqn:inner:drift:0}
    \langle \m{z}_k^{n,*}-\m{z}_{k+1}^n,\m{z}_{k+1}^{n,*}-\m{z}_k^{n,*} \rangle 
    &= \langle \m{z}_k^{n,*}-\m{z}_{k+1}^n,\nabla \m{z}^{n,*}(\hat{\m{z}}_{k+1}^{n-1})^\top (\m{z}_{k+1}^{n-1}-\m{z}_k^{n-1}) \rangle \\
    &= \left\langle \m{z}_k^{n,*}-\m{z}_{k+1}^n,\beta_{k,n-1}\nabla \m{z}^{n,*}(\hat{\m{z}}_{k+1}^{n-1})^\top \m{q}^{n-1}(\m{z}_k^{n-2},\m{z}_k^{n-1}) \right \rangle \label{eqn:inner:drift:1}\\
    &+ \left\langle \m{z}_k^{n,*}-\m{z}_{k+1}^n,\beta_{k,n-1}\nabla \m{z}^{n,*}(\hat{\m{z}}_{k+1}^{n-1})^\top \left( \m{q}_k^{n-1}- \m{q}^{n-1}(\m{z}_k^{n-2},\m{z}_k^{n-1})\right)\right\rangle.
    \label{eqn:inner:drift:2}
\end{align}
\end{subequations}
Now, we have %e first term in the right-hand side (RHS) of \eqref{eq:drift n>=2} can be bounded as
\begin{align}\label{eq:driftI1 n>=2}
     \eqref{eqn:inner:drift:1}
    %\langle \m{z}_k^{n,*}-\m{z}_{k+1}^n,\beta_{k,n-1}\nabla \m{z}^{n,*}(\hat{\m{z}}_{k+1}^{n-1})^\top \m{q}^{n-1}(\m{z}_k^{n-2},\m{z}_k^{n-1}) \rangle \nonumber\\
    &\leq L_{\m{z},n}\beta_{k,n-1}\| \m{z}_k^{n,*}-\m{z}_{k+1}^n\| \| \m{q}^{n-1}(\m{z}_k^{n-2},\m{z}_k^{n-1})\| \nonumber\\
    &\leq L_{\m{z},n}L_{\m{q},n-1}\beta_{k,n-1}\| \m{z}_k^{n,*}-\m{z}_{k+1}^n\|\|\m{z}_k^{n-1}-\m{z}_k^{n-1,*}\| \nonumber\\
    &\leq \frac{2 L_{\m{z},n}^2 L_{\m{q},n-1}^2}{\lambda_{n-1}}\beta_{k,n-1}\| \m{z}_k^{n,*}-\m{z}_{k+1}^n\|^2 + \frac{\lambda_{n-1}}{8} \beta_{k,n-1}\|\m{z}_k^{n-1}-\m{z}_k^{n-1,*}\|^2
\end{align}
where the second inequality follows from
\begin{align}\label{eq:hn-1}
    \| \m{q}^{n-1}(\m{z}_k^{n-2},\m{z}_k^{n-1})\| 
    &= \|\m{q}^{n-1}(\m{z}_k^{n-2},\m{z}_k^{n-1})- \m{q}^{n-1}(\m{z}_k^{n-2},\m{z}_k^{n-1,*})\| \nonumber\\
    &\leq L_{\m{q},n-1} \|\m{z}_k^{n-1}-\m{z}_k^{n-1,*}\|.
\end{align}
Similarly, 
\begin{align}%\label{eq:driftI1 n>=2}
     \eqref{eqn:inner:drift:2}
    &\leq L_{\m{z},n}\beta_{k,n-1}\| \m{z}_k^{n,*}-\m{z}_{k+1}^n\|   \left\| \m{q}_k^n- \m{q}^{n-1}(\m{z}_k^{n-2},\m{z}_k^{n-1})\right\|^2 \nonumber\\
  %  &\leq L_{\m{z},n}L_{\m{q},n-1}\beta_{k,n-1}\| \m{z}_k^{n,*}-\m{z}_{k+1}^n\|\|\m{z}_k^{n-1}-\m{z}_k^{n-1,*}\| \nonumber\\
    &\leq \frac{2 L_{\m{z},n}^2 L_{\m{q},n-1}^2}{\lambda_{n-1}}\beta_{k,n-1}\| \m{z}_k^{n,*}-\m{z}_{k+1}^n\|^2 + \frac{\lambda_{n-1}}{8} \beta_{k,n-1} \left\| \m{q}_k^{n-1}- \m{q}^{n-1}(\m{z}_k^{n-2},\m{z}_k^{n-1})\right\|^2.
\end{align}
Hence, we get 
\begin{align}
\left\|\m{z}_{k+1}^{n,*}-\m{z}_{k+1}^n\right\|^2 &\leq \left(1+ \frac{ 4 L_{\m{z},n}^2 L_{\m{q},n-1}^2}{\lambda_{n-1}}\beta_{k,n-1}\right)\| \m{z}_k^{n,*}-\m{z}_{k+1}^n\|^2 \\
 \nonumber
      &+ \frac{\lambda_{n-1}}{8} \beta_{k,n-1}\|\m{z}_k^{n-1}-\m{z}_k^{n-1,*}\|^2 + \frac{\lambda_{n-1}}{8} \beta_{k,n-1} \left\| \m{q}_k^n- \m{q}^{n-1}(\m{z}_k^{n-2},\m{z}_k^{n-1})\right\|^2. 
\end{align}
\end{proof}

\begin{remark}
Lemma~\ref{thm4:lemma2} shows that the bound on the client-drift scales linearly with $\tau_i$ and the inner error $\|\m{y}^+-\m{y}^\star(\m{x})\|^2$ in general nested FL. We aim to control such a drift by selecting $\alpha_i=\mc{O}(1/\tau_i)$ for all $ i \in \mc{S}$ and using the inner error bound provided in Lemma~\ref{thm:fedin}. 
\end{remark}

Next, we provide the proof of our main result which can be adapted to general nested problems (bilevel, min-max, compositional).
