# Supplementary material for: Federated Multi-Sequence Stochastic Approximation with Local Hypergradient Estimation
Source: arXiv:2306.01648 source file (2023-06-02)
Supplement: Supplementary file 3 [file supp_experiment.tex]

\section{Additional Experimental Results}\label{sec:app:experim}
In this section, we first provide the detailed parameters in Section~\ref{sec:numerics} and then discuss more experiments. In Section~\ref{sec:numerics}, our federated algorithm implementation is based on \cite{shaoxiong}, both hyper-representation and loss function tuning use batch size $64$ and Neumann series parameter $N=5$. We conduct 5 SGD/SVRG epoch of local updates in \fedinn and $\tau=1$ in \fedout. In \fednest, we use $T=1$, have 100 clients in total, and 10 clients are selected in each \fednest epoch.  
\begin{figure}[h]
    \begin{subfigure}{0.5\textwidth}
    \centering
        \begin{tikzpicture}
        \node at (0,0) [scale=0.5]{\includegraphics[]{figs/supp/supp_noniid_epoch.pdf}};
        \node at (-3.8,0) [rotate=90] {Test accuracy};
        \node at (0,-3.2) [] {Epoch};
        \end{tikzpicture}\caption{The test accuracy w.r.t to the algorithm epochs.}\label{fig:app:noniid_comm_a}
    \end{subfigure}
    \begin{subfigure}{0.5\textwidth}
    \centering
        \begin{tikzpicture}
        \node at (0,0) [scale=0.5]{\includegraphics[]{figs/supp/supp_noniid_round.pdf}};
        \node at (0,-3.2) [] {\# of communications};
        \end{tikzpicture}\caption{The test accuracy w.r.t to the number of communications.}\label{fig:app:noniid_comm_b}
    \end{subfigure}\caption{Hyper representation experiment comparing \lfedblo, $\lfedblo_{\textnormal{\tiny{SVRG}}}$ and \textsc{LFedNest-NonAlt} on \textbf{non-i.i.d} dataset. The number in parentheses corresponds to communication rounds shown in Table~\ref{tabl:supp:methods}.}
    \label{fig:app:noniid_comm}
\end{figure}
\begin{figure}[h]
    \begin{subfigure}{0.50\textwidth}
    \centering
        \begin{tikzpicture}
        \node at (0,0) {\includegraphics[scale=0.5]{figs/lrs/noniid_0.0075_round.pdf}};
        \node at (-4.3,0) [rotate=90, scale=1.2] {Test accuracy};
        \node at (0,-3.3) [scale=1.2] {\# of communications};
        \end{tikzpicture}\caption{$\alpha=0.0075$}
    \end{subfigure}
    \begin{subfigure}{0.4\textwidth}
    \centering
        \begin{tikzpicture}
        \node at (0,0) [scale=0.5]{\includegraphics[]{figs/lrs/noniid_0.005_round.pdf}};
        \node at (0,-3.3) [scale=1.2] {\# of communications};
        \end{tikzpicture}\caption{$\alpha=0.005$}
    \end{subfigure}
    
    \begin{subfigure}{0.5\textwidth}
    \centering
        \begin{tikzpicture}
        \node at (0,0) [scale=0.5]{\includegraphics[]{figs/lrs/noniid_0.0025_round.pdf}};
        \node at (-4.3,0) [rotate=90, scale=1.2] {Test accuracy};
        \node at (0,-3.3) [scale=1.2] {\# of communications};
        \end{tikzpicture}\caption{$\alpha=0.0025$}
    \end{subfigure}
    \begin{subfigure}{0.45\textwidth}
    \centering
        \begin{tikzpicture}
        \node at (0,0) [scale=0.5]{\includegraphics[]{figs/lrs/noniid_0.001_round.pdf}};
        \node at (0,-3.3) [scale=1.2] {\# of communications};
        \end{tikzpicture}\caption{$\alpha=0.001$}
    \end{subfigure}\caption{Learning rate analysis on \textbf{non-i.i.d.} data with respect to \textbf{\# of communications}.}\label{fig:app:lr_noniid}
\end{figure}
\subsection{The effect of the alternating between inner and outer global variables}\label{sec:joinvsalt} 
In our addition experiments, we investigate the effect of the alternating between inner and outer {global} variables $\m{x}$ and $\m{y}$. We use \textsc{LFedNest-NonAlt} to denote the training where each client updates their local $\y_{i}$ and then update local $\x_{i}$ w.r.t. local $\y_{i}$ for all $i \in\mc{S}$. Hence, the nested optimization is performed locally (within the clients) and the joint variable $[\x_{i},\y_{i}]$ is communicated with the server. One can notice that only one communication is conducted when server update global $\x$ and $\y$ by aggregating all $\x_{i}$ and $\y_{i}$. 

As illustrated in Figure~\ref{fig:app:noniid_comm}, the test accuracy of \textsc{LFedNest-NonAlt} remains around $80\%$, but both standard $\lfedblo$ and $\lfedblo_{\textnormal{\tiny{SVRG}}}$  achieves better performance. Here, the number of inner iterations is set to $T=1$. The performance boost reveals the necessity of both averaging and SVRG in \fedinn, where the extra communication makes clients more consistent.% in non-i.i.d. setup.

\subsection{The effect of the learning rate and the global inverse Hessian} 
Figure~\ref{fig:app:lr_noniid} shows that on non-i.i.d. dataset, both SVRG and \fedout have the effect of stabilizing the training. Here, we set  $T=1$ and $N=5$. As we observe in (a)-(d), where the learning rate decreases, the algorithms with more communications are easier to achieve convergence. We note that \lfedblo successfully converges in (d) with a very small learning rate. In contrast, in (a), \fednest (using the global inverse Hessian) achieves better test accuracy in the same communication round with a larger learning rate.
