# Supplementary material for: Federated Multi-Sequence Stochastic Approximation with Local Hypergradient Estimation
Source: arXiv:2306.01648 source file (2023-06-02)
Supplement: Supplementary file 4 [file supp_extension.tex]

\section{\fedout~2}

Estimator~\eqref{eq.inverse-estimatorfed} incorporates only one term of the Neumann series. Hence, one needs a quadratically growing number of samples which worsens the sample complexity \citep[
Corollary 3.1]{ghadimi2018approximation}. To overcome these issues, we consider an estimator which is based on the observation that the Neumann series has the following succinct recursive definition. 
\som{These should also be normalized with $\ell_{g,1}$ right?}
Let $\m{H}:=\nabla^2_y g(\m{x},\m{y})$, $\m{H}_i:=\nabla^2_y g_i(\m{x},\m{y})$, and define $\m{H}_{iN}^{-1} := \sum_{n=0}^{N} (\m{I} -\m{H}_i)^n$, i.e., the first $N+1$ terms of the Neumann series. Then, $\m{H}_{iN}^{-1} = \m{I}+(\m{I}-\m{H}_i)\m{H}^{-1}_{i,N-1}$. Using this formulation, one can obtain an unbiased estimator of $\m{H}_{i}^{-1}$ by deriving an unbiased estimator $\tilde{\m{H}}_{iN'}^{-1}$ for $\m{H}_{iN}^{-1}$ as follows:
\begin{eqnarray}\label{eq:neum:recu}
\tilde{\m{H}}_{i0}^{-1} =\m{I}, ~~~~ \tilde{\m{H}}_{in}^{-1} = \m{I} + (\m{I}-\m{X}_{in}) \tilde{\m{H}}_{i,n-1}^{-1}, 
\end{eqnarray}
 Here $\m{X}_{in} :=\nabla_{y}^2g_i(\m{x},\m{y};\zeta_{(n)})$, $N'$ is drawn from $\{1, 2, \ldots, N\}$ uniformly at random,  and $\{\zeta_{(1)}, \ldots,\zeta_{(N')}\}$ are i.i.d. samples. 
 
 It can be readily seen that $\mb{E}[\tilde{\m{H}}_{iN'}^{-1}] =\m{H}_{iN}^{-1} $ and therefore $\mb{E}[\tilde{\m{H}}_{iN'}^{-1}]\rightarrow \m{H}_{i}^{-1}$ as $N \rightarrow \infty$ giving us an unbiased estimator in the limit (see, Lemma~\ref{lem:neum:bias}). The procedure \eqref{eq:neum:recu} allows us to estimate $\m{p} \approx \tilde{\nabla}f(\m{x},\m{y})$ recursively as follows: For all $i\in \mc{S}$, let $\m{p}_{i,0} =1/m\sum_{i\in\mathcal{S}}\nabla_y g_i(\m{x}, \m{y})$ and define
\som{Why are you averaging Hessian inverses in (8b)? My concern is this is writing global inverse as sum of local inverses}
\begin{subequations}\label{eqn:hypergrad:est}
\begin{eqnarray}
\m{p}_{i,n} &=& \m{p}_{i,0}+ (\m{I}-\m{X}_{i,n})\m{p}_{i,n-1}~~~ \textnormal{for all}~~~ n=1, \ldots, N',\\
\m{p}_{N'}&=&1/m\sum_{i\in\mathcal{S}}\m{p}_{i,N'},\\
\m{p} &=& 1/m\sum_{i\in\mathcal{S}}\nabla_{\m{x}} f_i(\m{x}, \m{y})- \nabla^2_{\m{xy}}g_i(\m{x},\m{y})\m{p}_{N'}.
\end{eqnarray}
\end{subequations}
