# Supplementary material for: Federated Multi-Sequence Stochastic Approximation with Local Hypergradient Estimation
Source: arXiv:2306.01648 source file (2023-06-02)
Supplement: Supplementary file 6 [file supp_fedIMVP.tex]

\newcommand{\beq}{\begin{equation}}
\newcommand{\ba}{\begin{align}}
\newcommand{\ea}{\end{align}}

\newcommand{\eeq}{\end{equation}}

\newcommand{\B}{{{\mtx{B}}}}

\newcommand{\Qb}{{\mtx{Q}}}
\newcommand{\Qh}{{\mtx{\hat{Q}}}}
\newcommand{\Qt}{{\mtx{\tilde{Q}}}}

\newcommand{\Hb}{{\mtx{H}}}
\newcommand{\Hbi}{{\mtx{H}\mtx{I}}}

%\newcommand{\M}{{\mtx{M}}}

%\newcommand{\order}[1]{{\cal{O}}(#1)}

%\newcommand{\tn}[1]{\|{#1}\|_{\ell_2}}
%_{#2}}

%_{\Ttc}
%

%\newcommand{\supp}[1]{\text{supp}(#1)}

\newcommand{\Ac}{\mathcal{A}}

\newcommand{\Hh}{{\mtx{\hat{H}}}}

%%YP's macros

%\newcommand{\m}[1]{{\bf{#1}}}

%\newcommand{\lip}{L}

%\newcommand{\x}{\vct{x}}

%\newcommand{\y}{\vct{y}}

%--------------

% EJC's macros

\definecolor{emmanuel}{RGB}{255,127,0}

\newcommand{\Cov}[1]{\textrm{Cov}[#1]}
%\newcommand{\sgn}[1]{\textrm{sgn}(#1)}

%\newcommand{\E}{\operatorname{\mathbb{E}}}
%\newcommand{\var}{\operatorname{\mathbf{var}}}

%\newcommand{\todo}[1]{{\bf TODO: #1}}

% MS's macros

%\title{Improved Inverse Hessian Estimation via Neumann}

% \begin{document}
% \maketitle

    \begin{algorithm}[t]
  \caption{$\m{p}_{N'}=~\pmb{\fedhess}~(\m{x}, \m{y}^+,N)$: Federated approximation of inverse-Hessian-gradient product}
\begin{algorithmic}[1]
%\For{$t=T-1,...,0$}
\State Select $ N'\in \{0, \dots, N-1\}$ UAR.
\State Select $\mc{S}_0 \in \mc{S}$ UAR.
%\State If $N'=0$ 
  \For{$i \in \mc{S}_0$ \textbf{in parallel}} 
 \State $\m{p}_{i,0} =\nabla_\m{y} f_i(\m{x}, \m{y}^+; \xi_{i,0})$
 \EndFor
 \State $ \m{p}_0 = \frac{N}{\ell_{g,1}}  |\mc{S}_0|^{-1}\sum_{i\in\mathcal{S}_0} \m{p}_{i,0}$  %\hspace{.5cm}\texttt{\#communication}  
\If{$N'=0$}
\State  Return $\m{p}_{N'}$
\EndIf
%  \State{{\color{blue} Option~I (Local Inverse):} 
%  \State Select $\mc{S}_{ N'} \in \mc{S}$ UAR.}
%   		\For {$i \in \mc{S}_{N'}$ \textbf{in parallel}} 
% 		 \State $\m{p}_{i,N'} = \prod\limits_{n=1}^{N'} \big(\m{I}-\frac{1}{\ell_{g,1}}\nabla^2_y g_i(\m{x}, \m{y}^+;{\zeta}_{i,n})\big)\m{p}_{0}$% \Comment{$\m{X}_{i,j} := \nabla^2_y g_i(\m{x}, \m{y}^+;\xi_j)$}
% 	   \EndFor
% 	   \State $\m{p}_{N'}= |\mc{S}_{N'}|^{-1}\sum_{i\in\mc{S}_{N'}} \m{p}_{i,N'}$ 
%\State{{\color{blue} Option~II (Global Inverse):}}
\State Select $\mc{S}_1, \ldots, \mc{S}_{ N'} \in \mc{S}$ UAR.
\For{$n=1,\ldots, N'$}
 	   % \State Choose $N' \in \{0,\ldots,N-1\}$ randomly and 
	%	\For {$i \in \mc{S}$ \textbf{in parallel}} 
		\For {$i \in \mc{S}_n$ \textbf{in parallel}} 
		 \State $\m{p}_{i,n} = \left(\m{I}-\frac{1}{\ell_{g,1}}\nabla^2_\m{y} g_i(\m{x}, \m{y}^+;{\zeta}_{i,n})\right)\m{p}_{n-1}$% \Comment{$\m{X}_{i,j} := \nabla^2_y g_i(\m{x}, \m{y}^+;\xi_j)$}
	   \EndFor
	   \State $\m{p}_{n}=|\mc{S}_n|^{-1}\sum_{i\in\mc{S}_n} \m{p}_{i,n}$ %\hspace{.5cm}\texttt{\#communication}  
	   %\Else 
 	   %\State $\m{p}_{i}^{k,t}=\m{p}^{k,t+1}-\beta_i \nabla_\m{y}^+^2  g_i (\m{x},\m{y}^+)\m{p}^{k,t+1}$~~ 
	   %\EndFor
	%	\State $\m{p}^{k,t}= 1/m\sum_{i\in\mathcal{S}} \m{p}_{i}^t$
	%	\State { $\m{p}^k=\sum_{t=0}^{T-1}\m{p}^{k,t}$}
		\EndFor
%\State  Set $\m{p}_{N}= \frac{N}{\ell_{g,1}} \m{p}_{N'}$. Return $\m{p}_N$		
\end{algorithmic}\label{fedihgp_algo}
\end{algorithm}

%\ct{Should $\mathbf{p}_0$ change to use local iterates $x_{i,\ell}$ for OPTION 1? At least, to agree with $h_{i}(x_{i,\ell},y)$.}
\begin{theorem} Recall $B$ is the batch size, set $\kappa=L/\mu$ and $\Xi=\frac{\sigma^2+\sigmab^2}{BL^2}$. Then, for any (fixed) input $\vb$, the outcome of stochastic Neumann approximation with $N$ rounds obeys
\begin{align}
\tn{\vb}^{-1}\tn{\E[\s_{N-1}]-[\nabla^2 f(\x)]^{-1}\vb}&\leq \frac{1}{\mu} \left(1-\frac{1}{\kappa}\right)^{N},\label{conc1} \\
\tn{\vb}^{-2}\E\left[\tn{\s_{N-1}-\E[\s_{N-1}]}^2\right]&\leq\begin{cases} N^2((1+\Xi)^N-1)/L^2\\8\kappa^3\Xi/L^2\quad\text{if}\quad \Xi\kappa\leq 1/4\end{cases}.\label{conc2}
%\E\left[\tn{\s_{N-1}-[\nabla^2 f(\x)]^{-1}\vb}^2\right]^{1/2}&\leq \frac{1}{\mu} \left(1-\frac{1}{\kappa}\right)^{N}+\frac{N^{3/2}\sigma}{L^2\sqrt{B}}. \nonumber%\label{conc3}
\end{align}
%The final line follows from combining former two.
\end{theorem}

\begin{lemma}[Est 2 $\geq$ Est 1] Suppose $\Ac=(\A_i)_{i=1}^N$ are random matrices. Let $\B_1$ be a random matrix drawn from $\Ac$ uniformly at random (independent of $\Ac$). Also let $\B_2=\sum_{i=1}^N \A_i/N$. For fixed $\vb$, covariances obey
% of Estimator 1 
\[
\Cov{\B_1\vb}\succeq \Cov{\B_2\vb}.
\]
\end{lemma}
\begin{proof} Let $\mu$ be the measure that draws $\A'$ from $\Ac$. Through law of total (co)variance, we write\\
$
    \Cov{\B_1\vb}=\E_{\mu}[\Cov{\B_1\vb\big | \Ac}]+\Cov{\E_{\mu}[\B_1\vb\big | \Ac]}\succeq\Cov{\E_{\mu}[\B_1\vb\big | \Ac]}=\Cov{\B_2\vb}.
$
\end{proof}
\begin{assumption} $\nabla^2 f_i(\x;\zeta)$ is unbiased estimate of $\nabla^2 f_i(\x)$ with $\E\|\nabla^2 f_i(\x;\zeta)-\nabla^2 f_i(\x)\|^2\leq \sigma^2$. $f_i$ is $\mu$ strongly convex and $L$ Lipschitz for all $i\in [m]$. Let $\kappa\sim \unif{[m]}$. The inter-client variance obeys $\E\|\nabla^2 f_\kappa(\x)-\nabla^2 f(\x)\|^2\leq \sigmab^2$.
\end{assumption}
\begin{theorem} Recall $B$ is the batch size, set $\kappa=L/\mu$ and $\Xi=\frac{\sigma^2+\sigmab^2}{BL^2}$. Then, for any (fixed) input $\vb$, the outcome of Algorithm \ref{fedihgp_algo} obeys
\begin{align}
\tn{\vb}^{-1}\tn{\E[\s_{N-1}]-[\nabla^2 f(\x)]^{-1}\vb}&\leq \frac{1}{\mu} \left(1-\frac{1}{\kappa}\right)^{N},\label{conc1} \\
\tn{\vb}^{-2}\E\left[\tn{\s_{N-1}-\E[\s_{N-1}]}^2\right]&\leq\begin{cases} N^2((1+\Xi)^N-1)/L^2\\8\kappa^3\Xi/L^2\quad\text{if}\quad \Xi\kappa\leq 1/4\end{cases}.\label{conc2}
%\E\left[\tn{\s_{N-1}-[\nabla^2 f(\x)]^{-1}\vb}^2\right]^{1/2}&\leq \frac{1}{\mu} \left(1-\frac{1}{\kappa}\right)^{N}+\frac{N^{3/2}\sigma}{L^2\sqrt{B}}. \nonumber%\label{conc3}
\end{align}
%The final line follows from combining former two.
\end{theorem}
\textbf{Remark 1.} We provide two variance bounds. The first one always holds but grows with $N$. Observe that $N^2((1+\Xi)^N-1)=\order{N^3\Xi}$ as long as $\Xi N=o(1)$. On the other hand, the second bound only holds for small $\sigma^2/B$ i.e.~either batch size is large or Hessian sampling noise is small. The advantage of this bound is that, $N^3$ is replaced with $\kappa^3$ for all choices of $N$.

\noindent\textbf{Remark 2.} Above \emph{fixed} means $\vb$ is independent of the stochasticity of the \fedhess algorithm. Result can be extended to \emph{all} $\vb$ (i.e.~adversarial) under mild assumptions. This can be accomplished through Theorem I of Tropp's \url{https://arxiv.org/pdf/1506.04711}.

\begin{proof} Let us set $\Hb_i=\nabla^2 f_i(\x)$ and $\Hb=\nabla^2 f(\x)$. First, observe that
\[
\Hb^{-1}=\frac{1}{L}(\Iden-(\Iden-\frac{1}{L}\Hb))^{-1}=\frac{1}{L}\sum_{n=0}^\infty (\Iden-\frac{1}{L}\Hb)^n.
\]
Also define the truncation $\Hbi[N]=\frac{1}{L}\sum_{n=0}^{N} (\Iden-\frac{1}{L}\Hb)^n$. Observe that
\[
\|\Hb^{-1}-\Hbi[N]\|\leq \frac{1}{L}\sum_{n=N+1}^{\infty} \|(\Iden-\frac{1}{L}\Hb)^n\|\leq \frac{1}{\mu}\left(1-\frac{1}{\kappa}\right)^{N+1}.
\]
To proceed, let $\Hh_n=\frac{1}{|\Sc_n|}\sum_{i\in \Sc_n}\nabla^2 f_i(\m{x};{\zeta}_{i,n})$ and observe that $\E[\Hh_n]=\E[\frac{1}{|\Sc_n|}\sum_{i\in \Sc_n}\nabla^2 f_i(\m{x})]=\Hb$. 
Also set $\Qh_n=\prod_{i=1}^n (\Iden-\frac{1}{L}\Hh_i)$, $\Qb_n= (\Iden-\frac{1}{L}\Hb)^n$, $\Qt_n=\Qh_n-\Qb_n$. Note that, we are simply studying the vector $\s_N$
\[
\s_N=\frac{1}{L}\sum_{i=0}^N\prod_{i=1}^n(\Iden-\frac{1}{L}\Hh_i)\vb=\frac{1}{L}\sum_{n=0}^N\Qh_n\vb,
\]
Since $\E[\Qh_n]=\Qb_n$, we conclude with \eqref{conc1} via
\begin{align}
&\E[\s_N]=\frac{1}{L}\sum_{i=0}^n\Qb_n\vb=\Hbi[N]\vb\implies\\
&\tn{\Hb^{-1}\vb-\E[\s_N]}=\|\frac{1}{L}\sum_{n=N+1}^{\infty} (\Iden-\frac{1}{L}\Hb)^n\|\tn{\vb}\leq \frac{\tn{\vb}}{\mu}\left(1-\frac{1}{\kappa}\right)^{N+1}
\end{align}

The critical claim is \eqref{conc2} whose left hand side is equal to
\[
%\E[\vb^\top \frac{1}{L}\sum_{n=0}^N\Qh_n-\frac{1}{L}\sum_{n=0}^N\Qb_n\vb
\s_n-\E[\s_n]=\frac{1}{L}\sum_{n=0}^N\Qt_n\vb.
\]
Noticing $\Qt_0=0$, we may expand the variance as
\begin{align}
\E[\tn{\s_n-\E[\s_n]}^2]=\E[\tn{\frac{1}{L}\sum_{n=1}^N\Qt_n\vb}^2]=\frac{1}{L^2}\vb^\top \sum_{N\geq i,j\geq 1}\E[\Qt_i^\top \Qt_j]\vb.
\end{align}
\red{\textbf{Remark.} For Neumann Estimator 1 (random rather than average), instead of above, we would have % will be replaced with
\[
\E[\tn{\s^{\text{Est1}}_n-\E[\s_n]}^2]=\frac{N}{L^2}\vb^\top \sum_{N\geq i\geq 0}\E[\Qt_i^\top \Qt_i]\vb.
\]}
Observe that $\tn{(\A-\B)\vb}^2=\vb^\top (\A^\top \A+\B^\top\B-\A^\top\B-\B^\top\A)\vb\geq 0$. Thus, we can upper bound the cross terms via diagonal to conclude
\begin{align}
L^2\tn{\s_n-\E[\s_n]}^2\leq N\sum_{n=1}^N\vb^\top \E[\Qt_n^\top \Qt_n]\vb=N\sum_{n=1}^N\E[\tn{ \Qt_n\vb}^2].\label{naive bound}
\end{align}
\red{This also implies Neumann Estimator 1 is worse than Estimator 2 and the quality gap depends on the tightness of the arithmetic-geometric mean inequality above.}

To proceed, we have the following lemma that controls $\E[\tn{ \Qt_n\vb}^2]$.
\begin{lemma} Set $\Xi=\frac{\sigma^2}{L^2B}$. For all $0\leq n\leq \infty$, we have that
\[
\frac{\E[\tn{\Qt_{n}\vb}^2]}{\tn{\vb}^2}\leq (1+\Xi)^n-1.
\]
Additionally, if $\Xi\kappa \leq 1/4$, we have that 
\[
\frac{\E[\tn{\Qt_{n}\vb}^2]}{\tn{\vb}^2}\leq n(1-\frac{1}{\kappa})^{2n-2}\Xi.
\]
\end{lemma}
\begin{proof}
Set $(\gamma_n)_{n\geq 0}$ such that $\gamma_0=0$ and for $n\geq 1$
\[
\gamma_n=\frac{}{}\frac{\E[\tn{\Qt_{n}\vb}^2]}{\tn{\vb}^2}.
\]
We may write $\E[\tn{ \Qt_n\vb}^2]$ recursively in terms of $\E[\tn{ \Qt_{n-1}\vb}^2]$ as follows
\begin{align}
\E[\tn{\Qt_{n}\vb}^2]&=\E[\tn{\left[(\Iden-\frac{1}{L}\Hh_n)\Qh_{n-1}-(\Iden-\frac{1}{L}\Hb)\Qb_{n-1}\right]\vb}^2]\\
&=\E[\tn{\left[(\Iden-\frac{1}{L}\Hb)\Qt_{n-1}+\frac{1}{L}(\Hb-\Hh_n)\Qb_{n-1}+\frac{1}{L}(\Hb-\Hh_n)\Qt_{n-1}\right]\vb}^2]\\
&=\E\left[\vb^\top(\sum_{1\leq i,j\leq 3}\A_i^\top \A_j) \vb\right],
\end{align}
where $\A_1=(\Iden-\frac{1}{L}\Hb)\Qt_{n-1}$, $\A_2=\frac{1}{L}(\Hb-\Hh_n)\Qb_{n-1}$, $\A_3=\frac{1}{L}(\Hb-\Hh_n)\Qt_{n-1}$. Note that, the cross products $\E[\A_i^\top\A_j]=0$ for $i\neq j$ due to independence of sampling at $n$ from earlier samples and centered variables. To proceed, recalling $\frac{\E[\tn{\Qt_{n}\vb}^2]}{\tn{\vb}^2}= \gamma_{n}$ and setting $\sigmat=\sqrt{\sigma^2+\sigmab^2}$, we control each $\E\tn{\A_i\vb}^2$ term as follows% note that
\begin{align*}
&\E\tn{\A_1\vb}^2= \E[\tn{(\Iden-\frac{1}{L}\Hb)\Qt_{n-1}\vb}^2]\leq(1-\frac{1}{\kappa})^2\E[\tn{\Qt_{n-1}\vb}^2]\leq (1-\frac{1}{\kappa})^2 \gamma_{n-1}\tn{\vb}^2,\\
&\E\tn{\A_2\vb}^2\leq \E[\tn{\frac{1}{L}(\Hb-\Hh_n)\Qb_{n-1}\vb}^2]\leq\frac{\sigmat^2\tn{\Qb_{n-1}\vb}^2}{L^2|\Sc_n|}\leq(1-\frac{1}{\kappa})^{2n-2}\frac{\sigmat^2\tn{\vb}^2}{L^2|\Sc_n|},\\
&\E\tn{\A_1\vb}^2= \frac{1}{L^2}\E[\tn{(\Hb-\Hh_n)\Qt_{n-1}\vb}^2]\leq \frac{\sigmat^2\E[\tn{\Qt_{n-1}\vb}^2]}{L^2|\Sc_n|}\leq \frac{\sigmat^2\gamma_{n-1}\tn{\vb}^2}{L^2|\Sc_n|}.
\end{align*}
Set $\Xi_n=\frac{\sigmat^2}{L^2|\Sc_n|}$. Thus, starting with $\gamma_0=0$, we find the recursion
\[
\gamma_n\leq ((1-\frac{1}{\kappa})^2+\Xi_n)\gamma_{n-1}+(1-\frac{1}{\kappa})^{2n-2}\Xi_n.
\]
In our case, we have $B=|\Sc_n|$ and $\Xi=\Xi_n=\frac{\sigmat^2}{L^2B}=\frac{\sigma^2+\sigmab^2}{L^2B}$. Unrolling $\gamma_n$, we upper bound it via
\begin{align}
\gamma_n\leq \sum_{i=0}^{n-1}((1-\frac{1}{\kappa})^2+\Xi)^{n-1-i} (1-\frac{1}{\kappa})^{2i}\Xi.
\end{align}

To proceed, we consider two scenarios:

\textbf{Scenario 1: General $\Xi$:} When $\Xi$ is allowed to be large ($\Xi\geq \Omega(1/\kappa)$), we naively bound
\[
\gamma_n\leq \sum_{i=0}^{n-1}(1+\Xi)^{n-1-i}\Xi= (1+\Xi)^n-1.
\]

\textbf{Scenario 2: $\Xi\leq \frac{1}{4\kappa}$:} In this case, we observe $(1-\frac{1}{\kappa})^2+\Xi\leq (1-\frac{1}{2\kappa})^2$.%summing up the inequality, we obtain 
%\begin{align}
%\gamma_n&\leq (1-\frac{1}{2\kappa})^2\gamma_{n-1}+(1-\frac{1}{\kappa})^{2n-2}\Xi\leq (1-\frac{1}{2\kappa})^2\gamma_{n-1}+(1-\frac{1}{2\kappa})^{2n-2}\Xi
%\end{align}
%Summing up with $n\rightarrow\infty$, we obtain
%\[
%\sum_{n\geq 0}\gamma_n\leq 2\kappa \sum_{n\geq 0} (1-\frac{1}{\kappa})^{2n}\Xi\leq 2\kappa^2\Xi.
%\]
%Unrolling $\gamma_n$ recursively, 
This leads to the clean bound
\begin{align}
\gamma_n\leq \sum_{i=0}^{n-1}(1-\frac{1}{2\kappa})^{2(n-1-i)} (1-\frac{1}{\kappa})^{2i}\Xi\leq n(1-\frac{1}{2\kappa})^{2n-2}\Xi.\label{tighter bnd}
\end{align}
\end{proof}

To proceed, for general $\Xi$, through \eqref{naive bound}, we simply have
\[
\tn{\s_n-\E[\s_n]}^2\leq \frac{1}{L^2}N\sum_{n=0}^N( (1+\Xi)^n-1 )\leq \frac{1}{L^2}N^2((1+\Xi)^N-1)
\]
%\textbf{Scenario 2: $\Xi> \frac{1}{4\kappa}$:} 
%Set $B=|\Sc_n|$. This implies that $\gamma_N\leq \frac{2\sigma^2N}{L^2B}$ for $N\leq \frac{BL^2}{2\sigma^2}$. Thus, under advertised assumptions, setting $\tn{\vb}=1$, we obtain \eqref{conc2} via
%\[
%\frac{\E[\tn{\s_n-\E[\s_n]}^2]}{\tn{\vb}^2}\leq \frac{N+1}{L^2}\sum_{n=0}^N\gamma_n\leq \frac{(N+1)^3\sigma^2}{L^4B}.
%\]
On the other hand, when $\Xi\kappa \leq 1/4$, applying Cauchy-Schwarz and \eqref{tighter bnd}, we use
\[
\frac{\vb^\top \E[\Qt_i^\top \Qt_j]\vb}{\tn{\vb}^2}\leq \frac{ \E[\tn{\Qt_i\vb}\tn{\Qt_j\vb}]}{\tn{\vb}^2}\leq \sqrt{i(1-\frac{1}{2\kappa})^{2i-2}\Xi j(1-\frac{1}{2\kappa})^{2j-2}\Xi}\leq \frac{i+j}{2}(1-\frac{1}{2\kappa})^{i+j-2}\Xi.
\]
For a fixed $k=i+j$, there are at most $k-1$ pairs of $(i,j)$ (obeying $i,j\geq 1$) that can generate it. Summing up over all $0\leq i,j\leq N$, we find
\begin{align}
\frac{L^2\E[\tn{\s_n-\E[\s_n]}^2]}{\tn{\vb}^2}&\leq \sum_{k=2}^{2N}\frac{k(k-1)}{2}(1-\frac{1}{2\kappa})^{k-2}\Xi\\
&\leq \sum_{k=0}^{2N-2}\frac{k^2+3k+2}{2}(1-\frac{1}{2\kappa})^{k}\Xi\\
&\leq \frac{8\kappa^3(1-\frac{1}{2\kappa})(2-\frac{1}{2\kappa})+12\kappa^2(1-\frac{1}{2\kappa})+4\kappa}{2}\Xi\\
&\leq 8\kappa^3\Xi.
\end{align}
This concludes the proof.
%The final results follow by plugging in $N\gets N-1$ for cleaner notation on the right hand side.
%\newpage
\end{proof}
%\newpage

%\end{document}
