# Supplementary material for: Federated Multi-Sequence Stochastic Approximation with Local Hypergradient Estimation
Source: arXiv:2306.01648 source file (2023-06-02)
Supplement: Supplementary file 7 [file supp_localalgo.tex]

\section{\lfedblo}\label{sec:simp:algs}
Implementing \fedinn and \fedout naively by using the global direct and indirect gradients and sending the local information to the server that would then calculate the global gradients leads to a communication and space complexity of which can be  prohibitive for large-sized $d_1$ and $d_2$. One can consider possible local variants of \fedinn and \fedout tailore to such scenarios. Each of the possible algorithms (See Table~\ref{tabl:supp:methods}) can then either use the global gradient or only the local gradient, either use a SVRG or SGD. 
\begin{algorithm}[h]
\caption{$\m{x}^{+} ~=~\pmb{\lfedout}~(\m{x}, \m{y}, \alpha)$ for stochastic \colorbox{cyan!30}{bilevel}, \colorbox{green!30}{minimax}, and \colorbox{magenta!30}{compositional} problems
}
\begin{small}
\begin{algorithmic}[1]
 \State $\m{x}_{i,0}=\m{x}$ and $\alpha_i \in (0,\alpha]$ for each $i \in \mc{S}$.
 \State Choose $N \in \mb{N}$ (the number of terms of Neumann series).
 \For {$i \in \mc{S}$ \textbf{in parallel}} 
\For {$\nu=0,\ldots,\tau_i-1$} 
 \State%\colorbox{cyan!30}{
\colorbox{cyan!30}{Select $ N'\in \{0, \dots, N-1\}$ UAR.}
 \State%\colorbox{cyan!30}{
\colorbox{cyan!30}{$ \m{h}_{i,\nu }=\nabla_\m{x} f_i(\m{x}_{i,\nu },\m{y}; \xi_{i,\nu })-  \frac{N}{\ell_{g,1}} \nabla^2_{\m{xy}}g_i(\m{x}_{i,\nu },\m{y};{\zeta}_{i,\nu })  \prod\limits_{n=1}^{N'} \big(\m{I}-\frac{1}{\ell_{g,1}}\nabla^2_y g_i(\m{x}_{i,\nu }, \m{y};{\zeta}_{i,n})\big) \nabla_\m{x} f_i(\m{y}_{i,\nu },\m{y},\xi_{i,\nu })$}
 \State\colorbox{green!30}{$\m{h}_{i,\nu }=\nabla_{\m{x}} f_i(\m{x}_{i,\nu }, \m{y}; \xi_{i,\nu })$}
 \State \colorbox{magenta!30}{$\m{h}_{i,\nu }=\nabla \m{r}_i(\m{x}_{i,\nu };  \zeta_{i,\nu })^\top \nabla f_i(\m{y}_{i,\nu };  \xi_{i,\nu })$}
 \State  $ \m{x}_{i,\nu +1}= \m{x}_{i,\nu }-\alpha_i\m{h}_{i,\nu }$%~~\Comment{via automatic
  \EndFor
\EndFor
\State $\m{x}^{+}=|\mc{S}|^{-1}\sum_{i\in \mc{S}} \m{x}_{i,\tau_i}$
% \EndFor
\end{algorithmic}
\end{small}
\label{alg:localfedout}
\end{algorithm}
\begin{algorithm}[h]
\caption{$ \m{y}^+~=~\pmb{\lfedinn}~(\m{x},\m{y},\beta$) 
for stochastic \colorbox{cyan!30}{bilevel}, \colorbox{green!30}{minimax}, and \colorbox{magenta!30}{compositional} problems}
\begin{small}
\begin{algorithmic}[1]
 \State $\m{y}_{i,0}=\m{y}$ and $\beta_i \in (0,\beta]$ for each $i \in \mc{S}$.
 \For {$i \in \mc{S}$ \textbf{in parallel}} 
\For {$\nu=0,\ldots,\tau_i-1$} 
\State \colorbox{cyan!30}{$ \m{q}_{i,\nu }=\nabla_\m{y} g_i(\m{x}, \m{y}_{i,\nu };\zeta_{i,\nu })$} \colorbox{green!30}{$ \m{q}_{i,\nu }=-\nabla_\m{y} f_i(\m{x}, \m{y}_{i,\nu };\xi_{i,\nu })$} \colorbox{magenta!30}{$ \m{q}_{i,\nu }=\m{y}_{i,\nu }-\m{r}_i(\m{x};\zeta_{i,\nu })$}
\State $\m{y}_{i,\nu +1}= \m{y}_{i,\nu }-\beta_i\m{q}_{i,\nu }$
\EndFor
\EndFor
\State $\m{y}^{+}=|\mathcal{S}|^{-1}\sum_{i\in\mathcal{S}}\m{y}_{i,\tau_i}$
%\EndFor
\end{algorithmic}
\end{small}
\label{alg:localfedinn}
\end{algorithm}
\begin{table*}[h]
\centering
\scalebox{.9}{
\begin{tabular}{lccccccc}
\toprule 
 & \multicolumn{2}{c}{definition} & & \multicolumn{4}{c}{properties} \\ \cmidrule{2-3}\cmidrule{5-8} 
                            & outer & inner  & & global & global & global &  \#~communication \\
                       & optimizer  & optimizer & & outer gradient & IHGP& inner gradient & rounds \\
                       \midrule
\multirow{ 2}{*}{\pmb{\fedblo}} &Algorithm~\ref{alg:fedout}&Algorithm~\ref{alg:fedinn} && \multirow{ 2}{*}{yes}& \multirow{ 2}{*}{yes} & \multirow{ 2}{*}{yes}& \multirow{ 2}{*}{$2T+N+3$} \\
& (SVRG on $\m{x})$ & (SVRG on $\m{y})$ && &  & & \\
\hline
\multirow{ 2}{*}{\pmb{\lfedblo}}&Algorithm~\ref{alg:localfedout}&Algorithm~\ref{alg:localfedinn} && \multirow{ 2}{*}{no}& \multirow{ 2}{*}{no} &\multirow{ 2}{*}{ no}& \multirow{ 2}{*}{$T+1$} \\
& (SGD on $\m{x})$ & (SGD on $\m{y})$ && &  & & \\
\hline
\multirow{ 2}{*}{$\pmb{\fedblo}_\textbf{SGD}$} &Algorithm~\ref{alg:fedout}&Algorithm~\ref{alg:localfedinn} && \multirow{ 2}{*}{yes}& \multirow{ 2}{*}{yes} & \multirow{ 2}{*}{no}& \multirow{ 2}{*}{$T+N+3$} \\
& (SVRG on $\m{x})$ & (SGD on $\m{y})$ && &  & & \\

\hline
\multirow{ 2}{*}{$\pmb{\lfedblo}_\textbf{SVRG}$}&Algorithm~\ref{alg:localfedout}&Algorithm~\ref{alg:fedinn} && \multirow{ 2}{*}{no}& \multirow{ 2}{*}{no} &\multirow{ 2}{*}{ yes}& \multirow{ 2}{*}{$2T+1$} \\
& (SGD on $\m{x})$ & (SVRG on $\m{y})$ && &  & & \\

  \bottomrule
\end{tabular}
}
\caption{Definition of studied algorithms by using inner/outer optimization algorithms and server updates and resulting properties of these algorithms. $T$ and $N$ denote the number of inner iterations and terms of Neumann series, respectively.}
\label{tabl:supp:methods}
\vspace{-.3cm}
\end{table*}
