# Supplementary material for: Federated Multi-Sequence Stochastic Approximation with Local Hypergradient Estimation
Source: arXiv:2306.01648 source file (2023-06-02)
Supplement: Supplementary file 9 [file supp_minmax.tex]

\section {Proof for Federated Minimax Optimization}\label{sec:app:minmax}
Note that the  minimax optimization problem \eqref{fedminmax:prob} has the following bilevel form 
\begin{subequations}\label{fedminmax:prob2}
\begin{align}
\begin{array}{ll}
\underset{\m{x} \in \mb{R}^{{d}_1}}{\min} &
\begin{array}{c}
f(\m{x})=\frac{1}{m} \sum_{i=1}^{m} f_{i}\left(\m{x},\m{y}^*(\m{x})\right) %{\rm\sf (outer)} 
\end{array}\\
\text{subj.~to} & \begin{array}[t]{l} \m{y}^*(\m{\m{x}})=\underset{ \m{y}\in \mb{R}^{{d}_2}}{\textnormal{argmin}}~~ -\frac{1}{m}\sum_{i=1}^{m} f_i\left(\m{x},\m{y}\right). % ~~~~~~~~~~~~~~~~~~~~{\rm\sf (inner)} 
\end{array}
\end{array}
\end{align}
Here, 
\begin{align}
%\nonumber 
 %f_i(\m{x},\m{y}^*(\m{x})) &:= \mb{E}_{\xi \sim \mc{C}_i}[f_i(\m{x}, \m{y}^*(\m{x}); \xi)],\\
 f_i(\m{x},\m{y}) &= \mb{E}_{\xi \sim \mc{C}_i}[f_i(\m{x}, \m{y}; \xi)]
\end{align}
\end{subequations}
is the loss functions of the $i^{\text{th}}$ client.

In this case, the hypergradient of  \eqref{fedminmax:prob2} is  
\begin{equation}
	\nabla f_i(\m{x})=\nabla_\m{x} f_i\big(\m{x}, \m{y}^*(\m{x})\big)+\nabla_\m{x} \m{y}^*(\m{x})^{\top}\nabla_\m{y} f_i\big(\m{x}, \m{y}^*(\m{x})\big)=\nabla_\m{x} f_i\big(\m{x}, \m{y}^*(\m{x})\big), 
\end{equation}
where the second equality follows from the optimality condition of the inner problem, i.e., $\nabla_\m{y}f(\m{x},\m{y}^*(\m{x}))=0$.

For each $i \in \mc{S}$, we can approximate $\nabla f_i(\m{x})$ on a vector $\m{y}$ in place of $\m{y}^*(\m{x})$, denoted as $\overline{\nabla}f_i(\m{x},\m{y}):=\nabla_\m{x} f_i\big(\m{x}, \m{y}\big)$. We also note that in the minimax case $\m{h}_i$ is an unbiased estimator of $\bar{\nabla} f_i(\m{x},\m{y})$. Thus, $b=0$. Therefore, we can apply \fedblo  using 
\begin{equation}\label{eqn:grad:min-max}
\begin{aligned}
\m{q}_{i,\nu}&=-\nabla_{\m{y}} f_i(\m{x}, \m{y}_{i,\nu};\xi_{i,\nu})+\nabla_{\m{y}} f_i(\m{x}, \m{y};\xi_{i,\nu})-\frac{1}{m} \sum_{i=1}^m \nabla_{\m{y}} f_i(\m{x}, \m{y};\xi_{i}),\\
\m{h}_{i,\nu}&=\nabla_{\m{x}} f_i(\m{x}_{i,\nu}, \m{y}^+;\xi_{i,\nu})-\nabla_{\m{x}} f_i(\m{x}, \m{y}^+;\xi_{i,\nu})+
\frac{1}{m} \sum_{i=1}^m \nabla_{\m{x}} f_i(\m{x}, \m{y}^+;\xi_{i}).
%\m{h}(\m{x},\m{y}^+). 
\end{aligned}
\end{equation}

\subsection{Supporting Lemmas}

Let $\m{z}=(\m{x},\m{y}) \in \mb{R}^{d_1+d_2}$. We make the following assumptions that are counterparts of Assumptions~\ref{assu:f} and  \ref{assu:bound:var}.
\vspace{0.1cm}
% \noindent\textbf{Assumption 1 (Lipschitz continuity).}
%
\begin{assumption}\label{assu:f:minmax} 
%\noindent   {\bf Assumptions A}
For all $i \in [m]$:
\begin{enumerate}[label={\textnormal{\textbf{(\ref{assu:f:minmax}\arabic*})}}]
%[label={\textbf{(a\arabic*})}]
\item %[\textbf{a)}]
$f_i(\m{z}), \nabla f_i(\m{z}), \nabla^2 f_i (\m{z})$ are respectively $\ell_{f,0}$, $\ell_{f,1}, \ell_{f,2}$-Lipschitz continuous; and 
%That is, for $\m{z}_1:=[\m{x}_1;\m{y}_1]$, $\m{z}_2:=[\m{x}_2;\m{y}_2]$, we have $\|f(\m{x}_1,\m{y}_1)-f(\m{x}_2,\m{y}_2)\|\leq \ell_{f,0}\|\m{z}_1-\m{z}_2\|, \|\nabla f(\m{x}_1,\m{y}_1)-\nabla f(\m{x}_2,\m{y}_2)\|\leq \ell_{f,1}\|\m{z}_1-\m{z}_2\|, \|\nabla g(\m{x}_1,\m{y}_1)-\nabla g(\m{x}_2,\m{y}_2)\|\leq \ell_{g,1}\|\m{z}_1-\m{z}_2\|, \|\nabla^2 g(\m{x}_1,\m{y}_1)-\nabla^2 g(\m{x}_2,\m{y}_2)\|\leq \ell_{g,2}\|\m{z}_1-\m{z}_2\|$.
\item % [\textbf{d)}]
$f_i(\m{x},\m{y})$ is $\mu_{f}$-strongly convex in $\m{y}$ for any fixed $\m{x}\in \mb{R}^{d_1}$.
\end{enumerate}
\end{assumption}
We use $\kappa_f=\ell_{f,1}/\mu_f$ to denote the condition number of the inner objective with respect to $\y$.
%
% \begin{assumption}\label{ass:bound:var}%[Bounded Variance] 
% For all $\m{v}=(\m{x}, \m{y}) \in \mb{R}^{d_1+d_2}$:
% \begin{enumerate}[label={\textbf{(B\arabic*})}]
% \item %[\textbf{a)}]
% The function $G_i$ has $\sigma_i$-bounded variance, i.e., $\mb{E}[\|\nabla G_i(\m{v}, \zeta) - \nabla G_i(\m{v}, \zeta)\|^2] = \sigma_{i}^2$ for all  $i \in [n]$. 
% \item  Furthermore, we assume the (global) variance is bounded, $n^{-1} \sum_{i=1}^n \|\nabla G_i(\m{v}) - \nabla g_i(\m{v})\|^2 \leq \sigma_{g}^2$. 
% \end{enumerate}
% \label{asp:variance}
%\end{assumption}
% \noindent\textbf{Assumption 3 (Stochastic derivatives).}
\begin{assumption}\label{assu:bound:var:minmax}
For all $i \in [m]$:
\begin{enumerate}[label={\textnormal{\textbf{(\ref{assu:bound:var:minmax}\arabic*})}}]
\item $\nabla f_i(\m{z};\xi)$ is unbiased estimators of $\nabla f_i(\m{z})$; and
%$\mb{E}_{\xi}[\nabla f_i(\m{z};\xi)]=\nabla f_i(\m{z})$, $\mb{E}_{\zeta}[\nabla g_i(\m{z};\zeta)]=\nabla g_i(\m{z})$, $\mb{E}_{\zeta}[\nabla^2 g_i(\m{z}, \zeta)=\nabla g_i(\m{z})]$
%are unbiased estimators of $\nabla f_i(\m{z})$, $\nabla g_i(\m{z})$, and $\nabla^2g_i(\m{z})$, respectively; 
\item Its variance is bounded, i.e., $\mb{E}_{\xi}[\|\nabla f_i(\m{z};\xi)-\nabla f_i(\m{z})\|^2] \leq \sigma_f^2$,  for some $\sigma_f^2$.
\end{enumerate}
\end{assumption}
In the following, we re-derive Lemma~\ref{lem:lips} for the finite-sum minimax problem \eqref{fedminmax:prob2}. 
\begin{lemma}\label{lem:lips:minmax} 
Under Assumptions~\ref{assu:f:minmax} and \ref{assu:bound:var:minmax}, we have $\bar{\m{h}}_i (\m{x}, \m{y})=\bar{\nabla} f_i(\m{x},\m{y})$ for all $i \in \mc{S}$ and  \eqref{eqn:newlips:b}--\eqref{eqn:newlips:f} hold with 
% \begin{subequations}\label{eqn:newlips:minmax}
% 		\begin{align}
% \|\nabla f(\m{x}_1)-\nabla f(\m{x}_2)\|&	\leq  L_f\|\m{x}_1-\m{x}_2\|, \label{eqn:newlips:b:m}\\
% \|\m{y}^*(\m{x}_1)-\m{y}^*(\m{x}_2)\|&\leq  L_{\m{y}}\|\m{x}_1-\m{x}_2\|, \label{eqn:newlips:c:m}\\
% \|\nabla \m{y}^*(\m{x}_1)-\nabla \m{y}^*(\m{x}_2)\|&\leq  L_{yx}\|\m{x}_1-\m{x}_2\|, \label{eqn:newlips:d:m}\\
% %\mb{E}\left[\|\bar{\m{h}}_i (\m{x}, \m{y})- \m{h}_i(\m{x}, \m{y})\|^2\right] &\leq \tilde\sigma_f^2, \label{eqn:newlips:e:m}\\
% %\mb{E}\left[\|\m{h}_i(\m{x}_{i,\nu}, \m{y}^+)\|^2 |{\cal F}_{i, \ell-1} \right]  &\leq \tilde{D}_f,\label{eqn:newlips:f:m}
% \end{align}
% and for all~$i \in \mc{S}$, we have
% \begin{align}
% \|\bar{\nabla} f_i(\m{x},\m{y}) - \nabla f_i (\m{x},\m{y}^*(\m{x})) \|
% &	\leq  M_f\|\m{y}^*(\m{x})-\m{y}\|,~\textnormal{for all}~i \in \{1, \ldots, m\}, \label{eqn:newlips:a:m}\\
% \mb{E}\left[\|\bar{\m{h}}_i (\m{x}, \m{y})- \m{h}_i(\m{x}, \m{y})\|^2\right] &\leq \tilde\sigma_f^2, \label{eqn:newlips:e:m}\\
% \mb{E}\left[\|\m{h}_i(\m{x}_{i,\nu}, \m{y}^+)\|^2 |{\cal F}_{i, \nu-1} \right]  &\leq \tilde{D}_f.  \label{eqn:newlips:f:m}
% \end{align}
% \end{subequations}
% Here,
\begin{equation}\label{eqn:lip:condi:minimax}
\begin{split}
    &L_{yx}=\frac{\ell_{f,2}+\ell_{f,2}L_{\m{y}}}{\mu_f} + \frac{\ell_{f,1}(\ell_{f,2}+\ell_{f,2}L_{\m{y}})}{\mu_f^2}={\cal O}(\kappa^3_f),\\
    &M_f=\ell_{f,1}={\cal O}(1), ~~~ L_f=(\ell_{f,1}+\frac{\ell_{f,1}^2}{\mu_f})={\cal O}(\kappa_f), \\
     L_{\m{y}}&=\frac{\ell_{f,1}}{\mu_f}={\cal O}(\kappa_f),~~~\tilde\sigma_f^2 = \sigma_f^2,~~~ \tilde{D}_f^2=\ell_{l,0}^2 + \sigma_f^2,
\end{split}    
\end{equation}
where $\ell_{f,0}$, $\ell_{f,1}, \ell_{f,2}$, $\mu_f$, and $\sigma_f$ are given in Assumptions~\ref{assu:f:minmax} and \ref{assu:bound:var:minmax}.
\end{lemma}
% It can be observed that $h_f^k$ is an unbiased estimate of $\overline{\nabla}f(x^k,y^{k+1})$, that is, $\bar{h}_f^k=\overline{\nabla}f(x,y), b_k=0$.

\subsection{Proof of Corollary~\ref{thm:fednest:minmax}}
\begin{proof}
Let $\eta=1$. From \eqref{eq.step-cond-3} and \eqref{eqn2:dec:lyap}, we have
\begin{subequations}\label{eqn:scons:steps:minimax}
\begin{equation}%\label{eq.step-cond-3}
    \alpha_k=\min \left\{\bar\alpha_1, \bar\alpha_2, \bar\alpha_3,\frac{\bar\alpha}{\sqrt{K}}\right\},~~~~~~~\beta_k=\frac{\bar{\beta}\alpha_k}{T},
\end{equation}
 where 
\begin{equation}
\begin{aligned}
\bar{\beta}&=\frac{1}{\mu_g} \left(11 \ell_{f,1} L_{\m{y}} + L_{yx}\tilde{D}_f^2\bar\alpha_1 + \frac{\ell_{f,1}L_{\m{y}} \bar\alpha_1}{2}\right),\\
\bar\alpha_1&=\frac{1}{2L_f+4 \ell_{f,1} L_{\m{y}}+\frac{2 \ell_{f,1}L_{yx}}{L_{\m{y}}}},
~~~\bar\alpha_2= \frac{T}{8\ell_{g,1} \bar{\beta}}, 
%\frac{6T\rho_g}{\left(22M_fL_{\m{y}} + \eta L_{yx}\tilde{D}_f^2\bar\alpha_1 + M_fL_{\m{y}} \bar\alpha_1\right)}, 
~~~\bar\alpha_3= \frac{1}{216\ell_{f,1}^2+5\ell_{f,1}}. \\
\end{aligned}
\end{equation}
\end{subequations}
Using the above choice of stepsizes, \eqref{eqn:dec:final:bilevel} reduces to
\begin{equation}\label{eqn4:dec:lyap:minimax}
\begin{aligned}
    \frac{1}{K}\sum_{k=0}^{K-1}\mb{E}[\|\nabla f(\m{x}^k)\|^2]
    &\leq \frac{4\Delta_{\mb{W}}}{K\min\{\bar\alpha_1, \bar\alpha_2, \bar\alpha_3\}} + \frac{4\Delta_{\mb{W}}}{\bar{\alpha}\sqrt{K}} + \frac{4(c_1+c_2)\bar{\alpha}}{\sqrt{K}}\sigma_{f}^2,
\end{aligned}
\end{equation}
 where $\Delta_{\mb{W}}= \mb{W}^0-\mb{E}[\mb{W}^K]$, 
\begin{equation}\label{eqn:cons:cs:minimax}
    \begin{split}
     & c_1=\frac{25 \ell_{f,1}}{L_{\m{y}}}\left( 1+ \frac{11 \ell_{f,1} L_{\m{y}}}{2} \bar{\alpha}_1  +  \left(\frac{\ell_{f,1} L_{\m{y}} + 2 L_{\m{yx}}\tilde{D}_f^2 }{4} \right)\bar{\alpha}_1^2 \right)\bar{\beta}^2\frac{1}{T},%= \frac{\mc{O} (\kappa_f^3)}{T},
    \\
    &c_2=\frac{L_f +\frac{1}{2}}{2} + \ell_{f,1} L_{\m{y}} +\frac{L_{\m{yx}}\ell_{f,1}}{4 L_{\m{y}}}.       
    \end{split}
\end{equation}
Let $\bar{\alpha}=\mc{O}(\kappa^{-1}_f)$. Since by our assumption, $T=\mc{O}(\kappa_f)$, it follows from \eqref{eqn:lip:condi:minimax} and \eqref{eqn:cons:steps:minimax} that 
\begin{equation}\label{eqn:o:conditions}
    \bar\alpha_1={\cal O}(\kappa^{-2}_f),~~\bar\alpha_2={\cal O}(\kappa^{-1}_f),~~ \bar\alpha_3=\mc{O}(1),~~c_1= {\cal O}(\kappa^2_f), ~~c_2={\cal O}(\kappa^2_f).
\end{equation}
Substituting \eqref{eqn:o:conditions} in \eqref{eqn4:dec:lyap:minimax} and \eqref{eqn:cons:cs:minimax} gives
\begin{align}
    \frac{1}{K}\sum_{k=0}^{K-1}\mb{E}[\|\nabla f(\m{x}^k)\|^2]={\cal O}\left(\frac{\kappa^2_f}{K} + \frac{\kappa_f}{\sqrt{K}}\right).
\end{align}
To achieve $\varepsilon$-accuracy, we need $K={\cal O}(\kappa^2_f\varepsilon^{-2})$.
\end{proof}
