# Supplementary material for: Federated Multi-Sequence Stochastic Approximation with Local Hypergradient Estimation
Source: arXiv:2306.01648 source file (2023-06-02)
Supplement: Supplementary file 11 [file supp_single_level.tex]

\section{Proof for Federated Single-Level Optimization}\label{sec:app:sing}
Next, we re-derive Lemmas~\ref{lem:dec} and \ref{thm4:lemma2} for single-level nonconvex FL under Assumptions~\ref{assu:s:f} and \ref{assu:s:bound:var}. 

\begin{lemma}[Counterpart of Lemma~\ref{lem:dec}]\label{lem:s:dec}
Suppose Assumptions~\ref{assu:s:f} and \ref{assu:s:bound:var} hold. Further, assume $\tau_i \geq 1$ and $\alpha_i=\alpha/\tau_i$, for all $ i \in \mathcal{S}$ and some positive constant $\alpha$. Then, \fedout guarantees:
\begin{equation}
\begin{aligned}
\mb{E}\left[f(\m{x}^{+})\right] - \mb{E}\left[f(\m{x})\right]& \leq - \frac{\alpha}{2} \left(1- \alpha L_f\right) \mb{E}\left[\left\|\frac{1}{m}\sum\limits_{i=1}^{m} \frac{1}{\tau_i}\sum\limits_{\nu=0}^{\tau_i-1}  \nabla f_i(\m{x}_{i,\nu})\right\|^2\right]\\
   & - \frac{\alpha}{2} \mb{E}\left[\| \nabla f(\m{x})\|^2\right] + \frac{ \alpha L_f^2 }{ 2 m} \sum\limits_{i=1}^{m}   \frac{1}{\tau_i} \sum\limits_{\nu=0}^{\tau_i-1}  \mb{E}\left[\|\m{x}_{i,\nu} -\m{x}\|^2\right] +  \frac{\alpha^2 L_f}{2} \sigma_f^2.
\end{aligned}
\label{eqn0:lem:s:dec}
\end{equation}
\end{lemma}
\begin{proof}
By applying  Algorithm~\ref{alg:fedout} to the single-level optimization problem \eqref{fedsingle:prob2}, we get 
%\begin{subequations*}%\label{eqn:single:update}
%\begin{equation*}%\label{eqn:sl:update}
\begin{align*}
\m{x}_{i,0}=\m{x}~~\forall i\in\mathcal{S},~~~~\m{x}^{+}&=\m{x}- \frac{1}{m}\sum\limits_{i=1}^{m} \alpha_i \sum\limits_{\nu=0}^{\tau_i-1} \m{h}_i(\m{x}_{i,\nu}) - \m{h}_i(\m{x})  +\m{h}(\m{x})\\  
&=\m{x}- \frac{1}{m}\sum\limits_{i=1}^{m} \alpha_i \sum\limits_{\nu=0}^{\tau_i-1} \m{h}_i(\m{x}_{i,\nu}),
\end{align*}    
%\end{equation*}
where 
\begin{align*}%\label{eqn:sl:h:def}
\m{h}_i(\m{x}_{i,\nu})=\nabla f_i(\m{x}_{i,\nu};\xi_{i,\nu}),~~~~\m{h}_i(\m{x})=\nabla f_i(\m{x};\xi_{i,\nu}), ~~~~\textnormal{and}~~~~\m{h}(\m{x})= 1/m\sum_{i=1}^m \nabla f_i(\m{x};\xi_{i}).
\end{align*}
%\end{subequations*}
This together with  Assumption~\ref{assu:s:f} implies that 
\begin{equation}\label{eqn2:s:lem:dec}
    \begin{aligned}
\mb{E}\left[f(\m{x}^{+})\right] - \mb{E} \left[f(\m{x}) \right]
    \leq &   \mb{E} \left[\langle \m{x}^{+} - \m{x}, \nabla f(\m{x}) \rangle\right] + \frac{L_f}{2} \mb{E} \left[\Vert \m{x}^{+}-\m{x} \Vert^2 \right]\\
    = &- \mb{E}\left[ \left\langle \frac{1}{m}\sum\limits_{i=1}^{m} \alpha_i \sum\limits_{\nu=0}^{\tau_i-1} \m{h}_i(\m{x}_{i,\nu}) , \nabla f(\m{x}) \right\rangle \right]\\
    & +\frac{L_f}{2}  \mb{E}\left[ \left\| \frac{1}{m}\sum\limits_{i=1}^{m} \alpha_i \sum\limits_{\nu=0}^{\tau_i-1} \m{h}_i(\m{x}_{i,\nu})\right\|^2\right]. 
    \end{aligned}
\end{equation}
For the first term on the RHS of~\eqref{eqn2:s:lem:dec}, we obtain
%Further, for the second term in RHS of \eqref{eqn3:lem:dec}, we have 
\begin{equation}%\label{lemma12:eqn7}
\begin{aligned}
 - \mb{E}\left[ \left\langle \frac{1}{m}\sum\limits_{i=1}^{m} \alpha_i \sum\limits_{\nu=0}^{\tau_i-1}  \m{h}_i(\m{x}_{i,\nu}), \nabla f(\m{x}) \right\rangle \right] =& - \mb{E}\left[\frac{1}{m}\sum\limits_{i=1}^{m} \frac{\alpha}{\tau_i} \sum\limits_{\nu=0}^{\tau_i-1} \mb{E}\left[ \left\langle \m{h}_i(\m{x}_{i,\nu}), \nabla f(\m{x}) \right\rangle \mid {\cal F}_{i,\nu-1}  \right]\right]\\
%  =& - \mb{E}\left[ \left\langle \frac{1}{m}\sum\limits_{i=1}^{m} \alpha_i \sum\limits_{\nu=0}^{\tau_i-1} \nabla f_i(\m{x}_{i,\nu}) , \nabla f(\m{x}) \right\rangle  \right] \\
 =& - \frac{\alpha}{2} \mb{E}\left[\left\|  \frac{1}{m}\sum\limits_{i=1}^{m} \frac{1}{\tau_i} \sum\limits_{\nu=0}^{\tau_i-1} \nabla f_i(\m{x}_{i,\nu}) \right\|^2\right]- \frac{\alpha}{2} \mb{E}\left[\left\| \nabla f(\m{x})\right\|^2\right]\\
&+ \frac{\alpha}{2} \mb{E}\left[ \left\| \frac{1}{m}\sum\limits_{i=1}^{m} \frac{1}{\tau_i} \sum\limits_{\nu=0}^{\tau_i-1} \nabla f_i(\m{x}_{i,\nu})-\nabla f(\m{x})\right\|^2\right], \\
\leq& - \frac{\alpha}{2} \mb{E}\left[\left\|  \frac{1}{m}\sum\limits_{i=1}^{m} \frac{1}{\tau_i} \sum\limits_{\nu=0}^{\tau_i-1} \nabla f_i(\m{x}_{i,\nu}) \right\|^2\right]- \frac{\alpha}{2} \mb{E}\left[  \left\| \nabla f(\m{x})\right\|^2\right]\\
&+ \frac{\alpha L_f^2 }{2m} \sum\limits_{i=1}^{m}   \frac{1}{\tau_i} \sum\limits_{\nu=0}^{\tau_i-1}  \mb{E}\left[\left\|\m{x}_{i,\nu} -\m{x}\right\|^2\right].
%\\
 %& \leq -\|\bar{\m{h}}(\m{x},\m{y}^+)\|^2- \| \nabla f(\m{x})\|^2 +  2\|\bar{\nabla} f(\m{x},\m{y}^+)-\nabla f(\m{x})\|^2+ 2\|\bar{\m{h}}(\m{x},\m{y}^+)-\bar{\nabla} f(\m{x},\m{y}^+)\|^2 \\
% & \leq -\|\bar{\m{h}}(\m{x},\m{y}^+)\|^2- \| \nabla f(\m{x})\|^2 + 2M_f\|\m{y}^+-\m{y}^*(\m{x})\|^2+ 2b^2,\\
\end{aligned}
\label{eqn5:s:lem:dec}
\end{equation} 
Here, the first equality follows from the law of total expectation; the second equality uses $\mb{E}\left[\nabla f_i(\m{x}_{i,\nu})\right]= \mb{E}\left[\mb{E}\left[\m{h}_i(\m{x}_{i,\nu})|{\cal F}_{i,\nu-1}\right]\right]$ and the fact that 2 $\m{a}^\top \m{b} = \|\m{a}\|^2 + \|\m{b}\|^2 - \|\m{a}-\m{b}\|^2$; and the last inequality is obtained from Assumption~\ref{assu:s:f}.

For the second term on the RHS of~\eqref{eqn2:s:lem:dec}, Assumption~\ref{assu:s:bound:var} together with Lemma~\ref{lem:Jens} gives 
\begin{equation}
 \begin{aligned}
%\mc{A}_2
\mb{E}\left[ \left\| \frac{1}{m}\sum\limits_{i=1}^{m} \alpha_i \sum\limits_{\nu=0}^{\tau_i-1} \m{h}_i(\m{x}_{i,\nu})\right\|^2 \right]&= \alpha^2 \mb{E}\left[  \left\|\frac{1}{m}\sum\limits_{i=1}^{m} \frac{1}{\tau_i} \sum\limits_{\nu=0}^{\tau_i-1} \left( \m{h}_i(\m{x}_{i,\nu})- \nabla f_i(\m{x}_{i,\nu}) + \nabla f_i(\m{x}_{i,\nu}) \right) \right\|^2 \right]\\
 &\leq \alpha^2 \mb{E}\left[\left\|\frac{1}{m}\sum\limits_{i=1}^{m} \frac{1}{\tau_i}\sum\limits_{\nu=0}^{\tau_i-1}  \nabla f_i(\m{x}_{i,\nu})\right\|^2\right]+  \alpha^2 \sigma_f^2.
    \end{aligned}
\label{eqn6:s:lem:dec}
\end{equation}
Plugging \eqref{eqn6:s:lem:dec} and \eqref{eqn5:s:lem:dec} into \eqref{eqn2:s:lem:dec} gives the desired result.
\end{proof}

The following lemma provides a bound on the \textit{drift} of each $\m{x}_{i,\nu}$ from $\m{x}$ for stochastic nonconvex singl-level problems. It should be mentioned that similar drifting bounds are provided in the literature under either strong convexity~\citep{mitra2021linear} and/or bounded dissimilarity assumptions~\citep{wang2020tackling,reddi2020adaptive,li2020federated}. 

\begin{lemma}[Counterpart of Lemma~\ref{thm4:lemma2}]\label{thm4:s:lemma2}
Suppose Assumptions~\ref{assu:s:f} and \ref{assu:s:bound:var} hold. Further, assume $\tau_i \geq 1$ and $\alpha_i=\alpha/\tau_i, \forall i \in \mathcal{S}$, where $\alpha \leq 1/(3 L_f)$. Then, for all $\nu \in \{0,\ldots, \tau_i-1\}$, \fedout gives
\begin{align}\label{eqn1:lemm:s:drift}
 \mb{E}\left[\left\|\m{x}_{i,\nu}-\m{x}\right\|^2\right]\leq 12 \tau_i^2 \alpha_i^2  \mathbb{E}\left[\left\|\nabla  f(\m{x})\right\|^2\right] +  27 \tau_i \alpha_i^2 \sigma_f^2.
\end{align}
\end{lemma}
\begin{proof}
The result trivially holds for $\tau_i=1$. Similar to what is done in
the proof of Lemma~\ref{thm4:lemma2}, let $\tau_i>1$ and define
\begin{equation}\label{eqn1+:s:lemm:drift}
\begin{aligned}
\m{v}_{i,\nu}&:=\nabla f_i(\m{x}_{i,\nu})- \nabla f_i(\m{x}) + \nabla f (\m{x}),\\
\m{w}_{i,\nu}&:= \m{h}_i(\m{x}_{i,\nu})-\nabla f_i(\m{x}_{i,\nu})+  \nabla f_i(\m{x})-\m{h}_i(\m{x})+\m{h}(\m{x})- \nabla f(\m{x}).
\end{aligned}
\end{equation}
%where  $ \m{h}(\m{x})=
%1/m\sum_{i=1}^m \nabla_{\m{x}} f_i(\m{x};\xi_{i})$, $\m{h}_i(\m{x})=\nabla_{\m{x}} f_i(\m{x};\xi_{i,\nu})$, and $ \m{h}_i(\m{x}_{i,\nu})=\nabla_{\m{x}} f_i(\m{x}_{i,\nu};\xi_{i,\nu})- \m{h}_i(\m{x}) + \m{h}(\m{x})$.  

From Algorithm~\ref{alg:fedout}, for each $i\in\mathcal{S}$, and $\forall  \nu \in\{0,\ldots,\tau_i-1\}$, we obtain
\begin{equation*}
\begin{aligned}
        \m{x}_{i,\nu+1}-\m{x}&=\m{x}_{i,\nu}-\m{x}-\alpha_i \left(\m{h}_i(\m{x}_{i,\nu})-\m{h}_i(\m{x})+\m{h}(\m{x})\right)\\
          &= \m{x}_{i,\nu}-\m{x}-\alpha_i \left(\m{v}_{i,\nu}+\m{w}_{i,\nu}\right),
    \end{aligned}
\end{equation*}
which implies that 
\begin{equation}\label{eqn2:s:lemm:drift}
\begin{aligned}
\mb{E}\left[\|\m{x}_{i,\nu+1}-\m{x}\|^2\right]
&=\mb{E}\left[\|\m{x}_{i,\nu}-\m{x}-\alpha_i \m{v}_{i,\nu}\|^2\right]+\alpha_i^2\mb{E}\left[\|{\m{w}_{i,\nu}}\|^2\right]\\&-2\mb{E}\left[\mb{E}\left[\langle \m{x}_{i,\nu}-\m{x}-\alpha_i\m{v}_{i,\nu},\alpha_i \m{w}_{i,\nu} \rangle\mid\mathcal{F}_{i,\nu-1}\right]\right] \\ 
&= \mb{E}\left[\|\m{x}_{i,\nu}-\m{x}-\alpha_i\m{v}_{i,\nu}\|^2\right]+\alpha_i^2\mb{E}\left[\|\m{w}_{i,\nu}\|^2\right].
\end{aligned}
\end{equation}
Here, the last equality uses Lemma~\ref{lem:rand:zer} since  $\mb{E}[\m{w}_{i,\nu}|\mathcal{F}_{i,\nu-1}]=0$.

From  Assumption~\ref{assu:s:bound:var} and Lemma~\ref{lem:Jens}, for $\m{w}_{i,\nu}$ defined in \eqref{eqn1+:s:lemm:drift}, we have
\begin{equation}
\label{eqn3b:s:lemm:drift}
\begin{aligned}
\mb{E}\left[\|\m{w}_{i,\nu}\|^2\right] &\leq 3   \mb{E}\left[\|\m{h}_i(\m{x}_{i,\nu})-\nabla f_i(\m{x}_{i,\nu})\|^2+\|\nabla f_i(\m{x})-\m{h}_i(\m{x})\|^2+\|\m{h}(\m{x})- \nabla  f  (\m{x})\|^2\right]\\
        & \leq 9\sigma_f^2.
    \end{aligned}
\end{equation}
Substituting  \eqref{eqn3b:s:lemm:drift} into \eqref{eqn2:s:lemm:drift}, we get
\begin{equation}
\label{eqn4:s:lemm:drift}
\begin{aligned}
\mb{E}\left[\|\m{x}_{i,\nu}-\m{x}-\alpha_i\m{v}_{i,\nu}\|^2\right] &\leq  \left(1+\frac{1}{2\tau_i-1}\right)\mb{E}\left[\|\m{x}_{i,\nu}-\m{x}\|^2\right]+ 2\tau_i \alpha_i^2 \mb{E}\left[\|\m{v}_{i,\nu}\|^2\right] +9 \alpha_i^2\sigma_f^2 \\
       &\leq  \left(1+\frac{1}{2\tau_i-1}+4 \tau_i \alpha_i^2 L_f^2\right)\mb{E}\left[\|\m{x}_{i,\nu}-\m{x}\|^2\right]
 + 4 \tau_i \alpha_i^2  \mb{E}\left[\|\nabla f(\m{x})\|^2\right] +9 \alpha_i^2\sigma_f^2\\
        &\leq  \left(1+\frac{1}{\tau_i-1}\right)\mb{E}\left[\|\m{x}_{i,\nu}-\m{x}\|^2\right]+ 4 \tau_i \alpha_i^2  \mb{E}\left[\|\nabla f(\m{x})\|^2\right] +9 \alpha_i^2\sigma_f^2.
    \end{aligned}
\end{equation}
Here, the first inequality follows from Lemma~\ref{lem:trig}; the second inequality uses Assumption~\ref{assu:s:f} and Lemma~\ref{lem:Jens};
and the last inequality follows by noting $\alpha_i=\alpha/\tau_i, \forall i \in \mathcal{S}$ and $\alpha \leq 1/(3 L_f)$.

Now, iterating equation \eqref{eqn4:s:lemm:drift} and using $\m{x}_{i,0}=\m{x}, \forall i\in\mathcal{S}$, we obtain
\begin{equation}
\label{eqn6:lemm:drift}
    \begin{aligned}
        \mb{E}\left[\|\m{x}_{i,\nu}-\m{x}\|^2\right]&\leq  \left(   4 \tau_i \alpha_i^2  \mb{E}\left[\|\nabla f(\m{x})\|^2\right] +9 \alpha_i^2\sigma_f^2 \right) \sum\limits_{j=0}^{\nu -1} \left(1+\frac{1}{\tau_i-1}\right)^j\\
        &\leq 12 \tau_i^2 \alpha_i^2  \mb{E}\left[\|\nabla f(\m{x})\|^2\right] +27\tau_i \alpha_i^2 \sigma_f^2,
    \end{aligned}
\end{equation}
where the second inequality uses \eqref{eqn:sum:geom}. This completes the proof.
\end{proof}
\subsection{Proof of Theorem~\ref{thm:fednest:s:level}}
\begin{proof}
Let $\bar{\alpha}_1:= 1/(3L_f(1 + 8 L_f))$. Note that by our assumption $\alpha_k \leq \bar{\alpha}_1$. Hence, the stepsize $\alpha_k$ satisfies the condition of Lemma~\ref{thm4:s:lemma2}, and we also have $ 6 L_f^2 \alpha_k^3 \leq \alpha_k^2/4 \leq  \alpha_k/4$. This together with Lemmas \ref{lem:s:dec} and \ref{thm4:s:lemma2} gives
\begin{equation}\label{eqn:dec:s:lyap}
\begin{aligned}
    \mb{E}\left[f(\m{x}^{k+1})\right] - \mb{E} \left[f(\m{x}^k) \right] & \leq  -\frac{\alpha_k}{2}\mb{E}[\|\nabla f(\m{x}^k)\|^2] + \frac{L_f^2 \alpha_k }{2m}\sum \limits_{i=1}^m \frac{1}{\tau_i}\sum \limits_{\nu=0}^{\tau_i-1}\mb{E}\Big[\|\m{x}_{i,\nu}^k-\m{x}^k\|^2\Big]
\\
   & - \frac{\alpha_k}{2} (1- \alpha_k L_f) \mathbb{E}\left[ \left\| \frac{1}{m}\sum\limits_{i=1}^{m} \frac{1}{\tau_i} \sum\limits_{\nu=0}^{\tau_i-1} \nabla f_i(\m{x}_{i,\nu}^k)\right\|^2 \right] + \frac{\alpha^2_k L_f}{2} \sigma_f^2 
   \\
   & \leq   -\frac{\alpha_k}{2}\mb{E}[\|\nabla f(\m{x}^k)\|^2] + \frac{L_f^2 \alpha_k }{2m}\sum \limits_{i=1}^m \frac{1}{\tau_i}\sum \limits_{\nu=0}^{\tau_i-1}\mb{E}\Big[\|\m{x}_{i,\nu}^k-\m{x}^k\|^2\Big]+  \frac{\alpha^2_k L_f}{2}  \sigma_f^2
\\
&\leq  - \frac{\alpha_k}{2}\mb{E}[\|\nabla f(\m{x}^k)\|^2] + 6 L_f^2 \alpha_k^3 \mb{E}[\|\nabla f(\m{x}^k)\|^2] + \left(\frac{27}{2}\alpha_k^3  L_f^2 +  \frac{\alpha^2_k L_f}{2} \right)\sigma_f^2  \\
& \leq   - \frac{\alpha_k}{4}\mb{E}[\|\nabla f(\m{x}^k)\|^2] +  (1+L_f)  \alpha^2_k  \sigma_f^2, 
\end{aligned}
\end{equation}
where the second and last inequalities follow from  \eqref{eqn:param:s:choice}. 

Summing \eqref{eqn:dec:s:lyap} over $k$ and using our choice of stepsize in \eqref{eqn:param:s:choice}, we obtain
%and telescoping gives 
\begin{equation}\label{eqn:dec:s:final:bilevel}
\begin{aligned}
    \frac{1}{K}\sum_{k=0}^{K-1}\mb{E}[\|\nabla f(\m{x}^k)\|^2] %&\leq  \frac{4}{K\alpha}+ 5  L_f \sigma_{f}^2 \alpha \\
     &\leq \frac{4 \Delta_{f}}{K} \cdot  \min\left\{ \frac{1}{\bar{\alpha}_1},\frac{\sqrt{K}}{\bar{\alpha}}\right\} + 4 (1+L_f)  
      \sigma_{f}^2  \cdot \frac{\bar{\alpha}}{\sqrt{K}}  \\
 &\leq \left(\frac{4 \Delta_{f}}{ \bar{\alpha}_1}\right)\frac{1}{K} + \left( \frac{4\Delta_{f} }{\bar{\alpha}} + 4  (1+L_f) \bar{\alpha} \sigma_f^2 \right) \frac{1}{\sqrt{K}}, \\
 & \leq \mc{O}\left( \frac{ \Delta_f}{ \bar{\alpha}_1 K} + \frac{  \frac{\Delta_f}{\bar{\alpha}} + \bar{\alpha}\sigma_f^2 }{\sqrt{K}}\right),
\end{aligned}
\end{equation}
where $\Delta_{f}= f(\m{x}^0)-\mb{E}[f(\m{x}^K)]$.
%This completes the proof.
\end{proof}
