# Supplementary material for: Federated Multi-Sequence Stochastic Approximation with Local Hypergradient Estimation
Source: arXiv:2306.01648 source file (2023-06-02)
Supplement: Supplementary file 12 [file deter_neumann.tex]

%\section{Deterministic Local Neumann}
% \begin{algorithm}
%   \caption{Single round of local Neumann} 
% \begin{algorithmic}[1]
% \State \textbf{Inputs:} $(\A_i)_{i=1}^m,\bb,\vb,\eta$.
%   \State $\s= |\Sc|^{-1}\sum_{i\in\Sc}\A_i(\xi_{i}) \vb-\bb$
%   \State $\vb_{i,0} =\vb$  
%   \For {$\nu=0,\ldots,\tau-1$} 
% 		 \State $\vb_{i,\nu+1} = (\Iden-\eta\A_i(\xi_{i,\nu}))\vb_{i,\nu}$
% 		 \State $~~~~~~~~~~~~~~~+ \eta \A_i(\xi_{i,\nu})\vb-\eta \s$
% 	   \EndFor
% 	   \State \textbf{Return} $\hat{\vb}=|\Sc|^{-1}\sum_{i\in\Sc} \vb_{i,\tau}$
% \end{algorithmic}\label{local_Neumann_round}
% \end{algorithm}
% \begin{assumption} $\A_i(\zeta)$ is unbiased estimate of $\A_i$ with $\E\|\A_i(\zeta)-\A_i\|^2\leq \sigma^2$. When $\sigma=0$, we refer to the samples as \emph{deterministic}. Also assume $L\Iden\succeq \A_i\succeq \mu \Iden$ for all $i\in [m]$.
% \end{assumption}
