# Supplementary material for: Federated Multi-Sequence Stochastic Approximation with Local Hypergradient Estimation
Source: arXiv:2306.01648 source file (2023-06-02)
Supplement: Supplementary file 13 [file supp_fedDR.tex]

% \subsection{proof of Theorem~\ref{thm:DR+Neumann:convergence}}
% Douglas-Rachford splitting (DRS) solves problem \eqref{eq:isys:consensus:form} with the following iterations:
% \begin{subequations}\label{eq:DR:algorithm}
% \begin{align}
% \m{y}_{i,k} &= \text{prox}_{\eta}(\m{z}_{i,k})=\sum_{i=1}^m \sum_{j=0}^N \eta \left(\m{I}-\eta \m{A}_i\right)^j \m{b}_i, \label{eq: proximal f update} \\
% \m{w}_k &= \text{prox}_{\m{1}}(2\m{y}_{i,k}-\m{z}_{i,k})= \min_{\m{z}_i \in \mb{R}^{d_1}}  \|\m{A}_i \m{z}_i -\m{b}_i \|^2
% + \frac{1}{2}\|\m{z}_i - 2\m{y}_{i,k}-\m{z}_{i,k}\| \\
% &=\frac{1}{m}\sum_{i=1}^m(2\m{y}_{i,k}-\m{z}_{i,k}),  \label{eq: proximal g update}  \\
% \m{z}_{i,k+1} &= \m{z}_{i,k} +  \m{w}_k-\m{y}_{i,k},  \label{eq: x update}
% \end{align}
% \end{subequations}
% for $i \in [m]$, where $\text{prox}$ is the proximal operator and $\alpha$ is the proximal step size.   The goal of this work is to provide convergence rates for DRS over various assumptions on $f$, and optimize these rates with respect to the algorithm parameters $\alpha$ using semidefinite programs (SDPs).

% \begin{proof}
% For simplicity, we use the fact that the proximal operator for the function
% $\phi(\m{z}_1, \ldots, \m{z}_m) = \sum_{j=1} \phi_j(\m{z}_j)$ is
% block-separable, so that in terms of the block-partitioned vector $\m{z} =
% (\m{z}_1, \ldots, \m{z}_m)$, we have
% \begin{align*}
% \prox_{\eta \phi}(\m{z}) = \left(\prox_{\eta \phi_1}(\m{z}_1), \dots, \prox_{\eta
%   \phi_m}(\m{z}_m) \right), 
% \end{align*}
% and 
% \begin{align*}
% \refl_{\eta \phi}(z) = \left(\refl_{\eta \phi_1}(z_1), \dots, \refl_{\eta
%   \phi_m}(z_m)\right).
% \end{align*}
% %the reflected resolvent induced by $f$ is block-separable, taking the form
% Similarly, consider the approximate reflected resolvent defined by the
% algorithm, namely
% \begin{align*}
% \arefl(z) := 2 \aprox(z) - z, %\quad \mbox{for all $z = (z_1,
%  % \ldots, z_\numdevices) \in (\R^{d})^\numdevices$.}
% \end{align*}
% It also has the same block-separable form.  Let
% \begin{subequations}
% \begin{align}\label{eqn:t:oper}
% \mc{T}(z) &= \refl_{ \phi} \left(
% \refl_{I_\mc{C}}(z) \right), \textnormal{and}\\
% \wh{\mc{T}} & =  \arefl \big(\refl_{I_\mc{C}}(z)
% \big).
% \end{align}
% \end{subequations}
% %
% Algorithm~\ref{algo:FDR} generates the sequence
% $\{\m{z}^{(t)}\}_{t=1}^\infty$ via the updates $\m{z}^{(t+1)} =
% \wh{\mc{T}}(\m{z}^{(t)})$. Note that the the operators $\mc{T}$ and $\wh{\mc{T}}
% $ satisfy the relation
% \begin{align}\label{EqnPerturb}
% \wh{\mc{T}} - \mc{T} & =\arefl \circ \refl_{I_{\mc{C}}} -\refl_{\eta \phi} \circ \refl_{I_\mc{C}}.
% \end{align}
% Next, we show that  $\mc{T}$ is $\rho$-Lipschitz with $\rho=1- 2/(\sqrt{\kappa}+1)$. We note that  $\phi(z)=\sum_{j=1}^m \phi_j( \m{z}_j)$
% is $\mu_g$-strongly convex and $\ell_g$-smooth, known results on
% reflected proximal operators~\cite[Theorems 1 and 2]{giselsson2016linear} imply that with the stepsize choice $\eta = 1/\sqrt{\mu_g \ell_g}$, the
% operator $\refl_{\eta \phi}$ satisfies the bound
% \begin{align}\label{eqn:contr:refl}
% \|\refl_{\eta \phi}(z) - \refl_{\eta \phi}(z')\| & \leq \Big( 1 -
% \frac{2}{\sqrt{\kappa} + 1} \Big) \|z - z'\|
% \end{align}
% Applying the triangle inequality and using the operator $\mc{T}$, we have 
% \begin{align*}
%   \|\mc{T}(z) - \mc{T}(z')\| & \leq  \|
%   \refl_{\eta \phi} \big( \refl_{I_\mc{C}}(z) \big) - \refl_{\eta \phi}
%   \big( \refl_{I_\mc{C}}(z') \big)\| \\
% %
% & \stackrel{\rm (i)}{\leq}  \Big(1 -
%   \frac{2}{\sqrt{\kappa} + 1} \Big) \; \|\refl_{I_\mc{C}}(z) -
%   \refl_{I_\mc{C}}(z')\| \\
% %
% & \stackrel{\rm (ii)}{\leq} \Big( 1 - \frac{2}{\sqrt{\kappa} + 1}
%   \Big) \; \|z - z'\|,
% \end{align*}
% where step (i) uses the contractivity of
% the operator $\refl_{\eta \phi}$, and step (ii) uses the
% non-expansiveness of the operator $\refl_{I_\mc{C}}$. 

% Using this contractivity condition, we have
% procedure can be bounded as 
% \begin{align}
% \|\m{z}^{(t+1)} - \m{z}^*\| &=\|\wh{\mc{T}}\m{z}^{(t)}-\mc{T}\m{z}^*\| \nonumber\\
% %
%  & \stackrel{ (i)}{\leq} \|\mc{T}\m{z}^{(t)} - \mc{T} \m{z}^* \| + 2 \| \aprox
%   \refl_{I_\mc{C}} \m{z}^{(t)} - \prox_{\eta \phi} \refl_{I_\mc{C}} \m{z}^{(t)}\| \nonumber \\
%  & \stackrel{ (ii)}{\leq} \Big( 1 - \frac{2}{\sqrt{\kappa} + 1}
%   \Big) \|\m{z}^{(t)} - \m{z}^*\| + 2
%   \|\m{r}^{(t)}\| 
%   %\nonumber \\
%   %
% %& \leq \rho \|\m{z}^{(t)} - \m{z}^*\| + 2 \|\m{r}^{(t)}\|,
% \end{align}
% where inequality (i) applies the triangle inequality to the
% relation~\eqref{EqnPerturb} between the perturbed and idealized
% operators; step (ii) follows by definition of the residual $r^{(t)}$
% at round $t$, i.e.,
% \begin{align}
%  \m{r}^{(t)}:=\aprox(2\bar{z}^{(t)}-z^{(t)})-\prox_{\eta \phi}(2\bar{z}^{(t)} - z^{(t)}).
% \end{align}
% Since the fixed points of Algorithm~\ref{algo:FDR} are minimizers of $\phi$, hence unique under the strong convexity assumption. Consequently, we have
% \begin{align*}
% \|\m{s}^{(t + 1)} - \m{s}^\star\| \leq \frac{1}{\sqrt{m}} \|\m{z}^{(t + 1)} -
% \m{z}^\star\|, \qquad \mbox{for all $t = 1, 2, \ldots$.}
% \end{align*}
% Hence,
% \begin{align*}
% \|\m{s}^{(t + 1)} - \m{s}^\star\| \leq \frac{1}{\sqrt{m}} \left(1 -
% \frac{2}{\sqrt{\kappa} + 1} \right)^{\! t} \|\m{z}^{(1)}-\m{z}^\star\| +
% (\sqrt{\kappa} + 1) \mc{E}_{\textnormal{Neumann}},
% \end{align*}

% \textbf{Bounding  $\mc{E}_{\textnormal{Neumann}}$:}
% For $\m{z}$ and $\m{z}' \in \mathbb{R}^d$, define the iterates $\m{z}^n$ and $\bar{\m{z}}^n$ such that $\m{z}^0=\m{z}$ and $\bar{\m{z}}^{0}=\m{z}'$ and using the recursion:
% \begin{align}\label{eq:linear_recursion}
% \nonumber 
%  \m{v}_{i,\nu+1}&=\big(\m{I}-\eta_i\m{A}_i(\xi_{i,\nu})\big)\m{v}_{i,\nu} -\eta_i \big(|\mc{S}|^{-1}\sum_{i\in\mc{S}} \left(\m{A}_i(\xi_{i})\m{v}- \m{b}(\zeta_{i,n})\right)-\m{A}_i(\xi_{i,\nu})\m{v}\big)\\
%  %\m{v}_{i,\nu+1}&=\big(\m{I}-\eta_i\m{A}_i(\xi_{i,\nu})\big)\m{v}_{i,\nu} -\eta_i \big(|\mc{S}|^{-1}\sum_{i\in\mc{S}}\m{A}_i(\xi_{i})\m{v}- \m{b}(\zeta_{i,n})-\m{A}_i(\xi_{i,\nu})\m{v}\big),
% \\ 
% \bar{\m{z}}^n &= (\m{I} -\eta_i\m{A})\bar{\m{z}}^{n-1}-\eta_i\m{b}.
% 	\end{align}
% We have:
% 	\begin{align}
% 	\mathbb{E}\left[\|\m{z}^{n}-\bar{\m{z}}^{n}\|^2\right]=&\mathbb{E}\left(\m{z}^{n-1}- \bar{\m{z}}^{n-1}\right)^\top(\m{I}-\eta A)^2+\eta^2\Sigma_A \left(\m{z}^{n-1}- \bar{\m{z}}^{n-1}\right)\\
%  		&-2\eta\mathbb{E}\left[(\m{z}^{n-1}-\bar{\m{z}}^{n-1})^{\top}\right](\m{I}-\eta\m{A})(\hat{\m{b}}-\m{b})
% % 		&+ \beta^2\parens{\mathbb{E}\brakets{\Verts{\hat{b}-b}^2} + \mathbb{E}\brakets{\parens{\bar{z}^{n-1}}^{\top}\Sigma_A\bar{z}^{n-1}}} 
% % 		=& \mathbb{E}\brakets{\parens{z^{n-1}- \bar{z}^{n-1}}^{\top}\parens{(I-\beta A)^2+ \beta^2 \Sigma_A}
% % 		 \parens{z^{n-1}- \bar{z}^{n-1}}  }   \\
% % 		 &+\beta^2 \parens{\parens{\bar{z}^{n-1}}^{\top}\Sigma_A\bar{z}^{n-1}+ \mathbb{E}\brakets{\parens{\hat{b}-b}^{\top}\parens{ I + 2(I-\beta A)D_n}\parens{\hat{b}-b}}}  
% 	\end{align}

% % Let 
% % \begin{align*}
% % \rb_N= \Big[\frac{1}{m}\sum_{i=1}^m\Big((\Iden-\eta \A_i)^\tau+\eta \sum_{t=0}^{\tau-1}(\Iden-\eta \A_i)^t(\A_i-\A)\Big) \Big]^N\rb_0.
% % \end{align*}

% % \begin{align}%\label{eqn1:lem:dec}
% % \nonumber 
% %      \m{s}^{+}%&=\m{s}-\frac{1}{m}  \sum\limits_{i=1}^{m} \eta_i \sum\limits_{\nu=0}^{\tau_i-1}  \left( \m{h}(\m{v})-\m{h}_i(\m{v}^+)+\m{h}_i(\m{v})\right) \\
% %     &=\m{s}-\frac{1}{m}  \sum\limits_{i=1}^{m} \eta_i \sum\limits_{\nu=0}^{\tau_i-1} \m{h}_i(\m{v}).
% %  \end{align}
% %  where 
	
% \end{proof}



% \subsection{Proof of Theorem~\ref{thm:fednewton}}
% \begin{proof}
% 	We have that
% 	\begin{align}   
% 	\E_k[\|\m{x}^{k+1} - \m{x}^*\|] &= \E_k[\|\m{x}^k -\m{x}^*+ \m{p}_k^N\|]   \nonumber \\
% 	& \leq \underbrace{\E_k[\|\m{x}^k - \m{x}^* - \nabla^2f_{S_k}^{-1}(\m{x}^k)\nabla f(\m{x}^k)\|]}_\text{Term 4} +
% 	\underbrace{\E_k[\|\m{p}_k^N + \nabla^2f_{S_k}^{-1}(\m{x}^k)\nabla f(\m{x}^k)\|]}_\text{Term 5} . 
% 	\label{eqn:twoterm}
% 	\end{align}
	
	
% \end{proof}
