# Supplementary material for: Federated Multi-Sequence Stochastic Approximation with Local Hypergradient Estimation
Source: arXiv:2306.01648 source file (2023-06-02)
Supplement: Supplementary file 14 [file supp_fedMCO.tex]

% \section{Additional Experiment}
% In this section, we demonstrate the Algo.~\ref{alg:fedmsa} on \ref{fedmco_main} problem. Following \cite{balasubramanian2022stochastic}, we also conduct the experiment on risk-averse optimization which is given by the following form: $$\min_{x}{\bm{E}[U(x, \xi)]+\lambda(\bm{E}[\max(0, U(x,\xi)-\bm{E} [U(x,\xi)])^2])^{\tfrac{1}{2}}}.$$

% This problem is a stochastic three-level ($N=2$) composition optimization problem with 
% $$f_0(x) = (x, \bm{E}[U(x,\xi)]),$$
% $$f_1(x, y) = (y, \bm{E}[\max(0, U(x, \xi) - y)]),$$
% $$f_2(x, y) = x+ \lambda\sqrt{y+\delta}.$$

% The loss function can be written in the compositional form as:
% $f_2(f_1(f_0(x)))$

% We also note that to be consistent with \cite{balasubramanian2022stochastic}, in experiment, we also define $$U(x,\xi) = (b-g(a^\top x))^2\quad,\quad g(x)=x^2.$$

% For the experiment, we assueme $a\in\mathbb{R}^d$ is a zero-mean Gaussian random vector with a random covariance matrix $\Sigma_{i,j} \sim \mathcal{N}(0,1)$, and $\zeta \sim \mathcal{N}(0, 0.001\times I_d)$ is the noise. The true parameter $x^*\in \mathbb{R}^d$ is drawn from a standard Gaussian distribution and fixed. In the experiment, we choose $d=10$ and the total number of examples equals $1,000$.
% \begin{figure}[t]
%   \centering
%     \begin{tikzpicture}
%       \node at (0,0) {\includegraphics[scale=0.5]{figs/FedMCO/fedMCO.pdf}};
%       \node[scale=1.0] at (0,-3.1) {Communication rounds};
%       \node[scale=1.1, rotate=90] at (-4.2,-0.2) {$\|\m{x}-\m{x}^*\|$};
%     \end{tikzpicture}
%   \caption{ On \ref{eq:sc} problem, FedMSA achieves faster convergence compared to centralized gradient descent. }
%   \label{fig:supp_fedmco}
% \end{figure}
