# Supplementary material for: Federated Multi-Sequence Stochastic Approximation with Local Hypergradient Estimation
Source: arXiv:2306.01648 source file (2023-06-02)
Supplement: Supplementary file 15 [file supp_bilevel_draft.tex]

% \begin{algorithm*}[t]
% \caption{ Federated Multi-Sequence Stochastic Approximation}\label{alg:fedmsa}
% \begin{algorithmic}[1]
% \State Initialization $(\m{x},\m{y},\m{z})$, iteration number $R$, stepsize $\g{\alpha}=[\alpha^0,\ldots, \alpha^N]$, momentum parameters $\g{\rho}=[\rho^0,\ldots,\rho^N]$. 
% \For{$r=0, \ldots, R-1$} 
% %Set query function 
% %\State $\funcin_i(\cdot)\gets$ \colorbox{cyan!30}{$\nabla_\m{y} g_i(\m{x},\cdot)$~\text{(bilevel)}},\colorbox{green!30}{$-\nabla_\m{y} f_i(\m{x},\cdot)$~\text{(minimax)}}
% %\colorbox{magenta!30}{$-h_i(\cdot)$~\text{(composite)}},\\
% %\hspace{37pt}
% %\funcin_i\gets 
% % \State Server broadcasts  $\left(\m{Z}^{-}, \m{Z}\right)$
%  %\State Agents compute  $\m{p}_i\left(\m{x}, \m{Z}\right) + \xi_{i}$ and $\m{s}^n_i\left(\m{z}^{n-1},\m{z}^{n}\right)+\zeta_{i,n}$ send it to the server
% % \State Server computes  
%  \For {$m \in \mc{S}$ \textbf{in parallel}}  
%   \State Compute $\mb{F}^{m} \left( \m{x}_r,\m{Z}_{r}\right), \mb{F}^{m}\left(\m{x}_{r-1}, \m{Z}_{r-1}\right)$ and  $\mb{G}^{m,n}(\m{z}^{n-1}_{r},\m{z}^{n}_{r})$, $\mb{G}^{m,n}(\m{z}^{n-1}_{r-1},\m{z}^{n}_{r-1})$ for all $ n \in [N]$
% %   \hspace{-.5cm} Get $ \mb{F}^m \left(\m{x}_{r}, \m{Z}_{r}\right), \mb{F}^m\left(\m{x}_{r-1},\m{Z}_{r-1}\right)$
%  %\State \hspace{-.5cm} Get $\mb{G}^{m,n}(\m{z}^{n-1}_{r},\m{z}^{n}_{r})$, $\mb{G}^{m,n}(\m{z}^{n-1}_{r-1},\m{z}^{n}_{r-1})$
% %\EndIf 
% % \State $\m{q}_{i,n}=\mb{G}_{i,n}\left(\m{Z}_{n}\right)$
% %\State \colorbox{green!30}{$\m{q}_i=-\nabla_\m{y} f_i(\m{x}, \m{y};  \xi_{i})$}
% % \State \colorbox{magenta!30}{$\m{q}_i=-h_i(\m{x}; \zeta_{i})$}
%  \EndFor
%  \State $\m{h}_r= |\mathcal{S}|^{-1}\sum_{m\in\mathcal{S}}  \mb{F}^{m} \left(\m{x}_r,\m{Z}_{r}\right)+ (1-\rho^0)(\m{h}_{r-1}- |\mathcal{S}|^{-1}\sum_{m\in\mathcal{S}}  \mb{F}^{m}\left(\m{x}_r,\m{Z}_{r-1}\right)$
%   \State $\m{q}_r^n= |\mathcal{S}|^{-1}\sum_{m\in\mathcal{S}}  \mb{G}^{m,n}(\m{z}^{n-1}_{r},\m{z}^{n}_{r})+ (1-\rho^n) \left(\m{h}_{r-1}^{n}- |\mathcal{S}|^{-1}\sum_{m\in\mathcal{S}} \mb{G}^{m,n}(\m{z}^{n-1}_{r-1},\m{z}^{n}_{r-1})\right)$ for all $ n \in [N]$
%  %|\mathcal{S}|^{-1}\sum_{i\in\mathcal{S}} \m{Q}_{i}$
%   %\hspace{1.5cm}\texttt{\#communication}  
%  \For {$m \in \mc{S}$ \textbf{in parallel}} 
%  %\State Choose $\beta_i \in (0, \beta)$
%   \State  %$\m{x}_{0}^m=\m{x}$, 
%   $(\m{x}^{m}_{r+1,0},\m{Z}^{m}_{r+1,0})= (\m{x}_r,\m{Z}_r)$ and  $(\m{h}^{m}_{r+1,0}, \m{Q}^{m}_{r+1,0})=(\m{h}_{r},\m{Q}_{r})$ %for all    %$\m{q}^{n,m}_{r,0}=\m{q}^n_{r,0}$    %and $\alpha, \beta 
% \For {$k=0,\ldots,K-1$} 
% %\vspace{2mm}
% \State $\m{h}^{m}_{r,k}= \mb{F}^{m} \left(\m{x}^m_{r+1,k}  \m{Z}_{r+1,k}^m\right)+\m{h}^{m}_{r,k}-\mb{F}^{m} \left(\m{x}^m_{r+1,k-1},\m{Z}_{r+1,k-1}^m\right)$
% \State $\m{q}^{n,m}_{r,k}= \mb{G}^{m,n} \left(\m{z}^{m,n-1}_{r+1,k},\m{z}^{m,n}_{r+1,k}\right)+\m{q}^{m,n}_{r,k}-\mb{G}^{n,m} \left(\m{z}^{m,n-1}_{r+1,k-1},\m{z}^{m,n}_{r+1,k-1}\right)$  for all $ n \in [N]$
% \State $ \left(\m{x}_{r,k +1}^m,\m{Z}_{r,k +1}^m\right) = \m{Z}_{r,k }^m - \g{\alpha}  \m{H}_{r,k}^m$
% \EndFor
% \EndFor
% \State $\m{Z}_{r+1}=|\mc{S}|^{-1}\sum_{m\in\mc{S}} \m{Z}_{r,K}^m $
% %\hspace{1cm}\texttt{\#communication}  
% \EndFor
% \end{algorithmic}
% \end{algorithm*}


% In this paper, we consider federated stochastic approximation with multiple coupled sequences, which is used to find the root of a system of multiple coupled nonlinear equations. Specifically, given mappings $\mb{F}^{m}:\mathbb{R}^{d^0}\times \mathbb{R}^{d^1} \dots \times \mathbb{R}^{d^N} \mapsto \mathbb{R}^{d^0}$ and $\mb{G}^{m,n}:\mathbb{R}^{d^{n-1}}\times \mathbb{R}^{d_n} \mapsto \mathbb{R}^{d_n}$  for $n \in [N]:=\{1,\dots,N\}$, our goal is to find $\m{x}^*$ and $\m{Z}^*=[\m{z}^{1,*},\dots, \m{z}^{N,*}]$ such that
% \begin{equation}\label{fedmsa:prob}
% \begin{cases}
% \sum_{m=1}^M &\mb{F}^{m}\left(\m{x}^*,\m{Z}^*\right)=0\\
% \sum_{m=1}^M&\mb{G}^{m,n}\left(\m{z}^{0,*},\m{z}^{1,*}\right)=0\\
% &\vdots\\
% \sum_{m=1}^M&\mb{G}^{m,N}\left(\m{z}^{N-1,*},\m{z}^{N,*}\right)=0. %\\
% %\sum_{m=1}^M\mb{G}^{m,n}\left(\m{z}^{n-1,*},\m{z}^{n,*}\right)=&0. 
% \end{cases}    
% \end{equation}
% % \begin{equation}\label{fedmsa:prob}
% % \begin{cases}
% % \sum_{m=1}^M \mb{F}^m\left(\m{x}^*,\{\m{z}^{n,*}\}_{n=1}^N\right)=&0 \\
% % \sum_{m=1}^M\mb{G}^{m,n}\left(\m{z}^{n-1,*},\m{z}^{n,*}\right)=&0. 
% % \end{cases}    
% % \end{equation}
% % \begin{equation}\label{fedblo:prob}
% % =\sum_{i=1}^m\mb{G}^n_i\left(\m{z}^{n-1,*},\m{z}^{n,*}\right)=0.
% % \end{equation}
% Recall that $M$ is the number of clients. Here, to model mapping heterogeneity, each client $m$ is allowed to have its own mappings $(\mb{F}^m,\mb{G}^m)$. Moreover, we consider a general stochastic oracle model, access to local functions $(\m{s}_i,\m{p}_i)$ is via stochastic sampling as follows:% over stochastic functions (e.g.~local client data)
% \begin{align}
% %\nonumber 
% \mb{F}^{m}\left(\m{x},\m{Z}\right) &:= \mb{E}_{\xi \sim \mc{C}^m}\left[ \mb{F}^m\left(\m{x},\m{Z}\right)  + 
%  \xi\right],\\ 
%  \nonumber
%  \mb{G}^{m,n}\left(\m{z}^{n-1},\m{z}^{n}\right) &:= \mb{E}_{\zeta^n \sim \mc{D}^m}\left[ \mb{F}^{m,n}\left(\m{z}^{n-1},\m{z}^{n}\right)+ \zeta^n \right],
% \end{align}
% %\end{subequations}
% %are the loss functions of the $i^{\text{th}}$ client, 
% for all $n \in [N]$. Here, $(\xi, \zeta)\sim(\mc{C}^m, \mc{D}^m)$ are sampling distributions for the $m^{\text{th}}$ client. 

% %Before introducing the main results, we will first make some standard assumptions.
% %Throughout the discussion, we define $[N]\coloneqq \{1,2,...,N\}$, $[K]\coloneqq \{1,2,...,K\}$ and $\m{z}^0 \coloneqq x$ for conciseness.
% \begin{assumption}[Smoothness of the fixed points]\label{assum:lip:y*}
% For any $n \in [N]$:
% \vspace{-.3cm}
% \begin{enumerate}[label={\textnormal{\textbf{(A\arabic*})}}]
% \item %[\textbf{a)}]
% $\m{z}^{n-1} \in \mathbb{R}^{d_{n-1}}$, there exists a unique $\m{z}^{n,*}(\m{z}^{n-1}) \in \mathbb{R}^{d_n}$ such that $\mb{G}^n(\m{z}^{n-1},\m{z}^{n,*}(\m{z}^{n-1}))=0$. 
% \vspace{-.2cm}
% \item  $\m{z}^{n,*}(\m{z}^{n-1})$, $\nabla \m{z}^{n,*}(\m{z}^{n-1})$ are $\ell_{z,n}$ and $\ell_{z',n}$-Lipschitz continuous.
% \end{enumerate}
% \end{assumption}
% %$f_i(\m{w}), \nabla f_i(\m{w}), \nabla g_i(\m{w}), \nabla^2 g_i (\m{w})$ are $\ell_{f,0}$,$\ell_{f,1}$,$\ell_{g,1}$, $\ell_{g,2}$-Lipschitz continuous, respectively; and 

% % . Moreover, there exist constants $L_{y,n}$ and $L_{y',n}$ such that for any $\m{z}^{n-1},\dot{\m{z}}^{n-1}\in \mathbb{R}^{d_{n-1}}$, the following inequalities hold
% % \begin{subequations}
% % % \begin{align}\label{eq:y*lip}
% % %     \|y^{n,*}(y^{n-1}) - y^{n,*}(\Bar{y}^{n-1})\| &\leq L_{y,n} \|y^{n-1}-\Bar{y}^{n-1}\|,  \\
% % %     \label{eq:y*smooth}
% % %     \|\nabla y^{n,*}(y^{n-1}) - \nabla y^{n,*}(\Bar{y}^{n-1})\| &\leq L_{y',n} \|y^{n-1}-\Bar{y}^{n-1}\|.
% % % \end{align}
% % \begin{align*}
% % % \|\nabla f(\m{x}_1)-\nabla f(\m{x}_2)\|
% % % &	\leq  L_f\|\m{x}_1-\m{x}_2\|, \label{eqn:newlips:b}\\
% %  \|\m{z}^*(\m{z}^{n-1})-\m{z}^*(\dot{\m{z}}^{n-1})\|&\leq  L_{\m{z},n}\|\m{z}^{n-1}-\dot{\m{z}}^{n-1}\|, \label{eqn:newlips:c}\\
% % \|\nabla \m{z}^*(\m{z}^{n-1})-\nabla \m{z}^*(\dot{\m{z}}^{n-1})\|&\leq  L_{\m{zz},n}\| \m{z}^{n-1}- \dot{\m{z}}^{n-1}\|. \label{eqn:newlips:d}
% % \end{align*}
% %\end{subequations}

% % Due to the change of $y_k^{n-1}$ at each iteration, the solution of $h^n(y_k^{n-1},y^n)=0$ with respect to (w.r.t.) $y^n$, that is $y^{n,*}(y_k^{n-1})$, is drifting over consecutive iterations. Given $y_k^{n-1}$, since only one-step of $y_k^n$ update is performed at each iteration, one can only hope to establish convergence of $y_k^n$ if the drift of its optimal solution is controlled in some sense. Assumption \ref{assumption:y*} ensures both the zeroth-order and first-order drifts are controlled in the same scale of the change of $y_k^{n-1}$. This assumption is satisfied in linear SA \citep{kaledin2020finite} and other applications which will be shown later.

% % Define $v(x) \coloneqq v\big(x,y^{1,*}(x), y^{2,*}(y^{1,*}(x)),\dots,y^{N,*}(\dots y^{2,*}(y^{1,*}(x))\dots)\big)$. With $y^{1:N}$ as a concise notation for $(y^1,...,y^N )$, we make the following assumption.
% % \begin{assumption}[Well-behaved increments]\label{assum:lipmaps}
% % For any $n \in [N]$, $\m{x},\dot{\m{x}} \in \mathbb{R}^{d_0}$ and $\m{z}^n, \dot{\m{z}}^n \in \mathbb{R}^{d_n}$, there exist constants $L_f$, $L_{f,\m{z}}$ and $L_{g,n}$ such that the following inequalities hold
% % %\begin{subequations}
% % \begin{align*}
% % \label{eq:v lip}    \|\mb{F}_i(\m{z}) - \mb{F}_i(\dot{\m{z}})\|&\!\leq\! L_f \|\m{z}-\dot{\m{z}}\|,\\
% %     \|\mb{F}_i(\m{x},\m{z}^{1:N})\!-\!\mb{F}_i(\m{x},\dot{\m{z}}^{1:N})\| &\!\leq\! L_{f,\m{z}} \!\sum_{n=1}^N\!\|\m{z}^n \!-\!\dot{\m{z}}^n\|,\! \\
% %     \|\mb{G}_i^n(\m{z}^{n-1},\m{z}^n)\!-\! \mb{G}_i^n(\m{z}^{n-1},\dot{\m{z}}^n)\| &\!\leq\! L_{g,n} \|\m{z}^n -\dot{\m{z}}^n\|.
% % \end{align*}
% % %\end{subequations}
% % \end{assumption}

% We will use $\mathcal{F}^{m}_{r,k}$ to denote the filtration that captures all the randomness up to the $k$-th local step of client $m$ in round $r$. 
% %With a slight abuse of notation, $\mathcal{F}^{m}_{i,-1}$ is to be interpreted as $\mathcal{F}^{k,t}, \forall i \in \mc{S}$. For simplicity, we remove subscripts $k$ and $t$ from the definition of stepsize and model parameters. 
% \begin{assumption}[Bias and variance]\label{assum:bias}
% There exist constants $\{c_n,\sigma_n\}_{n=0}^N$ such that $\forall k, n$,
% \begin{enumerate}[label={\textnormal{\textbf{(B\arabic*})}}]
% \item $\|\E[\xi_{r,k} | \mathcal{F}_{r,k}^1]\|^2 \leq c_0^2\alpha_k$ and $\|\E[\zeta_{r,k}^n | \mathcal{F}_k^{n+1}]\|^2\leq c_n^2\beta_{k,n}$
% \item  $\E[\|\xi_{r,k}\|^2 | \mathcal{F}_{r,k}^1] \leq \sigma_0^2$ and $\E[\|\zeta_{r,k}^n\| | \mathcal{F}_{r,k}^{n+1}] \leq \sigma_n^2$.
% \end{enumerate}
% \end{assumption}

% \begin{assumption}[Monotonicity of $\mb{G}$]\label{assum:stmonot:g}
% For  $ n \in [N]$ and $m \in [M]$, $\mb{G}^{m,n}(\m{z}^{n-1},\m{z}^n)$ is one-point strongly monotone on $\m{z}^{n,*}(\m{z}^{n-1})$ given any $\m{z}^{n-1}$.
% % ; that is 
% % \begin{align*}
% %     \big\langle \m{z}^n\!-\!\m{z}^{n,*}(\m{z}^{n-1}),\mb{G}^n(\m{z}^{n-1},\m{z}^n) \big\rangle \leq -\lambda_n \|\m{z}^n\!-\!\m{z}^{n,*}(\m{z}^{n-1})\|^2,
% % \end{align*}
% % for some $\lambda_n>0$.
% \end{assumption}

% \begin{theorem}\label{thm:fedmsa:strong:mon}
% Suppose Assumptions~\ref{assum:lip:y*}--\ref{assum:stmonot:g} hold. Further, assume $\alpha^k=\mc{O}(\frac{1}{k})$ and $\beta^k=\mc{O}(\frac{1}{k})$, then it holds for any $k$ that
% \begin{equation*}
%     \E\|\m{x}_k-\m{x}^*\|^2 +  \sum_{n=1}^N\E \left\|\m{z}_k^n-\m{z}^{n,*}(\m{z}_k^{n-1})\right\|^2 
%     = \mathcal{O}\Big(\frac{1}{k} \Big)
% \end{equation*}
% where $\mathcal{O}(\cdot)$ hides constants in the polynomial of $N$. 
% \end{theorem}

% \begin{assumption}[Heterogeneity of $\mb{F}$]\label{assum:heter:f}
%  The set of $\{\mb{F}^{m}(\m{x}, \m{Z})\}$ satisfies the first and second order Heterogeneity assumption, i.e., 
% $\sup_{(\m{x}, \m{Z})} \sum_{m=1}^M\|\mb{F}^{m}(\m{x}, \m{Z})-\mb{F}(\m{x}, \m{Z}) \|/M \leq \tau^1$ and $ \sup_{(\m{x}, \m{Z})} \sup_{m \in [M]}\|\nabla\mb{F}^{m}(\m{x}, \m{Z})-\nabla \mb{F}(\m{x}, \m{Z}) \| \leq \tau^2$ for some $(\tau^1, \tau^2)$.
% % \begin{enumerate}[label={\textnormal{\textbf{(D\arabic*})}}]
% % \item 
% % %[\textbf{a)} 
% % %$\m{z}^{n-1} \in \mathbb{R}^{d_{n-1}}$, there exists a unique $\m{z}^{n,*}(\m{z}^{n-1}) \in \mathbb{R}^{d_n}$ such that $\mb{G}^n(\m{z}^{n-1},\m{z}^{n,*}(\m{z}^{n-1}))=0$. 
% % \vspace{-.2cm}
% % \item 
% % \end{enumerate}
% %$\mb{F}^{m}(\m{x},\m{Z})$ is one-point strongly monotone on $\m{z}^{n,*}(\m{z}^{n-1})$ given any $\m{z}^{n-1}$.
% % ; that is 
% % \begin{align*}
% %     \big\langle \m{z}^n\!-\!\m{z}^{n,*}(\m{z}^{n-1}),\mb{G}^n(\m{z}^{n-1},\m{z}^n) \big\rangle \leq -\lambda_n \|\m{z}^n\!-\!\m{z}^{n,*}(\m{z}^{n-1})\|^2,
% % \end{align*}
% % for some $\lambda_n>0$.
% \end{assumption}
% \begin{theorem}\label{thm:fednest}
% Suppose Assumptions~\ref{assum:lip:y*}--\ref{assum:heter:f} hold. Further, assume $\alpha^k=\mc{O}(\frac{1}{k})$ and $\beta^k=\mc{O}(\frac{1}{k})$, then it holds for any $k$ that
% \begin{align*}
%     &\E \left\|\mb{F}(\m{x}_k)\right\|^2 + \sum_{n=1}^N\E \left\|\m{z}_k^n-\m{z}^{n,*}(\m{z}_k^{n-1})\right\|^2 \qquad \qquad \\
%      & \leq \frac{\tau_1 \Delta}{R} +\frac{\Delta \ell_{f,1}}{\sqrt{K}R} + \frac{\sigma^2}{MKR} + \left(\frac{\sigma \Delta \ell_{f,1}}{MKR}\right)^{3/2}
% \end{align*}
% where $\mathcal{O}(\cdot)$ hides constants in the polynomial of $N$. 
% \end{theorem}


%\input{sec/intro_application}


\section{Proof of Theorem~\ref{th}}

Throughout the proof, we will use $\mathcal{F}^{k,t}_{i,\nu}$ to denote the filtration that captures all the randomness up to the $\nu$-th local step of client $i$ in inner round $t$ and outer round $k$. With a slight abuse of notation, $\mathcal{F}^{k,t}_{i,-1}$ is to be interpreted as $\mathcal{F}^{k,t}, \forall i \in \mc{S}$. For simplicity, we remove subscripts $k$ and $t$ from the definition of stepsize and model parameters. For example, $\m{x}$ and $\m{x}^+$ denote $\m{x}^k$ and $\m{x}^{k+1}$, respectively. We further set 
 \begin{align}\label{eqn:expe:h}
 \bar{\m{h}}_i (\m{x}_{i,\nu}, \m{y}^+)&:=\mb{E}\Big[\m{h}_i(\m{x}_{i,\nu}, \m{y}^+)|{\cal F}_{i,\nu-1}\Big].    
 \end{align}

%
\begin{lemma}\label{thm:fedin} 
Suppose Assumptions~\ref{assum:lip:y*}--\ref{assum:stmonot:g} hold.  Further, assume 
% \begin{equation*}
% \tau_i \geq 1,~~~~\alpha_i=\frac{\alpha}{\tau_i},~~~~\beta_i=\frac{\beta}{\tau_i},~~~~\forall i \in \mathcal{S},    
% \end{equation*}
% where  
$\beta <  \min\big(1/(6\ell_{g,1}),1\big)$ and $\alpha$ is some positive constant. Then, Algorithm~\ref{alg:fedmsa} guarantees: 
\begin{subequations}\label{eqn:err:fedin1}
\begin{align}
  \mb{E}\left[\left\|\m{y}^{+}\!\!-\m{y}^\star(\m{x})\right\|^2\right]& \leq  \left(1-  \frac{{\beta} \mu_g}{2} \right)^T \mb{E}\left[\left\| \m{y}- \m{y}^\star(\m{x}) \right\|^2\right] +25 T {\beta}^2 \sigma^2_{g,1},~~~\textnormal{and} \label{eqn:err:fedina1}\\
 \nonumber  
  \mb{E}\left[\left\|\m{y}^{+}-\m{y}^\star(\m{x}^{+})\right\|^2\right] &\leq a_1(\alpha)  \mb{E}\left[ \left\| \frac{1}{m}\sum\limits_{i=1}^{m} \frac{1}{\tau_i} \sum\limits_{k=0}^{K-1} \bar{\m{h}}_i(\m{x}_{i,\nu},\m{y}^+)\right\|^2 \right]\\
 &+ a_2(\alpha) \mb{E}\left[\left\|\m{y}^+\!\!-\m{y}^\star(\m{x})\right\|^2\right] +a_3(\alpha) \tilde{\sigma}_f^2.
 \label{eqn:err:fedinb1}
  %\label{eq:fedinn2} 
\end{align}
\end{subequations}
%\ct{added $2$'s above}
Here,
\begin{equation}\label{eqn:a1-3}
\begin{aligned}
a_1(\alpha) &:=  L_{\m{y}}^2 \alpha^2+ \frac{L_{\m{y}}\alpha}{4M_f} +\frac{L_{\m{yx}} \alpha^2}{2\eta},\\
a_2(\alpha)  &:=  1+ 4M_f L_{\m{y}} \alpha + \frac{\eta L_{\m{yx}}\tilde{D}_f^2 \alpha^2}{2}, \\
a_3(\alpha) &:=  \alpha^2  L_{\m{y}}^2  +\frac{L_{\m{yx}} \alpha^2}{2\eta},
\end{aligned}
\end{equation}
for any $\eta>0$.
\end{lemma}
\begin{proof}
Note that 
\begin{align}\label{eqn-1:dec:fedin}
\nonumber 
 \mb{E}\left[\|\m{y}^{+}-\m{y}^*(\m{x}^{+})\|^2\right] =& \mb{E}\left[\|\m{y}^{+}-\m{y}^*(\m{x})\|^2\right] + \mb{E}\left[\|\m{y}^*(\m{x}^{+})-\m{y}^*(\m{x})\|^2\right]\\
+&2\mb{E}\left[\langle \m{y}^{+}-\m{y}^*(\m{x}), \m{y}^*(\m{x})-\m{y}^*(\m{x}^{+})\rangle\right].
\end{align}
%
Next, we upper bound each term on the RHS of~\eqref{eqn-1:dec:fedin}.
\\
\textbf{Bounding the first term in \eqref{eqn-1:dec:fedin}}:\\


From \citep[Theorem 4]{mitra2021linear}, for all $t \in \{0,\ldots,T-1\}$, we obtain
%\begin{subequations}
\begin{equation*}%\label{eqn0-1:dec:fedin}
    \mb{E}[{\Vert\m{y}^{t+1}- \m{y}^\star(\m{x})\Vert}^2] \leq \left(1-  \frac{{\beta} \mu_g}{2} \right) \mb{E}[{\Vert \m{y}^{t}- \m{y}^\star(\m{x})\Vert}^2] +25 {\beta}^2 \sigma^2_{g,1},
\end{equation*}
which together with our setting $\m{y}^+= \m{y}^{T}$ implies
\begin{equation}\label{eqn0:dec:fedin}
\mb{E}[\|\m{y}^{+}-\m{y}^*(\m{x})\|^2] \leq \left(1-  \frac{{\beta} \mu_g}{2} \right)^T \mb{E}[{\Vert \m{y}- \m{y}(\m{x}^*) \Vert}^2] +25 T {\beta}^2 \sigma^2_{g,1}.
\end{equation}
%
\textbf{Bounding the second term in \eqref{eqn-1:dec:fedin}}:\\
By similar steps as in \eqref{eqn6:lem:dec}, we have
\begin{equation}
\begin{aligned}\label{eqn1:dec:fedin}
 \mb{E}\left[\|\m{y}^*(\m{x}^{+})-\m{y}^*(\m{x})\|^2\right] &\leq  L_{\m{y}}^2 \mb{E}\left[\left\| \frac{1}{m}\sum\limits_{i=1}^{m} \alpha_i \sum\limits_{k=0}^{K-1}  \m{h}_i(\m{x}, \m{y}^+)\right\|^2\right] \\
&\leq   L_{\m{y}}^2 \mb{E}\left[\norm[\bigg]{\frac{1}{m}\sum\limits_{i=1}^{m}\alpha_i \sum\limits_{k=0}^{K-1}  \bar{\m{h}}_i(\m{x}_{i,\nu}, \m{y}^+)}^2\right]+  \alpha^2  L_{\m{y}}^2 \tilde{\sigma}_f^2,
\end{aligned}
\end{equation}
where the inequalities are obtained from Lemmas~\ref{lem:lips} and \ref{lem:rand:zer}.
%and \ref{lem:neum:bias}. %\ct{detail: lemma \ref{lem:neum:bias} doesn't seem to be used here.} 

\textbf{Bounding the third term in \eqref{eqn-1:dec:fedin}}:\\
Observe that %\ct{Drop the $2$ on LHS below}
\begin{equation}
\label{eqn2:dec:fedin}
    \begin{aligned}
%\begin{align*}\label{eq.lemma2-new-pf-4-0}
\mb{E}\left[\langle \m{y}^{+}-\m{y}^*(\m{x}), \m{y}^*(\m{x})-\m{y}^*(\m{x}^{+})\rangle \right] &= -\mb{E}\left[\langle\m{y}^+\!\!-\m{y}^\star(\m{x}), \nabla \m{y}^\star(\m{x})(\m{x}^+\!\!-\m{x})\rangle \right]
\\
&\quad -\mb{E}\left[\langle\m{y}^+\!\!-\m{y}^\star(\m{x}), \m{y}^\star(\m{x}^+)-\m{y}^\star(\m{x})-\nabla \m{y}^\star(\m{x})(\m{x}^+\!\!-\m{x})\rangle \right].
\end{aligned}
\end{equation}
For the first term on the R.H.S. of the above equality, we have
\begin{equation}
\label{eqn3:dec:fedin}
    \begin{aligned}
 -\mb{E}[\langle\m{y}^+\!\!-\m{y}^\star(\m{x}), \nabla \m{y}^\star(\m{x})(\m{x}^+\!\!-\m{x})\rangle]  %=&-\mb{E}[\langle{\m{y}^+\!\!-\m{y}^\star(\m{x}), \mb{E}[\nabla \m{y}^\star(\m{x})(\m{x}^+\!\!-\m{x})\mid \mc{F}']\rangle}]\\
%=&-\mb{E}[\langle{\m{y}^+\!\!-\m{y}^\star(\m{x}), \mb{E}[\nabla \m{y}^\star(\m{x})(\m{x}^+\!\!-\m{x})]\rangle}]\\
=&-\mb{E}\left[\langle{\m{y}^+\!\!-\m{y}^\star(\m{x}), \frac{1}{m} \nabla \m{y}^\star(\m{x}) \sum\limits_{i=1}^{m} \alpha_i \sum\limits_{k=0}^{K-1} \bar{\m{h}}_i(\m{x}_{i,\nu},\m{y}^+) \rangle}\right]\\
 \leq & \mb{E}\left[\left\|\m{y}^+\!\!-\m{y}^\star(\m{x})\right\|  \left\| \frac{1}{m} \nabla \m{y}^\star(\m{x})\sum\limits_{i=1}^{m} \alpha_i \sum\limits_{k=0}^{K-1} \bar{\m{h}}_i(\m{x}_{i,\nu},\m{y}^+)\right\|\right]\\
\leq & L_{\m{y}}\mb{E}\left[\left\|\m{y}^+\!\!-\m{y}^\star(\m{x})\right\| \left\| \frac{1}{m}\sum\limits_{i=1}^{m} \alpha_i \sum\limits_{k=0}^{K-1} \bar{\m{h}}_i(\m{x}_{i,\nu},\m{y}^+)\right\|\right]\\
\leq &  2 \gamma\mb{E}\left[\left\|\m{y}^+\!\!-\m{y}^\star(\m{x})\right\|^2\right] + \frac{L_{\m{y}}^2 \alpha^2}{8\gamma } \mb{E}\left[\left\| \frac{1}{m}\sum\limits_{i=1}^{m} \frac{1}{\tau_i} \sum\limits_{k=0}^{K-1} \bar{\m{h}}_i(\m{x}_{i,\nu},\m{y}^+)\right\|^2\right],
\end{aligned}
\end{equation}
where the first equality uses the fact that $\bar{\m{h}}_i (\m{x}_{i,\nu}, \m{y}^+)=\mb{E}\left[\m{h}_i(\m{x}_{i,\nu}, \m{y}^+)|{\cal F}_{i,\nu-1}\right]$;  the second inequality follows from Lemma~\ref{lem:lips}; %\ct{Isn't this just CS inequality?}, \ct{To confirm: in second inequality, spectral norm of $\nabla \y^*(x)$ is bounded by $L_{\m{y}}$ because $\y^*(\x)$ is cvx? };
and the last inequality is obtained from the Young's inequality such that $ab\leq 2\gamma a^2+\frac{b^2}{8\gamma}$.

Further, using Lemma \ref{lem:lips}, we have 
\begin{equation}
\label{eqn4-:dec:fedin}
\begin{aligned}
-&\mb{E}[\langle\m{y}^+\!\!-\m{y}^\star(\m{x}),  \m{y}^\star(\m{x}^+)-\m{y}^\star(\m{x})-\nabla \m{y}^\star(\m{x})(\m{x}^+\!\!-\m{x})\rangle] \\
& \leq  \mb{E}\left[\left\|\m{y}^+\!\!-\m{y}^\star(\m{x})\| \|\m{y}^\star(\m{x}^+)-\m{y}^\star(\m{x})-\nabla \m{y}^\star(\m{x})(\m{x}^+\!\!-\m{x})\right\|\right] \\
&\leq \frac{L_{\m{yx}}}{2}\mb{E}\left[\left\|\m{y}^+\!\!-\m{y}^\star(\m{x})\right\|\left\|\m{x}^+\!\!-\m{x}\right\|^2\right],
\end{aligned}
\end{equation}
where the inequality follows from  Lemma~\ref{lem:lips}.

From Algorithm~\ref{alg:fedout}, we have
 \begin{align}\label{eqn:update}
\m{x}_{i,0}=\m{x}, \forall i\in\mathcal{S},~~~\textnormal{and}~~~\m{x}^{+}&=\m{x}-\frac{1}{m}  \sum\limits_{i=1}^{m} \frac{\alpha}{\tau_i} \sum\limits_{k=0}^{K-1} \m{h}_i(\m{x}_{i,\nu}, \m{y}^+).
 \end{align}
Note that $\mc{F}_{0}=\mc{F}_{i,0}$ for all $i \in \mc{S}$. Hence, 
\begin{equation}
\begin{aligned}\label{eqn:cond}
&~ \mb{E}\left[ \left\|\m{y}^+\!\!-\m{y}^\star(\m{x})\right\|^2 \left\|\m{x}^+\!\!-\m{x}\right\|^2 \right]\\
%& = \mb{E}\left[\left\|\m{y}^+\!\!-\m{y}^\star(\m{x})\right\|^2 \mb{E}\left[ \left\|\m{x}^+\!\!-\m{x}\right\|^2   \mid \mc{F}_{0} \right]\right]\\
%&= \mb{E}\left[ \mb{E}\left[ \left\|\m{y}^+\!\!-\m{y}^\star(\m{x})\right\|^2 \left\|\m{x}^+\!\!-\m{x}\right\|^2 \mid \mc{F}^{+}_{0} \right]\right]\\
 &\leq  \frac{1}{m}  \sum\limits_{i=1}^{m} \frac{\alpha^2}{\tau_i} \sum\limits_{k=0}^{K-1}  \mb{E}\left[\left\|\m{y}^+\!\!-\m{y}^\star(\m{x})\right\|^2   \mb{E}\left[ \left\| \m{h}_i(\m{x}_{i,\nu}, \m{y}^+) \right\|^2 \mid\mc{F}_{i,\tau_i-1} \right] \right]\\
 & \leq \alpha^2 \tilde{D}_f^2 \mb{E}\left[\left\|\m{y}^+\!\!-\m{y}^\star(\m{x})\right\|^2 \right], 
\end{aligned}
\end{equation}
where the last inequality uses Lemma~\ref{lem:lips}.
%\ct{Nice trick. I will look closer at what $i$ should be here in the conditions? Any $i$?}
% \begin{equation}\label{eqn:cond}
% A\leq \alpha^2 \tilde{D}_f^2.
% \end{equation}

Note also that for any $\eta>0$, we have $1 \leq \frac{\eta}{2}+\frac{1}{2\eta}$. Combining this inequality with \eqref{eqn4-:dec:fedin} and using \eqref{eqn:cond} give
\begin{equation}
\label{eqn4:dec:fedin}
\begin{aligned}
% -&\mb{E}[\langle\m{y}^+\!\!-\m{y}^\star(\m{x}),  \m{y}^\star(\m{x}^+)-\m{y}^\star(\m{x})-\nabla \m{y}^\star(\m{x})(\m{x}^+\!\!-\m{x})\rangle] \leq 
-&\mb{E}[\langle\m{y}^+\!\!-\m{y}^\star(\m{x}),  \m{y}^\star(\m{x}^+)-\m{y}^\star(\m{x})-\nabla \m{y}^\star(\m{x})(\m{x}^+\!\!-\m{x})\rangle]\\
& \leq \frac{L_{\m{yx}}}{2}\mb{E}\left[\left\|\m{y}^+\!\!-\m{y}^\star(\m{x})\right\|\left\|\m{x}^+\!\!-\m{x}\right\|^2\right] \\
& \leq \frac{\eta L_{\m{yx}}}{4}\mb{E}\left[\left\|\m{y}^+\!\!-\m{y}^\star(\m{x})\right\|\left\|\m{x}^+\!\!-\m{x}\right\|^2\right] + \frac{ L_{\m{yx}}}{4\eta}\mb{E}\left[\left\|\m{x}^+\!\!-\m{x}\right\|^2\right] \\
%&\leq \frac{1}{m}  \sum\limits_{i=1}^{m} \frac{\alpha^2}{\tau_i^2} \sum\limits_{k=0}^{K-1}  \left( \mb{E}\left[\left\|\m{y}^+\!\!-\m{y}^\star(\m{x})\right\|^2   \mb{E}\left[ \left\| \m{h}_i(\m{x}_{i,\nu}, \m{y}^+) \right\|^2 \mid\mc{F}_{i,\nu} \right] \right]+ \mb{E}\left[ \mb{E}\left[ \left\| \m{h}_i(\m{x}_{i,\nu}, \m{y}^+) \right\|^2 \mid\mc{F}_{i,\nu} \right] \right]\right)\\
%&=  \frac{L_{\m{yx}}}{2} \mb{E}\left[ \left\|\m{y}^+\!\!-\m{y}^\star(\m{x})\right\|^2 \mb{E}\left[ \left\|\m{x}^+\!\!-\m{x}\right\|^2   \mid \mc{F}_{0} \right] \right] \\
%& \leq   \frac{\eta L_{\m{yx}}}{4} \mb{E}\left[ \left\|\m{y}^+\!\!-\m{y}^\star(\m{x})\right\|^2 \left\|\m{x}^+\!\!-\m{x}\right\|^2 \right] + \frac{L_{\m{yx}} \alpha^2}{4\eta}  \mb{E}\left[\left\|\frac{1}{m}\sum\limits_{i=1}^{m} \frac{1}{\tau_i} \sum\limits_{k=0}^{K-1} \bar{\m{h}}_i(\m{x}_{i,\nu},\m{y}^+)\right\|^2\right] +  \frac{L_{\m{yx}} \alpha^2}{4\eta}  \tilde{\sigma}_f\\
&\leq \frac{\eta L_{\m{yx}} \tilde{D}_f^2\alpha^2 }{4}\mb{E}\left[\left\|\m{y}^+\!\!-\m{y}^\star(\m{x})\right\|^2 \right] + \frac{L_{\m{yx}} \alpha^2}{4\eta}  \mb{E}\left[\left\|\frac{1}{m}\sum\limits_{i=1}^{m} \frac{1}{\tau_i} \sum\limits_{k=0}^{K-1} \bar{\m{h}}_i(\m{x}_{i,\nu},\m{y}^+)\right\|^2\right] +  \frac{L_{\m{yx}} \alpha^2}{4\eta}  \tilde{\sigma}_f^2,
%& \leq \frac{\eta L_{\m{yx}}\tilde{D}_f^2\alpha^2}{4}\mb{E}\left[\left\|\m{y}^+\!\!-\m{y}^\star(\m{x})\right\|^2\right]+ \frac{L_{\m{yx}} \alpha^2}{4\eta}  \mb{E}\left[\left\|\frac{1}{m}\sum\limits_{i=1}^{m} \frac{1}{\tau_i} \sum\limits_{k=0}^{K-1} \bar{\m{h}}_i(\m{x}_{i,\nu},\m{y}^+)\right\|^2\right] +  \frac{L_{\m{yx}} \alpha^2}{4\eta}  \tilde{\sigma}_f,
\end{aligned}
\end{equation}
%\ct{First inequality, there is no $1/4$ in first term. }
where  the last inequality uses \eqref{eqn:cond} and Lemma~\ref{lem:neum:bias}.

Let  $\gamma=M_f L_{\m{y}} \alpha$. Plugging \eqref{eqn4:dec:fedin} and \eqref{eqn3:dec:fedin} into \eqref{eqn2:dec:fedin}, we have
\begin{equation}
\label{eqn5:dec:fedin}
    \begin{aligned}
  \mb{E}[\langle \m{y}^{+}-\m{y}^*(\m{x}), \m{y}^*(\m{x})-\m{y}^*(\m{x}^{+})\rangle] 
    &\leq\left( 2\gamma + \frac{\eta L_{\m{yx}}\tilde{D}_f^2}{4}\alpha^2\right)\mb{E}\left[\left\|\m{y}^+\!\!-\m{y}^\star(\m{x})\right\|^2\right] \\
    &+ \left(\frac{L_{\m{y}}^2 \alpha^2}{8\gamma} +\frac{L_{\m{yx}} \alpha^2}{4\eta}\right)\mb{E}\left[\left\|\frac{1}{m}\sum\limits_{i=1}^{m} \frac{1}{\tau_i} \sum\limits_{k=0}^{K-1} \bar{\m{h}}_i(\m{x}_{i,\nu},\m{y}^+)\right\|^2\right] +  \frac{L_{\m{yx}} \alpha^2}{4\eta}  \tilde{\sigma}_f^2\\
    &= \left( 2 M_f L_{\m{y}} \alpha + \frac{\eta L_{\m{yx}}\tilde{D}_f^2}{4}\alpha^2\right)\mb{E}\left[\left\|\m{y}^+\!\!-\m{y}^\star(\m{x})\right\|^2\right]\\
     &+ \left(\frac{L_{\m{y}} \alpha}{8 M_f} +\frac{L_{\m{yx}} \alpha^2}{4\eta}\right)\mb{E}\left[\left\|\frac{1}{m}\sum\limits_{i=1}^{m} \frac{1}{\tau_i} \sum\limits_{k=0}^{K-1} \bar{\m{h}}_i(\m{x}_{i,\nu},\m{y}^+)\right\|^2\right]+  \frac{L_{\m{yx}} \alpha^2}{4\eta}  \tilde{\sigma}_f^2.
\end{aligned}
\end{equation}
%\noindent\textbf{Completing the proof of Lemma~\ref{thm:fedin}}:\\
Substituting \eqref{eqn5:dec:fedin}, \eqref{eqn1:dec:fedin}, and \eqref{eqn0:dec:fedin} into \eqref{eqn-1:dec:fedin} completes the proof.
\end{proof}

\section{Proof for Federated Bilevel Optimization}\label{sec:app:bilevel}
%Next, we provide some results that will be used frequently in our analysis.
% From Algorithm~\ref{alg:fedout}, we have 
% \begin{equation}
% \begin{aligned}
% \m{h}_{i,\nu}:= \m{h}_i(\m{x}_{i,\nu}, \m{y}^+) &= \nabla_{\m{x}} f_i(\m{x}_{i,\nu}, \m{y}^+;\xi_{i,\nu}) - \nabla_{\m{x}} f_i(\m{x}, \m{y}^+; \xi_{i,\nu})\\
% &+ \frac{1}{m}\sum_{i=1}^m\left(\nabla_{\m{x}} f_i(\m{x}, \m{y}^+; \xi_{i,\nu})-\nabla^2_{\m{xy}}g_i(\m{x},\m{y}^+;{\zeta}_{i})\m{p}_N\right),
% %\bar{\m{h}}_i (\m{x}_{i,\nu}, \m{y}^+)&:=\mb{E}\left[\m{h}_i(\m{x}_{i,\nu}, \m{y}^+; \xi_{i,\nu})|{\cal F}_{i,\nu-1}\right].
% \end{aligned}
% \label{eqn:basic:not}
% \end{equation}
%Here,
%\begin{enumerate}[leftmargin=*, topsep = 0mm]
%\item Select $ N'\in \{1, \dots, N\}$ and $\mc{S}_1, \ldots, \mc{S}_{ N'} \in \mc{S}$ uniformly at random.
%\item  Draw independent samples $\zeta^{(1)} \sim \mu^{(1)}$, $\zeta_1^{(2)}, \dots, \zeta_{(N')}^{(2)} \sim \mu^{(2)}$ %where $m_n=|\mc{S}_n|$.
%\item For each $ n \in [N']$: draw independent samples  $\zeta_n^{(2,1)}, \dots, \zeta_{n}^{(2,m_n)} \sim \mu^{(2)}$ where $m_n=|\mc{S}_n|$.
%\item Construct an estimator of $h_f$ as
% \beq \notag
%\begin{subequations}
% \begin{align}%\label{eq:grad:est} 
% \m{p}_N=\frac{1}{|\mc{S}_0|} \frac{ N}{\ell_{g,1}} \prod_{n=1}^{N'} \big (\m{I} - \frac{1}{ \ell_{g,1}  |\mc{S}_n|} \sum_{i=1}^{|\mc{S}_n|} \nabla_{\m{y}}^2 g_i(\m{x},\m{y}; \zeta_{i,n}) \big) \big( \sum_{i\in\mc{S}_0} \nabla_\m{y} f_i(\m{x}, \m{y};\xi_{i,0})\big),
% \end{align}
% where as a convention, we have set
% \begin{align*}
% \prod_{n=1}^{0} \big (\m{I} - \frac{1}{\ell_{g,1}|\mc{S}_n|}\sum_{i=1}^{|\mc{S}_n|} \nabla_{\m{y}}^2 g_i(\m{x},\m{y}; \zeta_{i,n} )\big)=:\m{I}.
% \end{align*}
% From Line~12 in  Algorithm~\ref{alg:fedout}, for each $i\in\mathcal{S}$, and $\forall  \nu \in\{0,\ldots,\tau_i-1\}$, we have 
%  \begin{align}\label{eqn00:lem:dec}
%      \m{x}_{i,\nu+1}=\m{x}_{i,\nu}- \alpha_i \m{h}_i(\m{x}_{i,\nu}, \m{y}^+).
%  \end{align}
% Now, assume $\tau_i \geq 1$ and $\alpha_i=\alpha/\tau_i, \forall i \in \mathcal{S}$. Averaging \eqref{eqn00:lem:dec} across clients and using $\m{x}_{i,0}=\m{x}, \forall i\in\mathcal{S}$, we obtain ({\color{blue} write in expectation})
% \begin{equation}
% \begin{aligned}
% \m{x}^+ &=\m{x}-\frac{1}{m} \sum\limits_{i=1}^{m} \alpha_i \sum\limits_{k=0}^{K-1} \m{h}_i(\m{x}_{i,\nu}, \m{y}^+)\\
% & = \m{x} - \frac{1}{m} \sum\limits_{i=1}^{m} \alpha_i \sum\limits_{k=0}^{K-1} \left(\nabla_{\m{x}} f_i(\m{x}_{i,\nu}, \m{y}^+;\xi_{i,\nu}) - \nabla_{\m{x}} f_i(\m{x}, \m{y}^+; \xi_{i,\nu})\right)\\
% &+ \frac{\alpha}{m}\sum_{i=1}^m\left(\nabla_{\m{x}} f_i(\m{x}, \m{y}^+; \xi_{i,\nu})-\nabla^2_{\m{xy}}g_i(\m{x},\m{y}^+;{\zeta}_{i})\m{p}_N\right), \\
% & = \frac{\alpha}{m} \sum\limits_{i=1}^{m} \frac{1}{\tau_i} \sum\limits_{k=0}^{K-1}\nabla_{\m{x}} f_i(\m{x}_{i,\nu}, \m{y}^+;\xi_{i,\nu}) - \frac{\alpha}{m}\sum_{i=1}^m\nabla^2_{\m{xy}}g_i(\m{x},\m{y}^+;{\zeta}_{i})\m{p}_N.
% \end{aligned}    
% \end{equation}
%
%

The following lemma extends \citep[Lemma 2.2]{ghadimi2018approximation} and \citep[Lemma~2]{chen2021closing} to the finite-sum problem~\eqref{fedblo:prob}. Proofs follow similarly by applying their analysis to the inner \& outer functions $(f_i, g_i)$, $\forall i \in \mc{S}$.

%We omit the proofs which are very similar to the proof of \citep[Lemma 2.2]{ghadimi2018approximation}. 
%Proof follows similarly. 
\begin{lemma}\label{lem:lips} 
Under Assumptions~\ref{assu:f} and \ref{assu:bound:var}, for all $\x_1$, $\x_2$:
\begin{subequations}\label{eqn:newlips}
%\begin{enumerate}[label={\textnormal{L\arabic*.}}]
%\item \label{item:leml1} For all $\x_1$, $\x_2$:
\begin{align}
\|\nabla f(\m{x}_1)-\nabla f(\m{x}_2)\|
&	\leq  L_f\|\m{x}_1-\m{x}_2\|, \label{eqn:newlips:b}\\
	\|\m{y}^*(\m{x}_1)-\m{y}^*(\m{x}_2)\|&\leq  L_{\m{y}}\|\m{x}_1-\m{x}_2\|, \label{eqn:newlips:c}\\
\|\nabla \m{y}^*(\m{x}_1)-\nabla \m{y}^*(\m{x}_2)\|&\leq  L_{\m{yx}}\|\m{x}_1-\m{x}_2\|. \label{eqn:newlips:d}
\end{align}
Also, for all $i \in\mc{S}$, $\nu \in \{0,\ldots, \tau_i-1\}$,  $\x_1$, $\x_2$, and $\m{y}$, we have:
\begin{align}
\|\bar{\nabla} f_i(\m{x}_1,\m{y}) - \bar{\nabla} f_i (\m{x}_1,\m{y}^*(\m{x}_1)) \|
&\leq  M_f\|\m{y}^*(\m{x}_1)-\m{y}\|, \label{eqn:newlips:a}\\
\|\bar{\nabla} f_i(\m{x}_2,\m{y}) - \bar{\nabla} f_i (\m{x}_1,\m{y}) \|
&\leq  M_f\|\m{x}_2-\m{x}_1\|, \label{eqn:newlips:aa}\\
\mb{E}\left[\|\bar{\m{h}}_i (\m{x}_{i,\nu}, \m{y})- \m{h}_i(\m{x}_{i,\nu}, \m{y})\|^2\right] &\leq \tilde\sigma_f^2, \label{eqn:newlips:e}
\\
\mb{E}\left[\|\m{h}_i(\m{x}_{i,\nu}, \m{y}^+)\|^2 |{\mc{F}}_{i,\nu-1} \right] &\leq \tilde{D}_f^2.~~~ \label{eqn:newlips:f}
\end{align}
%\end{enumerate}
\end{subequations}
% \ct{In \eqref{eqn:newlips:e} Should this be $\x_{i,\nu}$? Otherwise, not clear to me what $\bar{\m{h}}_i(\x,\y)$ is}
% \ct{Should last one be just $\y$ instead of $\y^+$}
Here, 
\begin{equation}\label{eqn:lip:condi}
\begin{aligned}
L_{\m{y}} &:=\frac{\ell_{g,1}}{\mu_g}=\mc{O}(\kappa_g),\\
L_{\m{yx}}&:=\frac{\ell_{g,2}+\ell_{g,2}L_{\m{y}}}{\mu_g} + \frac{\ell_{g,1}}{\mu_g^2} \Big(\ell_{g,2}+\ell_{g,2}L_{\m{y}}\Big)=\mc{O}(\kappa_g^3),\\
M_f &:=\ell_{f,1} + \frac{\ell_{g,1}\ell_{f,1}}{\mu_g} + \frac{\ell_{f,0}}{\mu_g}\left(\ell_{g,2}+\frac{\ell_{g,1}{\ell_{g,2}}}{\mu_g}\right)=\mc{O}(\kappa_g^2),~~~
\\
L_f&:=\ell_{f,1} + \frac{\ell_{g,1}(\ell_{f,1}+M_f)}{\mu_g} + \frac{\ell_{f,0}}{\mu_g}\left(\ell_{g,2}+\frac{\ell_{g,1}{\ell_{g,2}}}{\mu_g}\right)=\mc{O}(\kappa_g^3),\\
\tilde{\sigma}_f^2&:=\sigma_f^2 + \frac{3}{\mu_g^2}\Big((\sigma_f^2+\ell_{f,0}^2)(\sigma_{g,2}^2+2\ell_{g,1}^2)+\sigma_f^2\ell_{g,1}^2\Big),\\
\tilde{D}_f^2&:= \left(\ell_{f,0} + \frac{\ell_{g,1}}{\mu_g}\ell_{f,1} + \ell_{g,1}\ell_{f,1}\frac{1}{\mu_g}\right)^2 + \tilde\sigma_f^2=\mc{O}(\kappa_g^2),
\end{aligned}
\end{equation}
where the other constants are provided in Assumptions~\ref{assu:f} and \ref{assu:bound:var}.
\end{lemma}
%
% \begin{proof}
% \end{proof}

%
\subsection{Descent of Main Objective}

The following lemma characterizes the descent of the outer objective. 

\begin{lemma}[Descent Lemma]\label{lem:dec}
Suppose Assumptions~\ref{assum:lip:y*}--\ref{assum:heter:f} hold. %Further, assume $\alpha= $ and  $\beta= $. 
Then, Algorithm~\ref{alg:fedmsa} guarantees:
\begin{equation}\label{eqn0:lem:dec}
 \begin{aligned}
f(\m{x}_{r+1,k}^{m}) -  f(\m{x}_{r,k}^m) \leq
 &-  \frac{3 \alpha_k} {4} \left(1- 2\alpha_k L_f\right) \left\| \nabla f  (\m{x}_{r+1,k}^m) \right\|^2 \\
  &+ \frac{\alpha_k}{2} \left(2+  3\alpha_k L_f\right)  \left\| \m{h}^m_{r,k}- \nabla f (\m{x}_{r+1,k}^m, \m{Z}_{r+1,k}^m ) \right\|^2 \\
  % &  3\alpha_k^2 \left(  \left\| \m{h}^m_{r,k}- \nabla f (\m{x}_{r+1,k}^m, \m{Z}_{r+1,k}^m ) \right\|^2+ \left\| \nabla f  (\m{x}_{r+1,k}^m) \right\|^2 \right)\\
    &+ \frac{ \alpha_k L_{\m{h},\m{z}}^2 N}{2} \left(2+ 3\alpha_k L_f\right) \sum_{n=1}^N L^2_y(n) \left\|\m{z}_{r,k}^{m,n}-\m{z}_r^{n,*}\right\|^2.
\end{aligned}
\end{equation}
\end{lemma}
%
\begin{proof}
From  Algorithm~\ref{alg:fedmsa} and 
% , and
%  \begin{align}\label{eqn1:lem:dec}
%      \m{x}_{r+1}&=\m{x}_{r}- \frac{\alpha}{M} \sum\limits_{m=1}^{M}  \sum\limits_{k=0}^{K-1} \m{h}^m_{r,k}
%  \end{align}
% Now, using 
the Lipschitz property of $\nabla f$ in Lemma~\ref{lem:lips}, we have
\begin{equation} \label{eqn1:lem:dec}
    \begin{aligned}
f(\m{x}_{r+1,k}^{m}) -  f(\m{x}_{r,k}^m)
    & \leq \left\langle \m{x}_{r+1,k}^m - \m{x}_{r,k}^m, \nabla f(\m{x}_{r+1,k}^m) \right \rangle + \frac{L_f}{2} \left\|\m{h}_{r,k}^m\right\|^2.
    %\\
   % & = + \mb{E}\left[ \left\langle \frac{\alpha}{M}\sum\limits_{m=1}^{M} \sum\limits_{k=0}^{K-1} \m{h}^m(\m{x}^m_{k}, \m{y}^m_{k}, \m{z}^m_{k}) , \nabla f(\m{x}) \right\rangle \right]\\
    %&+ \frac{L_f}{2}  \mb{E}\left[ \left\| \frac{\alpha}{M}\sum\limits_{m=1}^{M} \sum\limits_{k=0}^{K-1} \m{h}^m(\m{x}^m_{k}, \m{y}^m_{k},\m{z}^m_{k})\right\|^2\right].
    \end{aligned}
%\label{eqn2:lem:dec}
\end{equation}
In the following, we bound each term on the right hand side (RHS) of~\eqref{eqn1:lem:dec}. Let 
\begin{equation}\label{eq}
\m{a}^m_{r,k}:=\m{h}^m_{r,k}- \nabla f (\m{x}_{r+1,k}^m, \m{Z}_{r+1,k}^m ) + \nabla f  (\m{x}_{r+1,k}^m, \m{Z}_{r+1,k}^m ) -\nabla f  (\m{x}_{r+1,k}^m) + \nabla f  (\m{x}_{r+1,k}^m).
\end{equation}
For the first term, we have 
%$\m{x}_{r+1,k}^m - \m{x}_{r,k}^m =  \m{h}^m_{r,k} $ w
% Not that by our Assumption, we have $ \m{h}^m (\m{x}_{r+1,k}^m, \m{Z}_{r+1,k}^m ) =  \nabla f^m (\m{x}_{r+1,k}^m, \m{Z}_{r+1,k}^m )+ \xi_{r,k}^m$. 
%For the first term, we have $\m{x}_{r+1,k}^m - \m{x}_{r,k}^m =  \m{h}^m_{r,k} + $
%Further, for the second term in RHS of \eqref{eqn3:lem:dec}, we have
\begin{equation}\label{eqn2:lem:dec}
\begin{aligned}
 \left\langle \m{x}_{r+1,k}^m - \m{x}_{r,k}^m, \nabla f(\m{x}_{r+1,k}^m) \right\rangle &= - \alpha_k \left\langle \m{a}^m_{r,k} , \nabla f  (\m{x}_{r+1,k}^m) \right\rangle \\
  &\leq  \alpha_k \left\| \m{h}^m_{r,k}- \nabla f (\m{x}_{r+1,k}^m, \m{Z}_{r+1,k}^m ) \right\|^2\\
  &+  \alpha_k \left\|\nabla f (\m{x}_{r+1,k}^m, \m{Z}_{r+1,k}^m )- \nabla f  (\m{x}_{r+1,k}^m) \right\|^2- \frac{3\alpha_k}{4} \left\| \nabla f  (\m{x}_{r+1,k}^m)\right\|^2 \\
 &=\alpha_k \left\| \m{h}^m_{r,k}- \nabla f (\m{x}_{r+1,k}^m, \m{Z}_{r+1,k}^m ) \right\|^2 \\
 &+   L_{h,z}^2 N  \alpha_k \sum_{n=1}^N L^2_z(n) \left\|\m{z}_{r,k}^{m,n} - \m{z}_{r}^{n,*}\right\|^2 -\frac{3\alpha_k}{4}  \left\| \nabla f  (\m{x}_{r+1,k}^m) \right\|^2 .
\end{aligned}
%\label{eqn5:lem:dec}
\end{equation}
% For the first term, we have
% %Further, for the second term in RHS of \eqref{eqn3:lem:dec}, we have
% \begin{equation}%\label{lemma12:eqn7}
% \begin{aligned}
%  &\left\langle \frac{\alpha}{M}\sum\limits_{m=1}^{M} \sum\limits_{k=0}^{K-1}  \m{h}^m(\m{x}^m_{k},\m{Z}^m_{k}), \m{h}(\m{x}) \right\rangle \\
%  &\geq \frac{\alpha}{MK}\sum\limits_{m=1}^{M}  \sum\limits_{k=0}^{K-1} \left\langle \m{h}^m(\m{x}^m_{k}, \m{y}^m_{k},\m{z}^m_{k}) -\m{h}(\m{x}), \m{h}(\m{x}) \right\rangle +  \alpha\left\|\nabla f(\m{x})\right\|^2 \\
%  &\leq  \frac{\alpha}{MK}\sum\limits_{m=1}^{M} \sum\limits_{k=0}^{K-1}  L_{h}\left\|\nabla f(\m{x}) \right\|   \left( L_y\left\| \m{y}^m_{k}-  \m{y}^*\right\| + L_z\left\|\m{z}^m_{k}- \m{z}^*\right\| \right) - \alpha\left\|\nabla f(\m{x})\right\|^2 \\
%  &=-\frac{3\alpha}{4}  \left\|\nabla f(\m{x}) \right\|^2 +  \frac{\alpha}{MK}\sum\limits_{m=1}^{M} \sum\limits_{k=0}^{K-1}  L_h\left(L_y\left\| \m{y}^m_{k}-  \m{y}^*\right\| + L_z\left\|\m{z}^m_{k}- \m{z}^*\right\| \right)
% \end{aligned}
% \label{eqn5:lem:dec}
% \end{equation}
% Further, we have 
% \begin{equation}
%  \begin{aligned}
%  - \mb{E}\left\langle \nabla f(\m{x}_{r+1,k}^m) , \alpha_k \xi_{r,k}^m \right\rangle \leq \frac{\alpha^2_k}{4}\mb{E}\left\| \nabla f(\m{x}_{r+1,k}^m) \right\| + \alpha^2_k \tilde{\sigma}_f^2,
%     \end{aligned}
% \label{eqn6:lem:dec}
% \end{equation}
%
Similarly, for the second term in \eqref{eqn2:lem:dec}, we have
\begin{equation}\label{eqn3:lem:dec}
\begin{aligned}
\left\|\m{x}_{r+1,k}^m - \m{x}_{r,k}^m\right\|^2  &\leq 3\alpha_k^2 \left(  \left\| \m{h}^m_{r,k}- \nabla f (\m{x}_{r+1,k}^m, \m{Z}_{r+1,k}^m ) \right\|^2+ \left\| \nabla f  (\m{x}_{r+1,k}^m) \right\|^2 \right)\\
    & +3\alpha_k^2 \left\|\nabla f (\m{x}_{r+1,k}^m, \m{Z}_{r+1,k}^m )- \nabla f  (\m{x}_{r+1,k}^m) \right\|^2\\ 
        & \leq 3\alpha_k^2\left(  \left\| \m{h}^m_{r,k}- \nabla f (\m{x}_{r+1,k}^m, \m{Z}_{r+1,k}^m ) \right\|^2+ \left\| \nabla f  (\m{x}_{r+1,k}^m) \right\|^2 \right)\\
        &+ 3\alpha_k^2 L_{\m{h},\m{z}}^2 N \sum_{n=1}^N L^2_z(n) \left\|\m{z}_{r,k}^{m,n} - \m{z}_{r}^{n,*}\right\|^2. %\!+\! 2 \sigma_0^2 \alpha_k^2.
    \end{aligned}
\end{equation}
%where the first equality follows from the law of total expectation; the second equality uses the fact that $\bar{\m{h}}_i (\m{x}^m_{k}, \m{y}^+)=\mb{E}\left[\m{h}_i(\m{x}^m_{k}, \m{y}^+)|{\cal F}_{i,\nu-1}\right]$; and the last equality is obtained from our assumption $\alpha_i=\alpha/\tau_i, \forall i \in \mathcal{S}$.
% Substituting \eqref{eqn6+:lem:dec} into \eqref{eqn5:lem:dec} yields 
% \begin{equation}
% \begin{split}
% &- \mb{E}\left[ \left\langle \frac{1}{M}\sum\limits_{m=1}^{M} \alpha_i \sum\limits_{k=0}^{K-1}  \m{h}_i(\m{x}^m_{k}, \m{y}^+) , \nabla f(\m{x}) \right\rangle \right] \\
% &\leq - \frac{\alpha}{2} \mb{E}\left[\|  \frac{1}{M}\sum\limits_{m=1}^{M} \frac{1}{\tau_i} \sum\limits_{k=0}^{K-1} \bar{\m{h}}_i(\m{x}^m_{k}, \m{y}^+)  \|^2\right]- \frac{\alpha}{2} \mb{E}\left[\| \nabla f(\m{x})\|^2\right]\\
%  & +\frac{3\alpha }{2}  \Big( b^2 +  M_f^2 \mb{E}\left[\|\m{y}^+-\m{y}^*(\m{x})\|^2\right] + \frac{ M_f^2 }{m} \sum\limits_{m=1}^{M}   \frac{1}{\tau_i} \sum\limits_{k=0}^{K-1}  \mb{E}\left[\|\m{x}^m_{k} -\m{x}\|^2\right]\Big).
% \end{split}
% \label{eqn6-:lem:dec}
% \end{equation}   

% Next, we bound the second term on the RHS of~\eqref{eqn2:lem:dec}. Observe that 
% \begin{equation}
%  \begin{aligned}
% %\mc{A}_2
% &  \mb{E}\left\langle \frac{\alpha}{MK}\sum\limits_{m=1}^{M}  \sum\limits_{k=0}^{K-1}  \m{h}^m(\m{x}^m_{k}, \m{y}^m_{k},\m{z}^m_{k}), \alpha \xi_{k}^m \right\rangle\\
% %&= \alpha^2 \mb{E}\left[  \left\|\frac{1}{M}\sum\limits_{m=1}^{M} \frac{1}{\tau_i} \sum\limits_{k=0}^{K-1} \left( \m{h}_i(\m{x}^m_{k}, \m{y}^+)-  \bar{\m{h}}_i(\m{x}^m_{k}, \m{y}^+) + \bar{\m{h}}_i(\m{x}^m_{k}, \m{y}^+) \right) \right\| \right]\\
%  &\geq -\frac{\alpha^2}{4}\mb{E}\left\| \frac{1}{MK}\sum\limits_{m=1}^{M}  \sum\limits_{k=0}^{K-1} \m{h}^m(\m{x}^m_{k}, \m{y}^m_{k},\m{z}^m_{k})\right\| - \alpha^2 \tilde{\sigma}_f^2,
%     \end{aligned}
% \label{eqn6:lem:dec}
% \end{equation}
% where the inequality follows from Lemmas~\ref{lem:rand:zer} and \ref{lem:lips}. %\ct{Seems there is a missing square in $\tilde{\sigma}_f$}

Plugging \eqref{eqn3:lem:dec} and \eqref{eqn2:lem:dec} into \eqref{eqn1:lem:dec} completes the proof.
\end{proof}



%\subsection{Proof of Theorem~\ref{thm:fednest}}


\subsection{Drifting Errors  }

\begin{lemma}[Drifting Error I]\label{lem:drift:fedmsa}
Suppose Assumptions~ \ref{assum:lip:y*}--\ref{assum:stmonot:g} hold. Further, assume $K \geq 1$ and $ \alpha^{m}_k\leq 1/(5M_fK), \forall m \in \mathcal{S}$. Then, for each $m \in \mathcal{S}$ and $\forall k \in\{0,\ldots, K-1\}$,  Algorithm~\ref{alg:fedmsa} guarantees:
%
\begin{align}\label{eqn1:lem:drift:fedmsa}
\nonumber
 \mb{E}\left\|\m{x}^{m}_{r+1,k}-\m{x}_r\right\|^2           & \leq  3 \exp(1)\alpha_k^2 (1+K) \sum\limits_{k=1}^{K-1}  L_{\m{h},\m{z}}^2 N \sum_{n=1}^N L^2_z(n)\|\m{z}_{r+1,k}^{m,n}-\m{z}^{n,*}\|^2
        \\
        \nonumber
       &+ 3 \exp(1)\alpha_k^2 (1+K) \sum\limits_{k=1}^{K-1}  \left\| \m{h}^m_{r,k}- \nabla f (\m{x}_{r+1,k}^m, \m{Z}_{r+1,k}^m) \right\|^2\\
       &+ 3 \exp(1) \alpha_k^2 (1+K) \sum\limits_{k=1}^{K-1} \left\| \nabla f  (\m{x}_{r+1,k}^m) \right\|^2.
%  \leq 9  \tau_i \alpha_i^2 \left( 4\tau_i  \left( M_f^2 \mb{E}\left[\|\m{y}^+-\m{y}^\star(\m{x})\|^2\right]+  \mb{E}\left[\|\nabla f(\m{x})\|^2\right]+ 3  b^2\right) + 3 \tilde{\sigma}_f^2 \right).\\
 %&\leq 2 e \left(\mb{E} \left\| \m{v}_r- \nabla f(\m{x}_r)\right\|^2 + \sum_{n=1}^N\mb{E} \left\|\m{z}_k^n-\m{z}^{n,*}(\m{z}_k^{n-1})\right\|^2  \right)+  \frac{1}{6K} \sum_{k=1}^K \left\| \nabla f(\m{x}_{r+1,k}^m)\right\| 
%   36 \tau_i^2 \alpha_i^2 \left(M_f^2 \mb{E}\left[\|\m{y}^+-\m{y}^\star(\m{x})\|^2\right]+  \mb{E}\left[\|\nabla f(\m{x})\|^2\right]+ 3 b^2\right) \\
%  &+ 27 \tau_i \alpha_i^2  \tilde{\sigma}_f^2.
\end{align}
\end{lemma}
\begin{proof}
From  Algorithm~\ref{alg:fedmsa} that $\forall m\in\mathcal{S}$,
\begin{equation}
\label{eqn2:lem:drift:fedmsa}
\begin{aligned}
\left\|\m{x}_{r+1,k}^m-\m{x}_r-\alpha_k \m{h}_{r,k-1}^m \right\|^2 &\leq  \left(1+\frac{1}{K}\right)\|\m{x}_{r+1,k-1}^m-\m{x}_r\|^2+ (K+1)\alpha_k^2 \left\|\m{h}_{r,k-1}^m\right\|^2\\
%&\leq  \left(1+\frac{1}{K}\right)\|\m{x}_{r+1,k}^m-\m{x}_r\|^2\\
%&+ 3 \alpha_k^2 (1+K) \left\|\nabla f (\m{x}_{r+1,k}^m, \m{Z}_{r+1,k}^m )- \nabla f  (\m{x}_{r+1,k}^m) \right\|^2\\ 
        & \leq  \left(1+\frac{1}{K}\right)\|\m{x}_{r+1,k-1}^m-\m{x}_r\|^2 + 3\alpha_k^2 (1+K)  L_{\m{h},\m{z}}^2 N \sum_{n=1}^N L^2_z(n)\|\m{z}_{r+1,k-1}^{m,n}-\m{z}_{r}^{n,*}\|^2
        \\
       &+ 3\alpha_k^2 (1+K)  \left(  \left\| \m{h}^m_{r,k-1}- \nabla f (\m{x}_{r+1,k-1}^m, \m{Z}_{r+1,k-1}^m ) \right\|^2+ \left\| \nabla f (\m{x}_{r+1,k-1}^m) \right\|^2 \right).
% \left\| \right\|^2\\ 
%         & \leq 3\alpha_k^2\left(  \left\| \m{h}^m_{r,k}- \nabla f (\m{x}_{r+1,k}^m, \m{Z}_{r+1,k}^m ) \right\|^2+ \left\| \nabla f  (\m{x}_{r+1,k}^m) \right\|^2 \right)\\
%         &+ 3\alpha_k^2 L_{\m{h},\m{z}}^2 N \sum_{n=1}^N L^2_y(n)\|\m{z}_k^n-\m{z}_k^{n,*}\|^2.
% \left(\mb{E}\left\|\m{z}_{r,k}^m\right\|^2 + \mb{E}\left\| \m{v}_{r,k}^m \right\|^2 \right)\\
% %2\tau_i \mb{E}\Big[\|\alpha_i (\m{v}_{r,k}^m+\m{z}_{r,k}^m)\|^2\Big]\\
%  &\leq  \left(1+\frac{1}{K}\right)\mb{E}\left[\|\m{x}_{r+1,k}^m-\m{x}\|^2\right]+ 4\tau_i \alpha_i^2  \left(\mb{E}\left[\| \m{z}_{r,k}^m\|^2\right] + 9  b^2\right)\\
%      % &\leq  (1+\frac{1}{K})\mb{E}\Big[\|\m{x}_{r+1,k}^m-\m{x}\|^2\Big]+ 2\tau_i \mb{E}\Big[\|\alpha_i( \bar{\nabla} f_i(\m{x}_{r+1,k}^m, \m{y})-\bar{\nabla} f_i(\m{x},\m{y}))-\alpha_i \bar{\nabla} f(\m{x},\m{y})\|^2\Big] +\\
% %       &\leq  (1+\frac{1}{K})\mb{E}\Big[\|\m{x}_{r+1,k}^m-\m{x}\|^2\Big]+ 10 \tau_i \alpha_i^2M_f^2\mb{E}\Big[\|\m{x}_{r+1,k}^m-\m{x}\|\Big]+ 10\tau_i \alpha_i^2  \mb{E}\Big[\|\bar{\nabla} f(\m{x},\m{y})\|^2\Big] + 10b^2  \\
%       &\leq  \left(1+\frac{1}{K}+12\tau_i \alpha_i^2 M_f^2\right)\mb{E}\left[\|\m{x}_{r+1,k}^m-\m{x}\|^2\right]\\
%       &+ 12\tau_i \alpha_i^2 \left( M_f^2 \mb{E}\left[\|\m{y}^+-\m{y}^\star(\m{x})\|^2\right]+  \mb{E}\left[\|\nabla f(\m{x})\|^2\right]+ 3 b^2\right).
    \end{aligned}
\end{equation}
where the last inequality uses \eqref{eqn3:lem:dec}.

Now, iterating equation \eqref{eqn2:lem:drift:fedmsa} and using $  (\m{x}^{m}_{r+1,1},\m{Z}^{m}_{r+1,1})=(\m{x}^{m}_{r+1,0},\m{Z}^{m}_{r+1,0})= (\m{x}_r,\m{Z}_r), ~~\forall m\in [M]$, we obtain
\begin{equation}
\label{eqn3:lem:drift:fedmsa}
\begin{aligned}
\left\|\m{x}_{r+1,k}^m-\m{x}_r-\alpha_k \m{h}_{r,k-1}^m \right\|^2 
% leq  \left(1+\frac{1}{K}\right)\|\m{x}_{r+1,k-1}^m-\m{x}_r\|^2+ (K+1)\alpha_k^2 \left\|\m{v}_{r,k-1}^m\right\|^2\\
%&\leq  \left(1+\frac{1}{K}\right)\|\m{x}_{r+1,k}^m-\m{x}_r\|^2\\
%&+ 3 \alpha_k^2 (1+K) \left\|\nabla f (\m{x}_{r+1,k}^m, \m{Z}_{r+1,k}^m )- \nabla f  (\m{x}_{r+1,k}^m) \right\|^2\\ 
        & \leq  3\alpha_k^2 (1+K) \sum\limits_{j=2}^{k} \left(1+\frac{1}{K+1}\right)^j  L_{\m{h},\m{z}}^2 N \sum_{n=1}^N L^2_z(n)\|\m{z}_{r+1,j-1}^{m,n}-\m{z}^{n,*}\|^2
        \\
       &+ 3\alpha_k^2 (1+K) \sum\limits_{j=2}^{k} \left(1+\frac{1}{K+1}\right)^j  \left\| \m{h}^m_{r,j-1}- \nabla f (\m{x}_{r+1,j-1}^m, \m{Z}_{r+1,j-1}^m) \right\|^2\\
       &+ 3\alpha_k^2 (1+K) \sum\limits_{j=2}^{k} \left(1+\frac{1}{K+1}\right)^j \left\| \nabla f  (\m{x}_{r+1,j-1}^m) \right\|^2. 
\end{aligned}
\end{equation}
Since $\sum\limits_{j=2}^{k} \left(1+\frac{1}{K+1}\right)^j \leq  \exp(1)$. We have 
\begin{equation}
\label{eqn4:lem:drift:fedmsa}
\begin{aligned}
\left\|\m{x}_{r+1,k}^m-\m{x}_r-\alpha_k \m{h}_{r,k-1}^m \right\|^2 
% leq  \left(1+\frac{1}{K}\right)\|\m{x}_{r+1,k-1}^m-\m{x}_r\|^2+ (K+1)\alpha_k^2 \left\|\m{v}_{r,k-1}^m\right\|^2\\
%&\leq  \left(1+\frac{1}{K}\right)\|\m{x}_{r+1,k}^m-\m{x}_r\|^2\\
%&+ 3 \alpha_k^2 (1+K) \left\|\nabla f (\m{x}_{r+1,k}^m, \m{Z}_{r+1,k}^m )- \nabla f  (\m{x}_{r+1,k}^m) \right\|^2\\ 
  & \leq  3 \exp(1) \alpha_k^2 (1+K) \sum\limits_{k=2}^{K}  L_{\m{h},\m{z}}^2 N \sum_{n=1}^N L^2_z(n)\|\m{z}_{r+1,k-1}^{m,n}-\m{z}^{n,*}\|^2
        \\
       &+ 3 \exp(1)\alpha_k^2 (1+K) \sum\limits_{k=2}^{K}  \left\| \m{h}^m_{r,k-1}- \nabla f (\m{x}_{r+1,k-1}^m, \m{Z}_{r+1,k-1}^m) \right\|^2\\
       &+ 3 \exp(1) \alpha_k^2 (1+K) \sum\limits_{k=2}^{K} \left\| \nabla f  (\m{x}_{r+1,k-1}^m) \right\|^2 \\
         & \leq  3 \exp(1)\alpha_k^2 (1+K) \sum\limits_{k=1}^{K-1}  L_{\m{h},\m{z}}^2 N \sum_{n=1}^N L^2_z(n)\|\m{z}_{r+1,k}^{m,n}-\m{z}^{n,*}\|^2
        \\
       &+ 3 \exp(1)\alpha_k^2 (1+K) \sum\limits_{k=1}^{K-1}  \left\| \m{h}^m_{r,k}- \nabla f (\m{x}_{r+1,k}^m, \m{Z}_{r+1,k}^m) \right\|^2\\
       &+ 3 \exp(1) \alpha_k^2 (1+K) \sum\limits_{k=1}^{K-1} \left\| \nabla f  (\m{x}_{r+1,k}^m) \right\|^2.
\end{aligned}
\end{equation}


% Here, the first inequality follows from Lemma~\ref{lem:trig}; the second inequality uses Lemma~\ref{lem:Jens}; and the third and last inequalities follow from \eqref{eqn3a:lemm:drift} and \eqref{eqn3c:lemm:drift}.

% \begin{subequations}
% \begin{equation}
% \label{eqn3c:lemm:drift}
% \begin{aligned}
% \mb{E}\left\|\m{a}^{r,k}\right\|^2 & \leq  \left(1+\frac{1}{K}\right)\mb{E}\left[\|\m{v}_{r+1,k-1}^m- \nabla f (\m{x}_{r+1, k-1}^m)\|^2\right] \\
% &+ \left(K+1\right)\mb{E}\left\|  \nabla f^m(\m{x}^{m}_{r,k}, \m{Z}_{r,k})-\nabla f^m(\m{x}^{m}_{r,k-1}, \m{Z}_{r,k-1})+ \nabla f(\m{x}^{m}_{r,k-1}, \m{Z}_{r,k-1})-\nabla f(\m{x}^{m}_{r,k}, \m{Z}_{r,k})\right\|^2 \\
% %&+\left\| \nabla f(\m{x}^{m}_{r,k-1}, \m{Z}_{r,k-1}) - \nabla f(\m{x})\right\|^2+ \left\| \nabla f(\m{x}^{m}_{r,k}, \m{Z}_{r,k}) - \nabla f(\m{x})\right\|^2\\
% & \leq  \exp (3) \mb{E} \left\|\m{v}_{r,0}^m- \nabla f (\m{x}_{r+1, 0}^m)\right\|^2 +\exp(3) \tau_1  \left(K+1\right) \mb{E}\left\| (\m{x}^{m}_{r,k}, \m{Z}_{r,k}^m)-(\m{x}^{m}_{r,k-1}, \m{Z}_{r,k-1}^m)\right\|^2 \\
% \end{aligned}
% \end{equation}
% \end{subequations}
% where the last inequality uses Assumption~\ref{assum:heter:f}.



%%%%
Now, we bound  the local gradient estimation error. Let
\begin{equation}\label{eqn5:lem:drift:fedmsa}
\begin{aligned}
%\m{a}_{i,\nu}&:= \bar{\m{h}}_i(\m{x}_{i,\nu}, \m{y}^+)- \bar{\nabla} f_i(\m{x}_{i,\nu}, \m{y}^+)- \bar{\m{h}}_i(\m{x},\m{y}^+) \\
%& +\bar{\nabla} f_i(\m{x}, \m{y}^+) +\bar{\m{h}}(\m{x},\m{y}^+) -\bar{\nabla} f(\m{x}, \m{y}^+),\\
\m{a}_{r,k}^m &:= \m{h}^m_{r,k-1} - \nabla f (\m{x}_{r+1,k-1}^m, \m{Z}_{r+1,k-1}^m)\\
 & + \nabla f^m(\m{x}_{r+1,k}^m, \m{Z}_{r+1,k}^m) - \nabla f  (\m{x}_{r+1,k}^m, \m{Z}_{r+1,k}^m ) -\nabla f^m  (\m{x}_{r+1,k-1}^m,  \m{Z}_{r+1,k-1}^m) + \nabla f  (\m{x}_{r+1,k-1}^m,\m{Z}_{r+1,k-1}^m)\\
\m{b}^{m}_{r,k}&:=\m{h}^m(\m{x}^{m}_{r+1,k}, \m{Z}_{r+1,k}^m)- \nabla f^m(\m{x}^{m}_{r+1,k}, \m{Z}_{r+1,k}^m) \\
&+\m{h}^m(\m{x}^{m}_{r+1,k-1}, \m{Z}_{r+1,k-1}^m)-  \nabla f^m(\m{x}^{m}_{r+1,k}, \m{Z}_{r+1,k-1}^m).\\
%\m{a}^{m}_{r,k}&:= \m{v}_{r,k-1}^m+ \nabla f^m(\m{x}^{m}_{r,k}, \m{Z}_{r,k})-\nabla f^m(\m{x}^{m}_{r,k}, \m{Z}_{r,k})+ \nabla f(\m{x}^{m}_{r,k-1}, \m{Z}_{r,k-1}) - \nabla f(\m{x}_r) + \nabla  f(\m{x}_r).
\end{aligned}
\end{equation}
%Recall the definition of  
One will notice that  $\m{a}^{m}_{r,k} +  \m{b}^{m}_{r,k} =  \m{v}_{r,k-1}^m$. 
% Hence, from Algorithm~\ref{alg:fedmsa}, for each $m\in\mathcal{S}$, we have
% \begin{equation*}
% \begin{aligned}
%      \m{x}^{m}_{r+1,k}-\m{x}_r &=\m{x}^{m}_{r+1,k}-\m{x}_r-\alpha_k \left(\m{a}^{m}_{r,k} +  \m{b}^{m}_{r,k}\right),
%     \end{aligned}
% \end{equation*}
% which implies that 
% \begin{equation}\label{eqn3:lemm:drift:fedmsa}
% \begin{aligned}
% \mb{E}\left[\|\m{x}^{m}_{r+1,k}-\m{x}_r\|^2\right]
% &=\mb{E}\left[\|\m{x}^{m}_{r+1,k}-\m{x}_r-\alpha_k \m{a}^{m}_{r,k} \|^2\right]+\alpha_k^2\mb{E}\left[\| \m{b}^{m}_{r,k}\|^2\right]\\&-2\mb{E}\left[\mb{E}\left[\langle \m{x}^{m}_{r,k}-\m{x}_{r}-\alpha_k \m{a}^{m}_{r,k},\alpha_k \m{b}_{r,k} \rangle\mid\mathcal{F}_{r,k}^m\right]\right] \\ 
% &= \mb{E}\left[\|\m{x}^{m}_{r+1,k}-\m{x}_r-\alpha_k \m{a}_{r,k}\|^2\right]+\alpha_k^2\mb{E}\left[\|\m{b}_{r,k}^m\|^2\right].
% \end{aligned}
% \end{equation}
% Here, the last equality uses Lemma~\ref{lem:rand:zer} since  $\mb{E}[\m{b}_{r,k}^m|\mathcal{F}_{r,k}^m]=0$, {by definition}.
\begin{equation}\label{eqn6:lem:drift:fedmsa}
\begin{aligned}
\mb{E}\left\|\m{h}^m_{r,k}-\nabla f (\m{x}_{r+1,k}^m, \m{Z}_{r+1,k}^m )\right\|^2
% &=\m{h}^m_{r,k-1} - \nabla f (\m{x}_{r+1,k-1}^m, \m{Z}_{r+1,k-1}^m )\\
% &+ \m{h}^m(\m{x}^{m}_{r+1,k}, \m{Z}_{r+1,k}^m)- \nabla f^m(\m{x}^{m}_{r+1,k}, \m{Z}_{r+1,k}^m) +\m{h}^m(\m{x}^{m}_{r+1,k-1}, \m{Z}_{r+1,k-1}^m)-  \nabla f^m(\m{x}^{m}_{r+1,k-}, \m{Z}_{r+1,k-1}^m)  \\
% & + \nabla f^m(\m{x}_{r+1,k}^m, \m{Z}_{r+1,k}^m) - \nabla f  (\m{x}_{r+1,k}^m, \m{Z}_{r+1,k}^m ) -\nabla f^m  (\m{x}_{r+1,k-1}^m,  \m{Z}_{r+1,k-1}^m) + \nabla f  (\m{x}_{r+1,k-1}^m,\m{Z}_{r+1,k-1}^m)\\
&= \mb{E}\left\|\m{a}^{m}_{r,k} +  \m{b}^{m}_{r,k}\right\|^2\\
&= \mb{E}\left\|\m{a}^{m}_{r,k} \right\|^2+  \mb{E}\left\| \m{b}^{m}_{r,k}\right\|^2.
% &=\m{h}^m_{r,k-1} - \nabla f (\m{x}_{r+1,k-1}^m, \m{Z}_{r+1,k-1}^m )\\
% &+ \left\|\m{h}^m(\m{x}^{m}_{r+1,k}, \m{Z}_{r+1,k}^m)- \nabla f^m(\m{x}^{m}_{r+1,k}, \m{Z}_{r+1,k}^m) +\m{h}^m(\m{x}^{m}_{r+1,k-1}, \m{Z}_{r+1,k-1}^m)-  \nabla f^m(\m{x}^{m}_{r+1,k-}, \m{Z}_{r+1,k-1}^m)\right\|  \\
% & + \nabla f^m(\m{x}_{r+1,k}^m, \m{Z}_{r+1,k}^m) - \nabla f  (\m{x}_{r+1,k}^m, \m{Z}_{r+1,k}^m ) -\nabla f^m  (\m{x}_{r+1,k-1}^m,  \m{Z}_{r+1,k-1}^m) + \nabla f  (\m{x}_{r+1,k-1}^m,\m{Z}_{r+1,k-1}^m)
    \end{aligned}
\end{equation}
Here, the last equality uses Lemma~\ref{lem:rand:zer} since  $\mb{E}[\m{b}_{r,k}^m|\mathcal{F}_{r,k}^m]=0$, {by definition}.

%From Lemmas~\ref{lem:Jens}, \ref{lem:neum:bias}, and \ref{lem:lips},  for $\m{a}_{r,k}^m$ and $\m{b}_{r,k}^m$ defined in \eqref{eqn2:lem:drift:fedmsa},
From Assumption~\ref{assum:bias}, we have 
\begin{subequations}
\label{eqn7:lem:drift:fedmsa}
\begin{align}
\left\|\m{b}_{r,k}^m \right\|^2 &\leq  \frac{M_f^2}{b} \left\|\m{x}^{m}_{r+1,k}-\m{x}^{m}_{r+1,k-1}\right\|^2.
    \end{align}
Further, 
\begin{equation}
\begin{aligned}
\left\|\m{a}_{r,k}^m \right\|^2 &\leq  \left(1+ \frac{1}{K}\right) \left\|\m{h}^m_{r,k-1} - \nabla f (\m{x}_{r+1,k-1}^m, \m{Z}_{r+1,k-1}^m)\right\|^2\\
 & + \left(1+K\right) \big\|\nabla f^m(\m{x}_{r+1,k}^m, \m{Z}_{r+1,k}^m) - \nabla f  (\m{x}_{r+1,k}^m, \m{Z}_{r+1,k}^m ) \\
 &-\nabla f^m  (\m{x}_{r+1,k-1}^m,  \m{Z}_{r+1,k-1}^m) + \nabla f  (\m{x}_{r+1,k-1}^m,\m{Z}_{r+1,k-1}^m)\big\|^2\\
 &  \leq  \left(1+ \frac{1}{K}\right) \left\|\m{h}^m_{r,k-1} - \nabla f (\m{x}_{r+1,k-1}^m, \m{Z}_{r+1,k-1}^m)\right\|^2\\
 & +2 \tau^2 \left(1+K\right)  \left\|(\m{x}^{m}_{r+1,k}, \m{Z}_{r+1,k}^m)-(\m{x}^{m}_{r+1,k-1},\m{Z}_{r+1,k-1}^m)\right\|^2.
%\m{b}^{m}_{r,k}&:=\m{h}^m(\m{x}^{m}_{r+1,k}, \m{Z}_{r+1,k}^m)- \nabla f^m(\m{x}^{m}_{r+1,k}, \m{Z}_{r+1,k}^m) 
    \end{aligned}
\end{equation}
\end{subequations}
Now, iterating equation \eqref{eqn7:lem:drift:fedmsa} and using $  \m{h}^{m}_{r+1,0}=\m{h}_{r}, ~~\forall m\in [M]$, we obtain
\begin{equation}\label{eqn6:lem:drift:fedmsa}
\begin{aligned}
&~~~~~~\mb{E}\left\|\m{h}^m_{r,k}-  \nabla f (\m{x}_{r+1,k}^m, \m{Z}_{r+1,k}^m )\right\|^2
% &=\m{h}^m_{r,k-1} - \nabla f (\m{x}_{r+1,k-1}^m, \m{Z}_{r+1,k-1}^m )\\
% &+ \m{h}^m(\m{x}^{m}_{r+1,k}, \m{Z}_{r+1,k}^m)- \nabla f^m(\m{x}^{m}_{r+1,k}, \m{Z}_{r+1,k}^m) +\m{h}^m(\m{x}^{m}_{r+1,k-1}, \m{Z}_{r+1,k-1}^m)-  \nabla f^m(\m{x}^{m}_{r+1,k-}, \m{Z}_{r+1,k-1}^m)  \\
% & + \nabla f^m(\m{x}_{r+1,k}^m, \m{Z}_{r+1,k}^m) - \nabla f  (\m{x}_{r+1,k}^m, \m{Z}_{r+1,k}^m ) -\nabla f^m  (\m{x}_{r+1,k-1}^m,  \m{Z}_{r+1,k-1}^m) + \nabla f  (\m{x}_{r+1,k-1}^m,\m{Z}_{r+1,k-1}^m)\\
\\
&= \exp(1) \mb{E} \left\|\m{h}^m_{r,0}-  \nabla f (\m{x}_{r+1,0}^m, \m{Z}_{r+1,0}^m )\right\|^2 \\
%&+    \frac{  \exp(1) M_f^2}{b} \left\|\m{x}^{m}_{r+1,k}-\m{x}^{m}_{r+1,k-1}\right\|^2\\
&+\left( \frac{  \exp(1) M_f^2}{b}+2 \tau^2 \left(1+K\right) \right) \sum_{k=1}^K \mb{E}  \left\|(\m{x}^{m}_{r+1,k}, \m{Z}_{r+1,k}^m)-(\m{x}^{m}_{r+1,k-1},\m{Z}_{r+1,k-1}^m)\right\|^2.\\
& \leq \exp(1) \mb{E} \left\|\m{h}^m_{r,0}-  \nabla f (\m{x}_{r+1,0}^m, \m{Z}_{r+1,0}^m )\right\|^2 \\
%&+    \frac{  \exp(1) M_f^2}{b} \left\|\m{x}^{m}_{r+1,k}-\m{x}^{m}_{r+1,k-1}\right\|^2\\
&+\left( \frac{  \exp(1) M_f^2}{b}+2 \tau^2 \left(1+K\right) \right) \sum_{k=1}^K \mb{E} \left\|(\m{x}^{m}_{r+1,k}, \m{Z}_{r+1,k}^m)-(\m{x}^{m}_{r+1,k-1},\m{Z}_{r+1,k-1}^m)\right\|^2.\\
% &=\m{h}^m_{r,k-1} - \nabla f (\m{x}_{r+1,k-1}^m, \m{Z}_{r+1,k-1}^m )\\
% &+ \left\|\m{h}^m(\m{x}^{m}_{r+1,k}, \m{Z}_{r+1,k}^m)- \nabla f^m(\m{x}^{m}_{r+1,k}, \m{Z}_{r+1,k}^m) +\m{h}^m(\m{x}^{m}_{r+1,k-1}, \m{Z}_{r+1,k-1}^m)-  \nabla f^m(\m{x}^{m}_{r+1,k-}, \m{Z}_{r+1,k-1}^m)\right\|  \\
% & + \nabla f^m(\m{x}_{r+1,k}^m, \m{Z}_{r+1,k}^m) - \nabla f  (\m{x}_{r+1,k}^m, \m{Z}_{r+1,k}^m ) -\nabla f^m  (\m{x}_{r+1,k-1}^m,  \m{Z}_{r+1,k-1}^m) + \nabla f  (\m{x}_{r+1,k-1}^m,\m{Z}_{r+1,k-1}^m)
 \end{aligned}
\end{equation}
%where the last inequality uses Lemma~\ref{lem:lips}.
\end{proof}

\begin{lemma}[Local Momentum Bound]\label{lem:drift:fedmsa}
Suppose Assumptions~ \ref{assum:lip:y*}--\ref{assum:stmonot:g} hold. Further, assume $K \geq 1$ and $ \alpha^{m}_k\leq 1/(5M_fK), \forall m \in \mathcal{S}$. Then,  Algorithm~\ref{alg:fedmsa} guarantees:
%
\begin{align}\label{eqn1:lem:drift:fedmsa}
\nonumber
\frac{1}{K} \sum_{r=0}^{R-1} \mb{E} \left\| \m{h}_r- \nabla f(\m{x}_r)\right\|^2  \leq  \frac{1}{24 e KR } \sum_{r=0}^{R-1} \sum_{k=0}^{K-1}  \mb{E} \left\| \nabla f (\m{x}_{r+1,k}^m)\right\|+  \frac{48 e \sigma^2  \rho}{ MKb}  +  \frac{24 e \sigma^2 }{\ \rho MKb_0},
%+ \sum_{n=1}^N\mb{E} \left\|\m{z}_k^n-\m{z}^{n,*}(\m{z}_k^{n-1})\right\|^2  \right)+  \frac{1}{6K} \sum_{k=1}^K \left\| \nabla f(\m{x}_{r+1,k}^m)\right\| 
%   36 \tau_i^2 \alpha_i^2 \left(M_f^2 \mb{E}\left[\|\m{y}^+-\m{y}^\star(\m{x})\|^2\right]+  \mb{E}\left[\|\nabla f(\m{x})\|^2\right]+ 3 b^2\right) \\
%  &+ 27 \tau_i \alpha_i^2  \tilde{\sigma}_f^2.
\end{align}
where $\rho$ is the momentum parameter.
\end{lemma}
\begin{proof}
It follows from Algorithm~\ref{alg:fedmsa} that 
 \begin{equation}
  \m{h}^m_r = \m{h}^{m} \left(\m{x}_r,\m{Z}_r\right)+(1-\rho)\left(\m{h}_{r-1}-\m{h}^{m}\left(\m{x}_{r-1},\m{Z}_{r-1}\right)\right)     
 \end{equation} 
which implies that 
\begin{align}
\nonumber
 \m{h}_r- \nabla f(\m{x}_r)
 &=  (1 -\rho)  \left(\m{h}_{r-1}- \nabla f(\m{x}_{r-1})\right) + \rho \left( \frac{1}{M}\sum_{m=1}^M \m{h}^{m} \left(\m{x}_r,\m{Z}_r\right) - \nabla f(\m{x}_r)\right)\\
 &+(1-\rho)\left(  \frac{1}{M}\sum_{m=1}^M \m{h}^{m} \left(\m{x}_r,\m{Z}_r\right) -\frac{1}{M}\sum_{m=1}^M \m{h}^{m}\left(\m{x}_{r-1},\m{Z}_{r-1}\right) +  \nabla f (\m{x}_{r-1} ) +  \nabla f (\m{x}_{r} ) \right)    
\end{align}
Then, we consider 
\begin{align*}
\nonumber
\mb{E}_r\left\|\m{h}_r- \nabla f(\m{x}_r, \m{Z}_r)\right\|
 &=  (1 -\rho)^2  \left\|\m{h}_{r-1}- \nabla f(\m{x}_{r-1}, \m{Z}_r)\right\| \\
 &+ 2\rho^2 \left\| \frac{1}{M}\sum_{m=1}^M \m{h}^{m} \left(\m{x}_r,\m{Z}_r\right) - \frac{1}{M}\sum_{m=1}^M \nabla f^{m} \left(\m{x}_r,\m{Z}_r\right) \right\|\\
 \nonumber 
 &+2(1-\rho)\left\|  \frac{1}{M}\sum_{m=1}^M \m{h}^{m} \left(\m{x}_r,\m{Z}_r\right) - \nabla f \left(\m{x}_{r}, \m{Z}_r \right)\right\|^2\\
 & + 2(1-\rho) \left\|\frac{1}{M}\sum_{m=1}^M \m{h}^{m}\left(\m{x}_{r-1},\m{Z}_{r-1}\right) - \nabla f (\m{x}_{r}, \m{Z}_{r} ) \right\|^2\\
 & \leq  (1 -\rho)^2  \left\|\m{h}_{r-1}- \nabla f(\m{x}_{r-1})\right\| + 2 \rho^2 \frac{\sigma^2}{MKb}
 \\
 &+ 2(1-\rho)^2 \frac{M_f}{MKb} \left\| \left(\m{x}_r,\m{Z}_r\right) - \left(\m{x}_{r-1},\m{Z}_{r-1}\right) \right\|^2
 %&+2(1-\rho)\left(  \frac{1}{M}\sum_{m=1}^M \m{h}^{m} \left(\m{x}_r,\m{Z}_r\right) -\frac{1}{M}\sum_{m=1}^M \m{h}^{m}\left(\m{x}_{r-1},\m{Z}_{r-1}\right) +  \nabla f (\m{x}_{r-1} ) +  \nabla f (\m{x}_{r} ) \right) 
\end{align*}
Hence,
\begin{align*}
\nonumber
\rho \sum_{r=0}^{R-1}\mb{E}\left\|\m{h}_r- \nabla f(\m{x}_r, \m{Z}_r)\right\|
 &=   \sum_{r=0}^{R-1}\mb{E}\left\|\m{h}_r- \nabla f(\m{x}_r, \m{Z}_r)\right\|-(1-\rho) \sum_{r=0}^{R-1} \left\|\m{h}_{r-1}- \nabla f(\m{x}_{r-1}, \m{Z}_r)\right\| \\
%  &+ \left\|\m{h}_{R}- \nabla f(\m{x}_{R}, \m{Z}_R)\right\|  +\left\|\m{h}_{0}- \nabla f(\m{x}_0, \m{Z}_0)\right\|   \\
% \nonumber 
 &=+ \sum_{r=1}^{R}\mb{E}\left\|\m{h}_r- \nabla f(\m{x}_r, \m{Z}_r)\right\|-(1-\rho) \sum_{r=0}^{R-1} \left\|\m{h}_{r-1}- \nabla f(\m{x}_{r-1}, \m{Z}_r)\right\| \\
&~~ - \left\|\m{h}_{R}- \nabla f(\m{x}_{R}, \m{Z}_R)\right\|  +\left\|\m{h}_{0}- \nabla f(\m{x}_0, \m{Z}_0)\right\|  \\
 &= 2(1-\rho)^2 \frac{M_f^2}{ MKb} \sum_{r=0}^{R-1}\mb{E} \left\| \left(\m{x}_r,\m{Z}_r\right) - \left(\m{x}_{r-1},\m{Z}_{r-1}\right) \right\|\\
& + 2\rho^2 R \frac{\sigma^2}{MKb} + \mb{E}\left\|\m{h}_{0}- \nabla f(\m{x}_0, \m{Z}_0)\right\|.
\end{align*}
Here, the last inequality follows from
$$
\mb{E}\left\|\m{h}_{0}- \nabla f(\m{x}_0, \m{Z}_0)\right\| = \mb{E}\left\|  \frac{1}{M}\sum_{m=1}^M\nabla f^m(\m{x}_{0}, \m{Z}_{0})-\nabla f(\m{x}_{0}, \m{Z}_{0})\right\|^2 \leq \frac{\sigma^2}{ Mb_0}.
$$
Hence, we
\begin{align}
\nonumber 
\sum_{r=0}^{R-1}\mb{E}\left\|\m{h}_r- \nabla f(\m{x}_r, \m{Z}_r)\right\| &\leq 
 2(1-\rho)^2 \frac{M_f^2}{\rho  MKb R} \sum_{r=0}^{R-1}\mb{E} \left\| \left(\m{x}_r,\m{Z}_r\right)-\left(\m{x}_{r-1},\m{Z}_{r-1}\right) \right\|\\
& + 2\rho \frac{\sigma^2}{MKb}+\frac{\sigma^2}{\rho MKb}
\end{align}

%
%
Now, from Lemma~\ref{lem:drift:fedmsa}, we have 
\begin{align}
 \nonumber 
 \left\| \left(\m{x}_r^m,\m{Z}_r^m\right)-\left(\m{x}_{r-1},\m{Z}_{r-1}\right) \right\| &\leq  8 e^2 K^2 \eta^2  \left(\mb{E} \left\| \m{v}_r- \nabla f(\m{x}_r)\right\|^2 + \sum_{n=1}^N\mb{E} \left\|\m{z}_k^n-\m{z}^{n,*}(\m{z}_k^{n-1})\right\|^2  \right) \\
 &+  \frac{10 e K^2 \eta^2}{K}\sum_{k=1}^K \left\| \nabla f(\m{x}_{r+1,k}^{\tilde{m}})\right\| 
\end{align}
Hence, we have
%
\begin{align}
 \nonumber 
 \left\| \left(\m{x}_r,\m{Z}_r\right)-\left(\m{x}_{r-1},\m{Z}_{r-1}\right) \right\| = &\leq  8 e^2 K^2 \eta^2  \left(\mb{E} \left\| \m{v}_r- \nabla f(\m{x}_r)\right\|^2 + \sum_{n=1}^N\mb{E} \left\|\m{z}_k^n-\m{z}^{n,*}(\m{z}_k^{n-1})\right\|^2  \right) \\
 &+  \frac{10 e K^2 \eta^2}{K}\sum_{k=1}^K \left\| \nabla f(\m{x}_{r+1,k}^{\tilde{m}})\right\| 
\end{align}
Thus, 
\begin{align*}
\nonumber 
\sum_{r=0}^{R-1}\mb{E}\left\|\m{h}_r- \nabla f(\m{x}_r, \m{Z}_r)\right\| &\leq 
\frac{ 16 M_f^2 K^2 \alpha^2}{\rho  MKb R} \sum_{r=0}^{R-1}\left(\mb{E} \left\| \m{v}_r- \nabla f(\m{x}_r, \m{Z}_r)\right\|^2 + \sum_{n=1}^N\mb{E} \left\|\m{z}_k^n-\m{z}^{n,*}(\m{z}_k^{n-1})\right\|^2  \right)\\
& + 2\rho \frac{\sigma^2}{MKb}+\frac{\sigma^2}{\rho MKb}\\
&\leq 
\frac{ 1}{ (24 e +1)R} \sum_{r=0}^{R-1} \left(\mb{E} \left\| \m{v}_r- \nabla f(\m{x}_r,\m{Z}_r)\right\|^2 + \sum_{n=1}^N\mb{E} \left\|\m{z}_k^n-\m{z}^{n,*}(\m{z}_k^{n-1})\right\|^2  \right)\\
& + 2\rho \frac{\sigma^2}{MKb}+\frac{\sigma^2}{\rho MKb}.
\end{align*}
Hence,

\end{proof}
The following lemma provides a bound on the \textit{drift} of each $\m{x}_{i,\nu}$ from $\m{x}$ for stochastic nonconvex bilevel problems. 

\begin{lemma}[Drifting Error II]\label{thm4:lemma2}
Suppose Assumptions~\ref{assu:f} and \ref{assu:bound:var} hold. Further, assume $\tau_i \geq 1$ and $ \alpha_i\leq 1/(5M_f\tau_i), \forall i \in \mathcal{S}$. Then, for each $i \in \mathcal{S}$ and $\forall \nu \in\{0,\ldots, \tau_i-1\}$,  \fedout guarantees:
\begin{align}\label{eqn1:lemm:drift}
\nonumber
 \mb{E}\left[\left\|\m{x}_{i,\nu}-\m{x}\right\|^2\right] 
%  \leq 9  \tau_i \alpha_i^2 \left( 4\tau_i  \left( M_f^2 \mb{E}\left[\|\m{y}^+-\m{y}^\star(\m{x})\|^2\right]+  \mb{E}\left[\|\nabla f(\m{x})\|^2\right]+ 3  b^2\right) + 3 \tilde{\sigma}_f^2 \right).\\
 &\leq 36 \tau_i^2 \alpha_i^2 \left(M_f^2 \mb{E}\left[\|\m{y}^+-\m{y}^\star(\m{x})\|^2\right]+  \mb{E}\left[\|\nabla f(\m{x})\|^2\right]+ 3 b^2\right) \\
 &+ 27 \tau_i \alpha_i^2  \tilde{\sigma}_f^2.
\end{align}
\end{lemma}
\begin{proof}
The result trivially holds for $\tau_i=1$. Let $\tau_i>1$ and define
\begin{equation}\label{eqn1+:lemm:drift}
\begin{aligned}
\m{v}_{i,\nu}&:= \bar{\m{h}}_i(\m{x}_{i,\nu}, \m{y}^+)- \bar{\nabla} f_i(\m{x}_{i,\nu}, \m{y}^+)- \bar{\m{h}}_i(\m{x},\m{y}^+) \\
& +\bar{\nabla} f_i(\m{x}, \m{y}^+) +\bar{\m{h}}(\m{x},\m{y}^+) -\bar{\nabla} f(\m{x}, \m{y}^+),\\
\m{w}_{i,\nu}&:= \m{h}_i(\m{x}_{i,\nu}, \m{y}^+)-\bar{\m{h}}_i(\m{x}_{i,\nu},\m{y}^+)+\bar{\m{h}}_i(\m{x},\m{y}^+)\\
&-\m{h}_i(\m{x},\m{y}^+)+\m{h}(\m{x},\m{y}^+)-\bar{\m{h}} (\m{x},\m{y}^+),\\
\m{z}_{i,\nu}&:=\bar{\nabla} f_i(\m{x}_{i,\nu}, \m{y}^+) - \bar{\nabla} f_i(\m{x}, \m{y}^+)+  \bar{\nabla} f(\m{x}, \m{y}^+) - \nabla f(\m{x}) + \nabla  f(\m{x}).
\end{aligned}
\end{equation}
One will notice that 
$$
\m{v}_{i,\nu}+\m{w}_{i,\nu}+\m{z}_{i,\nu} = \m{h}_i(\m{x}_{i,\nu}, \m{y}^+)-\m{h}_i(\m{x},\m{y}^+)+\m{h}(\m{x},\m{y}^+).
$$
%
Hence, from Algorithm~\ref{alg:fedout}, for each $i\in\mathcal{S}$, and $\forall  \nu \in\{0,\ldots,\tau_i-1\}$, we have   
\begin{equation}
\begin{aligned}
        \m{x}_{i,\nu+1}-\m{x}&=\m{x}_{i,\nu}-\m{x}-\alpha_i (\m{v}_{i,\nu}+\m{w}_{i,\nu}+\m{z}_{i,\nu}),
    \end{aligned}
\end{equation}
which implies that 
\begin{equation}\label{eqn2:lemm:drift}
\begin{aligned}
\mb{E}\left[\|\m{x}_{i,\nu+1}-\m{x}\|^2\right]
&=\mb{E}\left[\|\m{x}_{i,\nu}-\m{x}-\alpha_i (\m{v}_{i,\nu}+\m{z}_{i,\nu})\|^2\right]+\alpha_i^2\mb{E}\left[\|{\m{w}_{i,\nu}}\|^2\right]\\&-2\mb{E}\left[\mb{E}\left[\langle \m{x}_{i,\nu}-\m{x}-\alpha_i(\m{v}_{i,\nu}+\m{z}_{i,\nu}),\alpha_i \m{w}_{i,\nu} \rangle\mid\mathcal{F}_{i,\nu-1}\right]\right] \\ 
&= \mb{E}\left[\|\m{x}_{i,\nu}-\m{x}-\alpha_i(\m{v}_{i,\nu}+\m{z}_{i,\nu})\|^2\right]+\alpha_i^2\mb{E}\left[\|\m{w}_{i,\nu}\|^2\right].
\end{aligned}
\end{equation}
Here, the last equality uses Lemma~\ref{lem:rand:zer} since  $\mb{E}[\m{w}_{i,\nu}|\mathcal{F}_{i,\nu-1}]=0$, {by definition}.

From Lemmas~\ref{lem:Jens}, \ref{lem:neum:bias}, and \ref{lem:lips},  for $\m{v}_{i,\nu}$, $\m{w}_{i,\nu}$, and $\m{z}_{i,\nu}$ defined in \eqref{eqn1+:lemm:drift}, we have
\begin{subequations}\label{eqn3:v-z:drift}
\begin{equation}
\label{eqn3a:lemm:drift}
\begin{aligned}
\mb{E}\Big[\|\m{v}_{i,\nu}\|^2\Big]  &\leq 3  \mb{E}\Big[ \left\|\bar{\nabla} f_i(\m{x}_{i,\nu}, \m{y}^+)-\bar{\m{h}}_i(\m{x}_{i,\nu},\m{y}^+) \right\|^2 \\
&+\left\|\bar{\m{h}}_i(\m{x},\m{y}^+)-\bar{\nabla} f_i(\m{x},\m{y}^+)\right\|^2+\left\|\bar{\nabla} f(\m{x},\m{y}^+)-\bar{\m{h}} (\m{x},\m{y}^+)\right\|^2 \Big]\\
&\leq  9 b^2,
\end{aligned}
\end{equation}
%where the first inequality follows from \eqref{eqn1+:lemm:drift} and Lemma~\ref{lem:Jens} and the last inequality uses Lemma~\ref{lem:neum:bias}.
%
%Similarly, we obtain
\begin{equation}
\label{eqn3b:lemm:drift}
\begin{aligned}
\mb{E}\left[\|\m{w}_{i,\nu}\|^2\right] &\leq 3   \mb{E}\Big[ \|\m{h}_i(\m{x}_{i,\nu},\m{y}^+)-\bar{\m{h}}_i(\m{x}_{i,\nu},\m{y}^+)\|^2\\
&+\|\bar{\m{h}}_i(\m{x},\m{y}^+)-\m{h}_i(\m{x},\m{y}^+)\|^2+\|\m{h}(\m{x},\m{y}^+)-\bar{\m{h}} (\m{x},\m{y}^+)\|^2\Big]\\
        & \leq 9\tilde{\sigma}_f^2,
    \end{aligned}
\end{equation}
%where the last inequality uses Lemma~\ref{lem:lips}.
and
\begin{equation}
\label{eqn3c:lemm:drift}
\begin{aligned}
\mb{E}\left[\|\m{z}_{i,\nu}\|^2\right] &\leq 3   \mb{E}\Big[ \|
\bar{\nabla} f_i(\m{x}_{i,\nu}, \m{y}^+) - \bar{\nabla} f_i(\m{x}, \m{y}^+)\|^2\\
&+\|  \bar{\nabla} f(\m{x}, \m{y}^+) - \nabla f(\m{x})\|^2+ \|\nabla  f(\m{x})\|^2\Big]\\
& \leq 3\left(M_f^2 \mb{E}\left[\|\m{x}_{i,\nu}-\m{x}\|^2\right]+ M_f^2 \mb{E}\left[\|\m{y}^+-\m{y}^\star(\m{x})\|^2\right]+  \mb{E}\left[\|\nabla f(\m{x})\|^2\right]\right).
\end{aligned}
\end{equation}
\end{subequations}

Now, the first term in the RHS of \eqref{eqn2:lemm:drift} can be bounded as follows:
\begin{equation}
\label{eqn4:lemm:drift}
\begin{aligned}
\mb{E}\left[\|\m{x}_{i,\nu}-\m{x}-\alpha_i(\m{v}_{i,\nu}+\m{z}_{i,\nu})\|^2\right] &\leq  \left(1+\frac{1}{2\tau_i-1}\right)\mb{E}\left[\|\m{x}_{i,\nu}-\m{x}\|^2\right]+ 2\tau_i \mb{E}\left[\|\alpha_i (\m{v}_{i,\nu}+\m{z}_{i,\nu})\|^2\right]\\
&\leq  \left(1+\frac{1}{2\tau_i-1}\right)\mb{E}\left[\|\m{x}_{i,\nu}-\m{x}\|^2\right]+ 4\tau_i \alpha_i^2  \left(\mb{E}\left[\| \m{z}_{i,\nu}\|^2\right] + \mb{E}\left[\| \m{v}_{i,\nu}\|^2\right] \right)\\
%2\tau_i \mb{E}\Big[\|\alpha_i (\m{v}_{i,\nu}+\m{z}_{i,\nu})\|^2\Big]\\
 &\leq  \left(1+\frac{1}{2\tau_i-1}\right)\mb{E}\left[\|\m{x}_{i,\nu}-\m{x}\|^2\right]+ 4\tau_i \alpha_i^2  \left(\mb{E}\left[\| \m{z}_{i,\nu}\|^2\right] + 9  b^2\right)\\
     % &\leq  (1+\frac{1}{2\tau_i-1})\mb{E}\Big[\|\m{x}_{i,\nu}-\m{x}\|^2\Big]+ 2\tau_i \mb{E}\Big[\|\alpha_i( \bar{\nabla} f_i(\m{x}_{i,\nu}, \m{y})-\bar{\nabla} f_i(\m{x},\m{y}))-\alpha_i \bar{\nabla} f(\m{x},\m{y})\|^2\Big] +\\
%       &\leq  (1+\frac{1}{2\tau_i-1})\mb{E}\Big[\|\m{x}_{i,\nu}-\m{x}\|^2\Big]+ 10 \tau_i \alpha_i^2M_f^2\mb{E}\Big[\|\m{x}_{i,\nu}-\m{x}\|\Big]+ 10\tau_i \alpha_i^2  \mb{E}\Big[\|\bar{\nabla} f(\m{x},\m{y})\|^2\Big] + 10b^2  \\
       &\leq  \left(1+\frac{1}{2\tau_i-1}+12\tau_i \alpha_i^2 M_f^2\right)\mb{E}\left[\|\m{x}_{i,\nu}-\m{x}\|^2\right]\\
       &+ 12\tau_i \alpha_i^2 \left( M_f^2 \mb{E}\left[\|\m{y}^+-\m{y}^\star(\m{x})\|^2\right]+  \mb{E}\left[\|\nabla f(\m{x})\|^2\right]+ 3 b^2\right).
    \end{aligned}
\end{equation}
Here, the first inequality follows from Lemma~\ref{lem:trig}; the second inequality uses Lemma~\ref{lem:Jens}; and the third and last inequalities follow from \eqref{eqn3a:lemm:drift} and \eqref{eqn3c:lemm:drift}.

%\eqref{eqn1+:lemm:drift}, Lemmas~\ref{lem:Jens} and \ref{lem:lips}.

Substituting \eqref{eqn4:lemm:drift} into \eqref{eqn2:lemm:drift} gives 
\begin{equation}
\label{eqn5:lemm:drift}
\begin{aligned}
        \mb{E}\left[\left\|\m{x}_{i,\nu+1}-\m{x}\right\|^2\right]&\leq \left(1+\frac{1}{2\tau_i-1}+12\tau_i \alpha_i^2 M_f^2\right)\mb{E}\left[\|\m{x}_{i,\nu}-\m{x}\|^2\right]\\
       & + 12\tau_i \alpha_i^2 \left( M_f^2 \mb{E}\left[\|\m{y}^+-\m{y}^\star(\m{x})\|^2\right]+  \mb{E}\left[\|\nabla f(\m{x})\|^2\right]+ 3  b^2\right) + 9 \alpha_i^2 \tilde{\sigma}_f^2 \\
        &\leq \left(1+\frac{1}{\tau_i-1}\right)\mb{E}\left[\|\m{x}_{i,\nu}-\m{x}\|^2\right] \\
        & + 12\tau_i \alpha_i^2 \left( M_f^2 \mb{E}\left[\|\m{y}^+-\m{y}^\star(\m{x})\|^2\right]+  \mb{E}\left[\|\nabla f(\m{x})\|^2\right]+ 3  b^2\right) + 9 \alpha_i^2 \tilde{\sigma}_f^2. \\
    \end{aligned} 
\end{equation}
Here, the first inequality uses \eqref{eqn3b:lemm:drift} and the last inequality follows by noting $\alpha_i\leq 1/(5M_f\tau_i)$. 
%\ct{Again might seem strange that you sub $\alpha_i=\alpha/\tau_i$ for some parts and not others.}

For all $\tau_i>1$, we have
\begin{equation}\label{eqn:sum:geom}
\begin{split}
\sum\limits_{j=0}^{\nu -1} \left(1+\frac{1}{\tau_i-1}\right)^j &= \frac{ \left(1+\frac{1}{\tau_i-1}\right)^{\nu }-1}{\left(1+\frac{1}{\tau_i-1}\right)-1} \\
&\leq  \tau_i {\left(1+\frac{1}{\tau_i} \right)}^{\nu } \leq \tau_i {\left(1+\frac{1}{\tau_i} \right)}^{\tau_i} \leq \exp{(1)}\tau_i < 3 \tau_i. 
\end{split}
\end{equation}
Now, iterating equation \eqref{eqn5:lemm:drift} and using $\m{x}_{i,0}=\m{x}, \forall i\in\mathcal{S}$, we obtain
\begin{equation*}
\begin{aligned}
        \mb{E}\left[\|\m{x}_{i,\nu}-\m{x}\|^2\right]&\leq  \left( 12\tau_i \alpha_i^2 \left( M_f^2 \mb{E}\left[\|\m{y}^+-\m{y}^\star(\m{x})\|^2\right]+  \mb{E}\left[\|\nabla f(\m{x})\|^2\right]+ 3  b^2\right) + 9 \alpha_i^2 \tilde{\sigma}_f^2 \right) \sum\limits_{j=0}^{\nu -1} \left(1+\frac{1}{\tau_i-1}\right)^j\\
        &\leq 3 \tau_i \left( 12\tau_i \alpha_i^2 \left( M_f^2 \mb{E}\left[\|\m{y}^+-\m{y}^\star(\m{x})\|^2\right]+  \mb{E}\left[\|\nabla f(\m{x})\|^2\right]+ 3  b^2\right) + 9 \alpha_i^2 \tilde{\sigma}_f^2 \right),
    \end{aligned}
\end{equation*}
where the second inequality uses \eqref{eqn:sum:geom}. This completes the proof.
\end{proof}
%

\begin{remark}
Lemma~\ref{thm4:lemma2} shows that the bound on the client-drift scales linearly with $\tau_i$ and the inner error $\|\m{y}^+-\m{y}^\star(\m{x})\|^2$ in general nested FL. We aim to control such a drift by selecting $\alpha_i=\mc{O}(1/\tau_i)$ for all $ i \in \mc{S}$ and using the inner error bound provided in Lemma~\ref{thm:fedin}. 
\end{remark}

Next, we provide the proof of our main result which can be adapted to general nested problems (bilevel, min-max, compositional). 
\subsection{Proof of Theorem ~\ref{thm:fednest}}
\begin{proof}
We define the following Lyapunov function 
\begin{equation}\label{eqn:lyapfunc}
 \mb{W}^k:= f(\m{x}^k)  + \frac{M_f}{L_{\m{y}}}\|\m{y}^k - \m{y}^\star(\m{x}^k)\|^2.   
\end{equation}
Motivated by \citep{chen2021closing}, we bound the difference between two Lyapunov functions. That is,
\begin{align}\label{eqn:lyapfunc:diff}
  \mb{W}^{k+1}  -  \mb{W}^k   =  &  f(\m{x}^{k+1}) -  f(\m{x}^k)+\frac{M_f}{L_{\m{y}}}\left(\|\m{y}^{k+1} - \m{y}^*(\m{x}^{k+1})\|^2 - \|\m{y}^k - \m{y}^\star(\m{x}^k)\|^2\right).
\end{align}
The first two terms on the RHS of \eqref{eqn:lyapfunc:diff} quantifies the descent of outer objective $f$ and the reminding terms measure the descent of the inner errors.  

From our assumption, we have  $\alpha_i^k=\alpha_k/\tau_i$, $\beta_i^k=\beta_k/\tau_i$,  $\forall i \in \mathcal{S}$. Substituting these stepsizes into the bounds provided in  Lemmas \ref{lem:dec} and \ref{thm:fedin}, and using \eqref{eqn:lyapfunc:diff}, we get 
\begin{subequations}\label{eqn:dec:lyap2}
\begin{align}
\nonumber 
\qquad \mb{E}[\mb{W}^{k+1}] - \mb{E}[\mb{W}^k]  &\leq  \left(\frac{L_f \alpha_k^2 }{2} + \frac{M_f}{L_{\m{y}}} a_3(\alpha_k)\right)\tilde{\sigma}_f^2 + \frac{3\alpha_k}{2} b^2,
\\
 &  -\frac{\alpha_k}{2}\mb{E}\left[\|\nabla f(\m{x}^k)\|^2\right] + \frac{3 M_f^2 \alpha_k }{2m}\sum \limits_{i=1}^m \frac{1}{\tau_i}\sum \limits_{k=0}^{K-1}\mb{E}\left[\|\m{x}_{i,\nu}^k-\m{x}^k\|^2\right]
\label{eqn:dec:lyap2i1}
\\
  & -  \left(\frac{\alpha_k}{2}-\frac{L_f\alpha_k^2}{2}-\frac{M_f}{L_\m{y}} a_1(\alpha_k)\right)  \mb{E}\left[ \left\| \frac{1}{M}\sum\limits_{m=1}^{M} \frac{1}{\tau_i} \sum\limits_{k=0}^{K-1} \bar{\m{h}}_i(\m{x}_{i,\nu}^k,\m{y}^{k+1})\right\|^2 \right] 
\label{eqn:dec:lyap2i2}   
   \\
   &+ \frac{M_f}{L_{\m{y}}} \left( \frac{3 M_f L_{\m{y}}\alpha_k }{2} +a_2(\alpha_k)\right) \mb{E}\left[\|\m{y}^{k+1}-\m{y}^*(\m{x}^k)\|^2\right]-  \frac{M_f}{L_{\m{y}}} \mb{E}\left[\|\m{y}^k-\m{y}^*(\m{x}^k)\|^2\right],
\label{eqn:dec:lyap2i3}  
 %&+   \frac{25 M_f a_3(\alpha_k) }{L_{\m{y}}} T \beta_k^2 \sigma^2_{g,1}\\
\end{align}
\end{subequations}
where $a_1(\alpha)-a_3(\alpha)$ are defined in \eqref{eqn:a1-3}.

Let
\begin{equation}\label{eqn:stepsize0}
\alpha_i^k=\frac{\alpha_k}{\tau_i},~~\forall i \in \mathcal{S}~ ~~\textnormal{where}~~\alpha_k \leq \frac{1}{ 216M_f^2 +5M_f}.
\end{equation}
 The above choice of $\alpha_k$ satisfies the condition of Lemma~\ref{thm4:lemma2} and we have $54 M_f^2 \alpha_k^3 \leq \alpha_k^2/4$. Hence, from  Lemma~\ref{thm4:lemma2}, we get
\begin{equation}\label{eqn:step1}
\begin{aligned}
\eqref{eqn:dec:lyap2i1}
% & \leq 
% - \frac{\alpha_k}{2}\mb{E}[\|\nabla f(\m{x}^k)\|^2] +    \frac{3 M_f^2 \alpha_k^3 }{2} \mb{E}[\|\nabla f(\m{x}^k)\|^2] + \frac{45M_f^2 \alpha_k^3  }{2}  \left(3\tilde{\sigma}_f^2 +8b^2_k\right)+ 30 \alpha_k^3 \|\m{y}^{k+1}-\m{y}^\star(\m{x})\|^2 \\
 \leq &- \frac{\alpha_k}{2}\mb{E}\left[\|\nabla f(\m{x}^k)\|^2\right] + \frac{81}{2} \alpha_k^3 M_f^2\tilde{\sigma}_f^2\\
&+ 54 M_f^2 \alpha_k^3 \left(M_f^2 \mb{E}\left[\|\m{y}^{k+1}-\m{y}^\star(\m{x}^k)\|^2\right]+  \mb{E}\left[\|\nabla f(\m{x}^k)\|^2\right]+ 3 b^2\right)\\
%&\leq - \frac{\alpha_k}{4}\mb{E}[\|\nabla f(\m{x}^k)\|^2] + 54 M_f^2 \alpha_k^3 \left(M_f^2 \mb{E}\left[\|\m{y}^{k+1}-\m{y}^\star(\m{x}^k)\|^2\right]+ 3 b^2\right) + \frac{81}{2} \alpha_k^3 M_f^2\tilde{\sigma}_f^2\\
\leq &- \frac{\alpha_k}{4}\mb{E}\left[\|\nabla f(\m{x}^k)\|^2\right] + \frac{\alpha_k^2}{4}\tilde{\sigma}_f^2+ \frac{\alpha_k^2}{4} \left(M_f^2 \mb{E}\left[\|\m{y}^{k+1}-\m{y}^\star(\m{x}^k)\|^2\right]+ 3 b^2\right)\\
\leq &- \frac{\alpha_k}{4}\mb{E}\left[\|\nabla f(\m{x}^k)\|^2\right] + \frac{\alpha_k^2}{4}\tilde{\sigma}_f^2+ \frac{3\alpha_k^2}{4} b^2\\
&+  \frac{25M_f }{L_{\m{y}}} \left(\frac{M_fL_{\m{y}}}{4} \alpha_k^2 \right) T\beta_k^2\sigma_{g,1}^2 +\frac{M_f  }{L_{\m{y}}} \left( \frac{M_fL_{\m{y}}}{4} \alpha_k^2\right)\left(1-  \frac{{\beta}_k \mu_g}{2} \right)^T, 
%\\
%& \leq - \frac{\alpha_k}{4}\mb{E}[\|\nabla f(\m{x}^k)\|^2] + 54 M_f^2 \alpha_k^3 \left(M_f^2 \mb{E}\left[\|\m{y}^+-\m{y}^\star(\m{x})\|^2\right]+ 3 b^2\right) + \frac{81}{2} \alpha_k^3 M_f^2\tilde{\sigma}_f^2
\end{aligned}
\end{equation}
where the first inequlaity uses \eqref{eqn:stepsize0} and the last inequality follows from \eqref{eqn:err:fedina1}.

To guarantee the descent of $\mb{W}^k$, the following constraints need to be satisfied
%\begin{subequations}
\begin{equation}\label{eqn:stepsize1}
\begin{aligned}
\eqref{eqn:dec:lyap2i2} &\leq  0, \\
&\Longrightarrow~~ \frac{\alpha_k}{2}-\frac{L_f\alpha_k^2}{2} -\frac{M_f}{L_\m{y}} \left( L_{\m{y}}^2 \alpha^2_k+ \frac{L_{\m{y}}\alpha_k}{4M_f} +\frac{L_{\m{yx}} \alpha^2_k}{2\eta}\right) \geq 0,\\
&\Longrightarrow~~\alpha_k\leq \frac{1}{2L_f+4M_fL_{\m{y}}+\frac{2M_fL_{\m{yx}}}{L_{\m{y}}\eta}}, %=:\bar\alpha_1.
\end{aligned}
\end{equation}
where the second line uses \eqref{eqn:a1-3}.


% Here, we use our assumption that 
% \begin{equation}\label{eqn:stepsize0}
%  \alpha_k \leq \frac{1}{15M_f}.   
% \end{equation}
% where we select $\bar\alpha_3 := 1/8M_f$.

Further, substituting \eqref{eqn:err:fedin1} in \eqref{eqn:dec:lyap2i3} gives
% using Lemma~\ref{thm:fedin}, we have 
\begin{equation}\label{eqn:step2}
\begin{aligned}
 \eqref{eqn:dec:lyap2i3} & \leq  \frac{25M_f }{L_{\m{y}}} \left( \frac{3 M_f L_{\m{y}}\alpha_k }{2}  +a_2(\alpha_k)\right) T\beta_k^2\sigma_{g,1}^2
 \\
 & +\frac{M_f  }{L_{\m{y}}}  \left(\left( \frac{3 M_f L_{\m{y}}\alpha_k }{2}  +a_2(\alpha_k)\right)\left(1-  \frac{{\beta}_k \mu_g}{2} \right)^T -1\right) \mb{E}[\|\m{y}^{k}-\m{y}^*(\m{x}^k)\|^2].
\end{aligned}
\end{equation}
% To do so,  let $\alpha_i^k=\frac{\alpha_k}{\tau_i}, \forall i \in \mathcal{S}$, where 
% \begin{equation}\label{eqn4:dec:fedinn}
% \begin{aligned}
% % C_1= \Big(\frac{\alpha_k}{2}-\frac{L_f\alpha_k^2}{2}-\frac{M_f}{L_{\m{y}}} L_{\m{y}}^2\alpha_k^2- \frac{M_f}{L_{\m{y}}}\frac{\alpha_k^2L_{\m{y}}^2}{4\gamma_k}-\frac{M_f}{L_{\m{y}}}\frac{L_{y\m{x}}\alpha_k^2}{4\eta}\Big) \\
% % C_3 =\frac{M_f}{L_\m{y}}\Big(1 + \gamma_k + M_fL_\m{y}\alpha_k + \frac{\eta L_{\m{y}\m{x}}\tilde{C}_f^2}{4}\alpha_k^2 \Big)
% %\\
% C_1 (\alpha_k)&:= \frac{\alpha_k}{2}-\frac{L_f\alpha_k^2}{2}-\frac{M_f}{L_\m{y}} a_1(\alpha_k) %L_\m{y}^2\alpha_k^2- \frac{M_f}{L_\m{y}} \frac{\alpha_k^2L_\m{y}^2}{4\gamma_k}-\frac{M_f}{L_\m{y}} \frac{L_{\m{y}\m{x}}\alpha_k^2}{4\eta},
% \\
% C_2 (\alpha_k) &:= \frac{M_f}{L_{\m{y}}}\Big(a_2(\alpha_k)(1-\rho_g\beta_k)^T -1\Big),\\
% C_3(\alpha_k) &:=  \frac{M_f}{L_{\m{y}}}\Big(1 + 2M_fL_{\m{y}}\alpha_k + \frac{\eta L_{\m{yx}}\tilde{D}_f^2}{4}\alpha_k^2 \Big),\\
% C_4(\alpha_k)&:= \Big(\frac{L_f}{2} + M_fL_{\m{y}} +\frac{L_{\m{yx}}M_f}{4\eta L_{\m{y}}}\Big)\alpha_k^2.
% \end{aligned}
% \end{equation}
Substituting  \eqref{eqn:step1}--\eqref{eqn:step2} into \eqref{eqn:dec:lyap2} gives 
% We bound the two difference terms in \eqref{eq.diff-Lya} and obtain
\begin{subequations}\label{eqn:dec:lyap}
\begin{align}
%\begin{equation}
%\begin{aligned}
\nonumber 
   \mb{E}[\mb{W}^{k+1}] - \mb{E}[\mb{W}^k]  \leq & -\frac{\alpha_k}{4}\mb{E}[\|\nabla f(\m{x}^k)\|^2]
   \\
\nonumber    
   &+ \left(\frac{3}{2} \alpha_k+ \frac{3}{4}\alpha_k^2\right)b^2\\
   \nonumber 
   &+ \left(\left(\frac{L_f}{2}+\frac{1}{4}\right) \alpha_k^2  +  \frac{M_f}{L_{\m{y}}} a_3(\alpha_k) \right)\tilde{\sigma}_f^2 \\
   \nonumber 
   &+\frac{25M_f}{L_{\m{y}}}  \left( \frac{M_fL_{\m{y}}}{4} \alpha_k^2+  \frac{3 M_f L_{\m{y}}\alpha_k }{2}  +a_2(\alpha_k)\right) T\beta_k^2\sigma_{g,1}^2
%   & -  \left(\frac{\alpha_k}{2}-\frac{L_f\alpha_k^2}{2}-\frac{M_f}{L_\m{y}} a_1(\alpha_k)\right)  \mb{E}\left[ \| \frac{1}{M}\sum\limits_{m=1}^{M} \frac{1}{\tau_i} \sum\limits_{k=0}^{K-1} \bar{\m{h}}_i(\m{x}_{i,\nu}^k,\m{y}^{k+1})\|^2 \right] \\
\\
   &+  \frac{M_f  }{L_{\m{y}}}  \left( \left( \frac{M_fL_{\m{y}}}{4} \alpha_k^2+ \frac{3 M_f L_{\m{y}}\alpha_k }{2}  +a_2(\alpha_k)\right)\left(1-  \frac{{\beta}_k\mu_g}{2} \right)^T -1\right) \mb{E}[\|\m{y}^{k}-\m{y}^*(\m{x}^k)\|^2]. \label{eqn:dec:lyap4} 
%\end{aligned}
%\end{equation}
\end{align}
\end{subequations}
%
Let $\beta_k <  \min\big(1/(6\ell_{g,1}),1\big)$. Then, we have  $\beta_k\mu_g/2 < 1 $. This together with \eqref{eqn:a1-3} implies that for any $\alpha_k >0$ 
\begin{equation}\label{eqn:stepsize2}
\begin{aligned}
      \eqref{eqn:dec:lyap4}& \leq  0,\\
     &\Longrightarrow~~ \left(1+  \frac{M_fL_{\m{y}}}{4} \alpha_k^2+ \frac{11M_f L_{\m{y}} \alpha_k}{2} + \frac{\eta L_{\m{yx}}\tilde{D}_f^2 \alpha^2_k}{2} \right)\left(1-  \frac{{\beta}_k\mu_g}{2} \right)^T -1 \leq  0,\\
      &\Longrightarrow \exp\left(\frac{M_fL_{\m{y}}}{4} \alpha_k^2+ \frac{11M_f L_{\m{y}} \alpha_k}{2} + \frac{\eta L_{\m{yx}}\tilde{D}_f^2 \alpha^2_k}{2}\right) \exp\left(- \frac{T{\beta}_k\mu_g}{2} \right) -1 \leq 0, \\
      &\Longrightarrow~~\beta_k\geq \frac{11 M_fL_{\m{y}} + \eta L_{\m{yx}}\tilde{D}_f^2 \alpha_k + \frac{M_f L_{\m{y}}\alpha_k}{2}}{\mu_g} \cdot \frac{\alpha_k}{T}.
    % &\Longrightarrow~~\beta_k\geq \frac{5M_fL_{\m{y}} + \frac{\eta L_{\m{yx}}\tilde{D}_f^2}{4} \bar{\alpha}_1}{T\mu_g} \alpha_k,
\end{aligned}
\end{equation}
% where the second line uses \eqref{eqn:a1-3}.
%where the last inequality uses \eqref{eqn:stepsize1}.
%\end{subequations}

 From \eqref{eqn:stepsize0}, \eqref{eqn:stepsize1} and \eqref{eqn:stepsize2}, we select
 \begin{equation}\label{eq.step-cond-3}
    \alpha_k=\min\{\bar\alpha_1, \bar\alpha_2, \bar\alpha_3,\frac{\bar\alpha}{\sqrt{K}}\},~~~~~~~\beta_k=\frac{\bar{\beta}\alpha_k}{T},
\end{equation}
 where 
\begin{equation}\label{eqn2:dec:lyap}
\begin{aligned}
\bar{\beta}&:=\frac{1}{\mu_g} \left(11 M_fL_{\m{y}} + \eta L_{\m{yx}}\tilde{D}_f^2\bar\alpha_1 + \frac{M_fL_{\m{y}} \bar\alpha_1}{2}\right),\\
\bar\alpha_1&:=\frac{1}{2L_f+4M_fL_{\m{y}}+\frac{2M_fL_{\m{yx}}}{L_{\m{y}}\eta}},
~~~\bar\alpha_2:= \frac{T}{8\ell_{g,1} \bar{\beta}}, 
%\frac{6T\rho_g}{\left(22M_fL_{\m{y}} + \eta L_{\m{yx}}\tilde{D}_f^2\bar\alpha_1 + M_fL_{\m{y}} \bar\alpha_1\right)}, 
~~~\bar\alpha_3:= \frac{1}{216M_f^2+5M_f}, \\
\end{aligned}
\end{equation}
%Here, $\rho_g:=\frac{\mu_g\ell_{g,1}}{\mu_g+\ell_{g,1}}$. 
%To satisfy \eqref{eqn:stepsize1} and \eqref{eqn:stepsize2}, we choose

With the above choice of stepsizes, \eqref{eqn:dec:lyap} can be simplified as
\begin{equation}\label{eqn:dec3:lyap}
\begin{aligned}
   \mb{E}[\mb{W}^{k+1}] - \mb{E}[\mb{W}^k] & \leq  -\frac{\alpha_k}{4}\mb{E}[\|\nabla f(\m{x}^k)\|^2] \\
%   & -  \left(\frac{\alpha_k}{2}-\frac{L_f\alpha_k^2}{2}-\frac{M_f}{L_\m{y}} a_1(\alpha_k)\right)  \mb{E}\left[ \| \frac{1}{M}\sum\limits_{m=1}^{M} \frac{1}{\tau_i} \sum\limits_{k=0}^{K-1} \bar{\m{h}}_i(\m{x}_{i,\nu}^k,\m{y}^{k+1})\|^2 \right] \\
%   &+  \frac{M_f  }{L_{\m{y}}}  \left( (M_f L_{\m{y}}\alpha_k +a_2(\alpha_k))\left(1-  \frac{{\beta}_k\mu_g}{2} \right)^T -1\right) \mb{E}[\|\m{y}^{k+1}-\m{y}^*(\m{x}^k)\|^2] \\
%   &+ \left(\frac{3\alpha_k}{2}+ 24\alpha_k^2\right)b^2\\
%   &+ \left(\frac{L_f \alpha_k^2 }{2} + a_3(\alpha_k)+ 9 \alpha_k^2 \right)\tilde{\sigma}_f^2 \\
%   &+\frac{25M_f}{L_{\m{y}}}  \left(M_f L_{\m{y}}\alpha_k +a_2(\alpha_k)\right)\sigma_{g,1}^2 \\
   &+ \left(\frac{3}{2} \alpha_k+ \frac{3}{4}\alpha_k^2\right)b^2\\
   &+ \left(\frac{L_f+\frac{1}{2}}{2} \alpha_k^2  +  \frac{M_f}{L_{\m{y}}} a_3(\alpha_k) \right)\tilde{\sigma}_f^2 \\
   &+\frac{25M_f}{L_{\m{y}}}  \left( \frac{M_fL_{\m{y}}}{4} \alpha_k^2+ \frac{3 M_f L_{\m{y}} }{2}  \alpha_k +a_2(\alpha_k)\right) T\beta_k^2\sigma_{g,1}^2\\
   & \leq  - \frac{\alpha_k}{4} \mb{E}[\|\nabla f(\m{x}^k)\|^2]  + c_1\alpha_k^2\sigma_{g,1}^2 +    \left(\frac{3}{2} \alpha_k+ \frac{3}{4}\alpha_k^2\right)b^2+ c_2\alpha_k^2\tilde\sigma_f^2,
\end{aligned}
\end{equation}
where the constants $c_1$ and $c_2$ are defined as
\begin{equation}\label{eqn44:dec:lyap}
\begin{aligned}
    &c_1=\frac{25 M_f}{L_{\m{y}}}\left( 1+ \frac{11 M_f L_{\m{y}}}{2} \bar{\alpha}_1  +  \left(\frac{M_fL_{\m{y}} + 2\eta L_{\m{yx}}\tilde{D}_f^2 }{4} \right)\bar{\alpha}_1^2 \right)\bar{\beta}^2\frac{1}{T},\\
    &c_2=\frac{L_f +\frac{1}{2}}{2} + M_fL_{\m{y}} +\frac{L_{\m{yx}}M_f}{4\eta L_{\m{y}}}.
  %  & c_3= 24 
\end{aligned}
\end{equation}
Then telescoping gives
\begin{equation}\label{eqn:dec:final:bilevel}
\begin{aligned}
    \frac{1}{K}\sum_{k=0}^{K-1}\mb{E}[\|\nabla f(\m{x}^k)\|^2]
    &\leq \frac{4}{\sum_{k=0}^{K-1}\alpha_k} \left(\Delta_{\mb{W}} +\sum_{k=0}^{K-1} \frac{3}{2}\left(\alpha_k+ \frac{\alpha_k^2}{2}\right) b^2 + c_1\alpha_k^2\sigma_{g,1}^2 + c_2 \alpha_k^2\tilde{\sigma}_{f}^2\right)\\
    &\leq \frac{4\Delta_{\mb{W}} }{\min\{\bar\alpha_1, \bar\alpha_2,\bar\alpha_3\}K} + \frac{4\Delta_{\mb{W}} }{\bar\alpha\sqrt{K}} +6\left(1+ \frac{\bar\alpha}{2\sqrt{K}}\right) b^2 +  \frac{4c_1\bar\alpha}{\sqrt{K}}\sigma_{g,1}^2 + \frac{4c_2\bar\alpha}{\sqrt{K}}\tilde\sigma_{f}^2 \\
    &= {\cal O}\left(\frac{1}{\min\{\bar{\alpha}_1, \bar{\alpha}_2, \bar{\alpha}_3\}K}+ \frac{\bar{\alpha}\max(\sigma_{g,1}^2, \sigma_{g,2}^2,\sigma_f^2)}{\sqrt{K}} + b^2 \right),
\end{aligned}
\end{equation}
where $\Delta_{\mb{W}} := \mb{W}^0-\mb{E}[\mb{W}^K]$.
%This completes the proof.
\end{proof}

\subsection{Proof of Corollary~\ref{thm:fednest:bilevel}}
\begin{proof}
Let $\eta=\frac{M_f}{L_{\m{y}}}=\mc{O}(\kappa_g)$ in \eqref{eqn44:dec:lyap}. It follows from \eqref{eqn:lip:condi}, \eqref{eqn2:dec:lyap}, and \eqref{eqn44:dec:lyap} that  
%We can have
\begin{equation}
\bar\alpha_1=\mc{O}(\kappa^{-3}_g), ~~\bar\alpha_2=\mc{O}(T\kappa^{-3}_g),~~\bar\alpha_3=\mc{O}(\kappa^{-4}_g),~~ c_1=\mc{O}(\kappa^9_g/T), ~~c_2=\mc{O}(\kappa^3_g).
\end{equation}
Further,  $N=\mc{O}(\kappa_g\log K)$  gives $b=\frac{1}{K^{1/4}}$. Now, if we select $\bar\alpha=\mc{O}(\kappa^{-2.5}_g)$ and $T=\mc{O}(\kappa^4_g)$, Eq.~\eqref{eqn:dec:final:bilevel} gives
\begin{align*}
    \frac{1}{K}\sum_{k=0}^{K-1}\mb{E}[\|\nabla f(\m{x}^k)\|^2] = \mc{O}\left(\frac{\kappa^4_g}{K} + \frac{\kappa^{2.5}_g}{\sqrt{K}}\right).
\end{align*}
To achieve $\varepsilon$-optimal solution, we need $K=\mc{O}(\kappa^5_g\varepsilon^{-2})$, and the samples in  $\xi$ and $\zeta$ are $\mc{O}(\kappa^5_g\varepsilon^{-2})$ and $\mc{O}(\kappa^9_g\varepsilon^{-2})$, respectively.
\end{proof}






% \section{Proof for Stochastic Bilevel Problem}\label{sec:app:bilevel}
% Throughout the proof, we use ${\mc{F}}^{k,t}=\sigma\{\m{y}^0, \m{x}^0, \ldots, \m{y}^k, \m{x}^k, \m{y}^{k,1},\ldots, \m{y}^{k,t}\}$, ${\cal F}^k=\sigma\{\m{y}^0, \m{x}^0,\ldots, \m{y}^{k+1}\}$, where $\sigma\{\cdot\}$ denotes the $\sigma$-algebra generated by the random variables.  Further, we will use $\mathcal{F}^{k,t}_{i,\nu}$ to denote the filtration that captures all the randomness up to the $\ell$-th local step of client $i$ in inner round $t$ and outer round $k$. Throughout, we use the following notations
% \begin{equation}
%     \begin{aligned}
% \m{h} (\m{x}_{i,\nu}, \m{y}) &= \nabla_{\m{x}} f_i(\m{x}_{i,\nu}, \m{y}, \xi_{i,\nu})-\nabla^2_{\m{xy}}g_i(\m{x}_{i,\nu},\m{y};{\zeta}_{i,\nu})
%  \m{p}_N   \\
% \bar{\m{h}}_i (\m{x}_{i,\nu}, \m{y})&:=\mb{E}\left[\m{h}_i(\m{x}_{i,\nu}, \m{y})|{\cal F}_{i,\nu-1}\right],\\
% \bar{\m{h}} (\m{x}, \m{y})&:=\mb{E}\left[\m{h}(\m{x}, \m{y})|{\mc{F}}\right],\\
% &b:= \|\bar{\m{h}}(\m{x}, \m{y})- \bar{\nabla}f (\m{x}, \m{y})\|.
% \end{aligned}
% \label{eqn:basic:not}
% \end{equation}

% The following lemma extends \citep[Lemma 2.2]{ghadimi2018approximation} to the finite sum problem \eqref{fedblo:prob}. Proof follows similarly. 
% \begin{lemma}\label{lem:lips} 
% Under Assumption~\ref{assu:f}, we have
% \begin{subequations}\label{eqn:newlips}
% 		\begin{align}
% \|\bar{\nabla} f_i(\m{x},\m{y}) - \nabla f_i (\m{x},\m{y}^*(\m{x})) \|
% &	\leq  M_f\|\m{y}^*(\m{x})-\m{y}\|,~\textnormal{for all}~i \in \{1, \ldots, m\}, \label{eqn:newlips:a}\\
% \|\nabla f(\m{x}_1)-\nabla f(\m{x}_2)\|
% &	\leq  L_f\|\m{x}_1-\m{x}_2\|, \label{eqn:newlips:b}\\
% 	\|\m{y}^*(\m{x}_1)-\m{y}^*(\m{x}_2)\|&\leq  L_{\m{y}}\|\m{x}_1-\m{x}_2\|, \label{eqn:newlips:c}\\
% \|\nabla \m{y}^*(\m{x}_1)-\nabla \m{y}^*(\m{x}_2)\|&\leq  L_{\m{yx}}\|\m{x}_1-\m{x}_2\|. \label{eqn:newlips:d}
% \end{align}
% \end{subequations}
% Here, 
% \begin{align*}
% L_{\m{yx}}&:=\frac{\ell_{g,2}+\ell_{g,2}L_{\m{y}}}{\mu_g} + \frac{\ell_{g,1}(\ell_{g,2}+\ell_{g,2}L_{\m{y}})}{\mu_g^2},~~~L_{\m{y}} :=\frac{\ell_{g,1}}{\mu_g},\\
% M_f &:=\ell_{f,1} + \frac{\ell_{g,1}\ell_{f,1}}{\mu_g} + \frac{\ell_{f,0}}{\mu_g}\Big(\ell_{g,2}+\frac{\ell_{g,1}{\ell_{g,2}}}{\mu_g}\Big),~~~
% \\
% L_f&:=\ell_{f,1} + \frac{\ell_{g,1}(\ell_{f,1}+L_f)}{\mu_g} + \frac{\ell_{f,0}}{\mu_g}\Big(\ell_{g,2}+\frac{\ell_{g,1}{\ell_{g,2}}}{\mu_g}\Big),
% \end{align*}
% where   $\ell_{f,0}$, $\ell_{f,1}, \ell_{g,1}, \ell_{g,2}$, and $\mu_g$ are given in Assumption~\ref{assu:f}.
% \end{lemma}
% %
% \begin{lemma}[Bounded Variance]\label{lem:var:approx:boun}
% For $\bar{\m{h}}_i (\m{x}, \m{y})$ defined in \eqref{eqn:basic:not}, we have
% \begin{equation}
% \begin{aligned}
%     \mb{E}\left[\|\bar{\m{h}}_i (\m{x}, \m{y})- \m{h}_i(\m{x}, \m{y})\|^2\right] &\leq\sigma_f^2 + \frac{3}{\mu_g^2}\left[(\sigma_f^2+\ell_{f,0}^2)(\sigma_{g,2}^2+2\ell_{g,1}^2)+\sigma_f^2\ell_{g,1}^2\right]
%     \\
%     &=:\tilde\sigma_f^2.
% \end{aligned}
% \label{eqn:var:dec}
% \end{equation}
% \end{lemma}
% \begin{proof}
%     The proof is similar to 
% \end{proof}
% \subsection{Descent of Outer Objective}

% The following lemma characterizes the descent of outer objective.

% \begin{lemma}[Descent Lemma]\label{lem:dec}
% Suppose Assumptions~\ref{assu:f} holds. Further, assume $\tau_i \geq 1, \forall i\in\mathcal{S}$, and $\alpha_i=\frac{\alpha}{\tau_i}, \forall i \in \mathcal{S}$, where $\alpha\in (0,1)$. Then, \fedout guarantees:
% \begin{equation}
%     \begin{aligned}
% \mb{E}\left[f(\m{x}^{+})\right] - \mb{E}\left[f(\m{x})\right]& \leq  \left(24M_f^2+ 3\alpha^2\bar{L}^2_fL_f^2 \right) \frac{1}{m} \sum\limits_{m=1}^{M}   \frac{1}{\tau_i} \sum\limits_{k=0}^{K-1} \left[\|\m{x}_{i,\nu} -\m{x}\|^2\right]\\
% &+\alpha M_f^2 \mb{E}\left[\|\m{y}^+-\m{y}^*(\m{x})\|^2\right]- \frac{\alpha}{2} \mb{E}\left[\| \nabla f(\m{x})\|^2\right]\\
% &+8\alpha^2\tilde{\sigma}^2_f L_f + 24 \alpha  b^2 -\alpha (1- 2 L_f\alpha  ) \mb{E}\left[\|\bar{\m{h}}(\m{x},\m{y}^+)\|^2\right].
% \end{aligned}
% \label{eqn0:lem:dec}
% \end{equation}
% %Here, $M_f, L_f, \tilde{\sigma}_f$ are given in Lemma~\ref{eqn:newlips}; $b$ is defined in \eqref{eqn:basic:not}; and  ...
% %
% \end{lemma}
% %
% \begin{proof}
% It follows from  Algorithm~\ref{alg:fedout} that $\m{x}_{i,0}=\m{x}, \forall i\in\mathcal{S}$, and 
%  \begin{align}\label{eqn1:lem:dec}
%      \m{x}^{+}&=\m{x}-\frac{1}{m}  \sum\limits_{m=1}^{M} \alpha_i \sum\limits_{k=0}^{K-1} \m{h}_i(\m{x}_{i,\nu}, \m{y}^+).
%  \end{align}
% Now, using the Lipschitz property of $\nabla f$ in Lemma~\ref{lem:lips}, we have
% \begin{equation}
%     \begin{aligned}
% \mb{E}\left[f(\m{x}^{+}) |\mc{F}_{i,\nu-1} \right] 
%     &\leq f(\m{x}) + \mb{E} \left[\langle \m{x}^{+} - \m{x}, \nabla f(\m{x}) \rangle | \mc{F}_{i,\nu-1} \right] + \frac{L_f}{2} \mb{E} \left[{\Vert \m{x}^{+}-\m{x} \Vert}^2 | \mc{F}_{i,\nu-1} \right]\\
%     & = - \mb{E}\Big[ \underbrace{\big\langle \frac{1}{M}\sum\limits_{m=1}^{M} \alpha_i \sum\limits_{k=0}^{K-1} ( \m{h}_i(\m{x}_{i,\nu}, \m{y}^+) , \nabla f(\m{x}) \big\rangle}_{=:\mc{A}_1} | \mc{F}_{i,\nu-1}\Big] \\
%     &+ \frac{L_f}{2}  \mb{E}\Big[ \underbrace{\big\| \frac{1}{M}\sum\limits_{m=1}^{M} \alpha_i \sum\limits_{k=0}^{K-1} \m{h}_i(\m{x}_{i,\nu}, \m{y}^+)\big\|^2}_{=:\mc{A}_2} | \mc{F}_{i,\nu-1} \Big].\\
%     \end{aligned}
% \label{eqn2:lem:dec}
% \end{equation}
% %
% In the following, we bound each term in \eqref{eqn2:lem:dec}.

% \textbf{Bounding first term in \eqref{eqn2:lem:dec}}:
% \\
% For the first term on the right hand side (RHS) in~\eqref{eqn2:lem:dec}, we have
% \begin{equation}
% \label{eqn3:lem:dec}
%     \begin{aligned}
%       \mb{E}[\mathcal{A}_1|\mc{F}_{i,\nu-1}]&=- \big\langle \frac{1}{M}\sum\limits_{m=1}^{M} \alpha_i \sum\limits_{k=0}^{K-1} \bar{\m{h}}_i(\m{x}_{i,\nu},\m{y}^+), \nabla f(\m{x}) \big\rangle\\
%       &= - \Big \langle \frac{1}{M}\sum\limits_{m=1}^{M} \alpha_i \sum\limits_{k=0}^{K-1} \left( \bar{\m{h}}_i(\m{x}_{i,\nu},\m{y}^+)-\bar{\m{h}}_i(\m{x},\m{y}^+) \right) + \frac{1}{m} \sum\limits_{m=1}^{M} \alpha_i \sum\limits_{k=0}^{K-1} \bar{\m{h}}_i(\m{x},\m{y}^+), \nabla f(\m{x}) \Big \rangle \\
% &= - \Big \langle \frac{1}{m}\sum\limits_{i=1}^{m} \alpha_i \sum\limits_{k=0}^{K-1} \left( \bar{\m{h}}_i(\m{x}_{i,\nu},\m{y}^+)-\bar{\m{h}}_i(\m{x},\m{y}^+) \right) + \frac{1}{m} \sum\limits_{i=1}^{m} \underbrace{\alpha_i \tau_i}_{\alpha} \bar{\m{h}}_i(\m{x},\m{y}^+), \nabla f(\m{x}) \Big \rangle \\
% &=  \underbrace{-\Big \langle \frac{1}{m}\sum\limits_{i=1}^{m} \alpha_i \sum\limits_{k=0}^{K-1} \left( \bar{\m{h}}_i(\m{x}_{i,\nu},\m{y}^+)-\bar{\m{h}}_i(\m{x},\m{y}^+) \right), \nabla f(\m{x}) \Big \rangle}_{=:\mc{A}_{11}} - \alpha\underbrace{ \Big \langle \bar{\m{h}}(\m{x},\m{y}^+), \nabla f(\m{x}) \Big \rangle}_{=:\mc{A}_{12}}.
% \end{aligned}
% \end{equation}
% It follows from \eqref{eqn:Jens} that 
% \begin{equation}
% %\label{eqn3+:lem:dec}
% \begin{aligned}
% \mb{E}[\|\bar{\m{h}}_i(\m{x}_{i,\nu},\m{y}^+)-\bar{\m{h}}_i(\m{x},\m{y}^+)\|^2] &\leq  3 \mb{E}[ \|\bar{\m{h}}_i(\m{x}_{i,\nu},\m{y}^+)-\bar{\nabla}f _i(\m{x}_{i,\nu},\m{y}^+)\|^2+ 3 \|\bar{\nabla}f _i(\m{x}_{i,\nu},\m{y}^+) - \bar{\nabla}f _i(\m{x},\m{y}^+)\| \\
%     &+ 3\| \bar{\nabla}f _i(\m{x},\m{y}^+)-   \bar{\m{h}}_i(\m{x},\m{y}^+)\|^2]\\
%     & \leq 6b^2+ 3 M_f^2  \|\m{x}_{i,\nu} -\m{x}\|^2
% \end{aligned}   
% \end{equation}
% where the last inequality uses Lemma~\ref{eqn:newlips}.
 
% The above inequality together with Young's inequality, i.e., $ab\leq \gamma a^2+\frac{b^2}{4\gamma}$ implies that 
% \begin{equation}%\label{lemma12:eqn7}
% \begin{aligned}
% \mc{A}_{11} &\leq\frac{1}{2\alpha} \| \frac{1}{m} \sum\limits_{i=1}^{m} \alpha_i \sum\limits_{k=0}^{K-1}  \bar{\m{h}}_i(\m{x}_{i,\nu},\m{y}^+) -\bar{\m{h}}_i(\m{x},\m{y}^+) \|^2+ \frac{\alpha}{2} \|\nabla f(\m{x})\|^2\\
% &\leq  \frac{1}{2\alpha} \frac{1}{m} \sum\limits_{i=1}^{m} \alpha_i^2 \tau_i \sum\limits_{k=0}^{K-1} \| \bar{\m{h}}_i(\m{x}_{i,\nu},\m{y}^+) -\bar{\m{h}}_i(\m{x},\m{y}^+)  \|^2+ \frac{\alpha}{2}\|\nabla f(\m{x})\|^2\\
% &\leq 3 \alpha b^2+  \frac{3M_f^2}{2\alpha}\frac{1}{m} \sum\limits_{i=1}^{m} \alpha_i^2  \tau_i \sum\limits_{k=0}^{K-1} \|\m{x}_{i,\nu} -\m{x}\|^2 + \frac{\alpha}{2} \|\nabla f(\m{x})\|^2\\
% &=3\alpha  b^2+ \frac{ 3 \alphaM_f^2 }{2m} \sum\limits_{i=1}^{m}   \frac{1}{\tau_i} \sum\limits_{k=0}^{K-1}  \|\m{x}_{i,\nu} -\m{x}\|^2 + \frac{\alpha}{2} \|\nabla f(\m{x})\|^2.\\
% \end{aligned}
% \label{eqn4:lem:dec}
% \end{equation}
% Here, the last equality uses our assumption that $\alpha_i=\frac{\alpha}{\tau_i}, \forall i \in \mathcal{S}$, where $\alpha\in (0,1)$.

% Further, for the second term in RHS of \eqref{eqn3:lem:dec}, we have 
% \begin{equation}%\label{lemma12:eqn7}
% \begin{aligned}
% \mc{A}_{12}&=-\|\bar{\m{h}}(\m{x},\m{y}^+)\|^2- \| \nabla f(\m{x})\|^2+\|\bar{\m{h}}(\m{x},\m{y}^+)-\nabla f(\m{x})\|^2\\
%  & \leq -\|\bar{\m{h}}(\m{x},\m{y}^+)\|^2- \| \nabla f(\m{x})\|^2 +  2\|\bar{\nabla} f(\m{x},\m{y}^+)-\nabla f(\m{x})\|^2+ 2\|\bar{\m{h}}(\m{x},\m{y}^+)-\bar{\nabla} f(\m{x},\m{y}^+)\|^2 \\
%  & \leq -\|\bar{\m{h}}(\m{x},\m{y}^+)\|^2- \| \nabla f(\m{x})\|^2 + 2M_f\|\m{y}^+-\m{y}^*(\m{x})\|^2+ 2b^2,\\
% \end{aligned}
% \label{eqn5:lem:dec}
% \end{equation} 
% where the last inequality uses Lemmas~\ref{lem:lips} and \ref{lem:neum:bias}. 

% Substituting \eqref{eqn4:lem:dec} and \eqref{eqn5:lem:dec} in \eqref{eqn3:lem:dec} gives 
% \textbf{\begin{equation}%\label{lemma12:eqn7}
% \begin{aligned}
% \mb{E}\left[\mc{A}_{1}  | \mc{F}_{i,\nu-1} \right]&\leq \frac{ 3 \alpha M_f^2}{2m} \sum\limits_{i=1}^{m}   \frac{1}{\tau_i} \sum\limits_{k=0}^{K-1}  \|\m{x}_{i,\nu} -\m{x}\|^2 - \alpha \|\bar{\m{h}}(\m{x},\m{y}^+)\|^2\\
%  &- \frac{\alpha}{2}\| \nabla f(\m{x})\|^2 + 2 \alpha M_f \|\m{y}^+-\m{y}^*(\m{x})\|^2+ 5\alpha b^2,\\
% \end{aligned}
% \label{eqn5:lem:dec}
% \end{equation} }
% where we used our assumption that $\alpha \in (0,1)$.

% \noindent\textbf{Bounding second term in \eqref{eqn2:lem:dec}}:

% Observe that 
% \begin{equation}
%  \begin{aligned}
% \mc{A}_2 &=\norm[\bigg]{\frac{1}{m}\sum\limits_{i=1}^{m} \alpha_i \sum\limits_{k=0}^{K-1} ( \m{h}_i(\m{x}_{i,\nu}, \m{y}^+)-  \m{h}_i(\m{x}, \m{y}^+)) + \frac{1}{m} \sum\limits_{i=1}^{m} \alpha_i \sum\limits_{k=0}^{K-1}  \m{h}_i(\m{x}, \m{y}^+)}^2\\
%  &= \norm[\bigg]{\frac{1}{m}\sum\limits_{i=1}^{m} \alpha_i \sum\limits_{k=0}^{K-1} \left(   \m{h}_i(\m{x}_{i,\nu}, \m{y}^+) -  \m{h}_i(\m{x}, \m{y}^+)\right) + \alpha  \m{h}_i(\m{x}, \m{y}^+) }^2\\
% &  \leq 2 \underbrace{\norm[\bigg]{\frac{1}{m}\sum\limits_{i=1}^{m}\alpha_i \sum\limits_{k=0}^{K-1} \Big(  \m{h}_i(\m{x}_{i,\nu}, \m{y}^+) -  \m{h}_i(\m{x}, \m{y}^+) \Big)}^2}_{\mc{A}_{21}} + 2 {\alpha}^2 \underbrace{{\Vert \m{h}(\m{x}, \m{y}^+)\Vert}^2}_{\mc{A}_{22}},\\
% % & \overset{(b)} \leq \frac{1}{m}  \sum\limits_{i=1}^{m} {\alpha_i}^2 \norm[\bigg]{ \sum\limits_{k=0}^{K-1} \left(   \m{h}_i(\m{x}_{i,\nu}, \m{y}^+) -  \m{h}_i(\m{x}, \m{y}^+)  \right)}^2 + {\alpha}^2 L_f {\Vert  \m{h}^k  \Vert}^2\\
% % & \overset{(c)} \leq \frac{1 }{m}  \sum\limits_{i=1}^{m} {\alpha_i}^2 \tau_i \sum\limits_{k=0}^{K-1} {\Vert \m{h}_{i,\nu}^k -  \m{h}_i(\m{x}, \m{y}^+)  \Vert }^2 + {\alpha}^2 L_f {\Vert \m{h}^k  \Vert}^2 
% %& \overset{(d)} \leq \frac{\alpha L^3}{m}  \sum\limits_{i=1}^{m} \alpha_i \sum\limits_{k=0}^{K-1} {\Vert  x_{i,\nu}-\m{x}^{k} \Vert }^2 + {\alpha}^2 L {\Vert \nabla f(\m{x}^{k}) \Vert}^2.
%     \end{aligned}
% \label{eqn6:lem:dec}
% \end{equation}
% where the inequality follows from \eqref{eqn:Jens}. 

% For the first term in the RHS of \eqref{eqn6:lem:dec}, we have
% \begin{equation*}
% \begin{aligned}
%  \mc{A}_{21} &=\Big\|\dfrac{1}{m}\sum \limits_{i=1}^m \alpha_i \sum \limits_{k=0}^{K-1}( \m{h}_i(\m{x}_{i,\nu}, \m{y}^+)- \m{h}_i(\m{x}, \m{y}^+))\Big\|^2 \\
%       & {\leq} \dfrac{1}{m}\sum \limits_{i=1}^m  \alpha_i^2 \tau_i \sum \limits_{k=0}^{K-1}\| \m{h}_i(\m{x}_{i,\nu}, \m{y}^+)- \m{h}_i(\m{x}, \m{y}^+)\|^2\\
%         &= \dfrac{\alpha}{m}\sum \limits_{i=1}^m \alpha_i\sum \limits_{k=0}^{K-1}\| \m{h}_i(\m{x}_{i,\nu}, \m{y}^+)- \m{h}_i(\m{x}, \m{y}^+)\|^2.
%     %     &\leq \dfrac{3\alpha}{m}\sum \limits_{i=1}^m \alpha_i\sum \limits_{k=0}^{K-1}\Big(\| \m{h}_i(\m{x}_{i,\nu}, \m{y}^+)-\bar{\m{h}}_i(\m{x}_{i,\nu},\m{y}^+)\|^2\\
%     %     &+\|\bar{\m{h}}_i(\m{x}_{i,\nu},\m{y}^+)-\bar{\m{h}}_i(\m{x},\m{y}^+)\|^2+\|\bar{\m{h}}_i(\m{x},\m{y}^+)- \m{h}_i(\m{x}, \m{y}^+)\|^2\Big),
%     \end{aligned}
% \end{equation*}
% % Now, using \eqref{eqn:Jens}, we obtain
% % \begin{equation}\label{eqn7:lem:dec}
% % \begin{aligned}
% %         \mb{E}\left[ \mc{A}_{21} \right] &\leq \dfrac{3\alpha}{m}\sum \limits_{i=1}^m \alpha_i\sum \limits_{k=0}^{K-1} \Big( \mb{E}\left[\mb{E}\left[\| \m{h}_i(\m{x}_{i,\nu}, \m{y}^+)-\bar{\m{h}}_i(\m{x}_{i,\nu},\m{y}^+)\|^2| \mc{F}_{i,\nu-1}\right]\right]\\
% %      &\leq  \|\bar{\m{h}}_i(\m{x}_{i,\nu},\m{y}^+)-\bar{\nabla}f _i(\m{x}_{i,\nu},\m{y}^+)\|^2  +\|\bar{\nabla}f _i(\m{x}_{i,\nu},\m{y}^+) - \bar{\nabla}f _i(\m{x},\m{y}^+)\|^2
% %      \\
% %      &+\| \bar{\nabla}f _i(\m{x},\m{y}^+)-   \bar{\m{h}}_i(\m{x},\m{y}^+)\|^2
% %     +\mb{E}\left[\|\bar{\m{h}}_i(\m{x}_{i,\nu},\m{y}^+)-\bar{\m{h}}_i(\m{x},\m{y}^+)\|^2\right]
% %     \\
% %     &+\mb{E}\left[\mb{E}\left[\|\bar{\m{h}}_i(\m{x},\m{y}^+)- \m{h}_i(\m{x}, \m{y}^+)\|^2| \mc{F}\right]\right]\Big)\\
% %         & \leq 6\alpha^2\tilde{\sigma}^2_f+\dfrac{3\alpha \bar{L}^2_f}{m}\sum \limits_{i=1}^m \alpha_i\sum \limits_{k=0}^{K-1}\mb{E}\Big[\|\m{x}_{i,\nu}-\m{x}\|^2\Big],
% %     \end{aligned}
% % \end{equation}
% Now, using \eqref{eqn:Jens}, we obtain
% \begin{equation}\label{eqn7:lem:dec}
% \begin{aligned}
%         \mb{E}\left[ \mc{A}_{21} \right] &\leq \dfrac{6\alpha}{m}\sum \limits_{i=1}^m \alpha_i\sum \limits_{k=0}^{K-1} \Big( \mb{E}\Big[\| \m{h}_i(\m{x}_{i,\nu}, \m{y}^+)-\bar{\m{h}}_i(\m{x}_{i,\nu},\m{y}^+)\|^2\\ 
%      &+  \|\bar{\m{h}}_i(\m{x}_{i,\nu},\m{y}^+)-\bar{\nabla}f _i(\m{x}_{i,\nu},\m{y}^+)\|^2  +\|\bar{\nabla}f _i(\m{x}_{i,\nu},\m{y}^+) - \bar{\nabla}f _i(\m{x},\m{y}^+)\|^2
%      \\
%      &+\| \bar{\nabla}f _i(\m{x},\m{y}^+)-   \bar{\m{h}}_i(\m{x},\m{y}^+)\|^2
%     +\|\bar{\m{h}}_i(\m{x},\m{y}^+)- \m{h}_i(\m{x}, \m{y}^+)\|^2\Big]\\
%         & \leq 12 \alpha^2 b^2+ 12 \alpha^2\tilde{\sigma}^2_f+\dfrac{6\alpha \bar{L}^2_f}{m}\sum \limits_{i=1}^m \alpha_i\sum \limits_{k=0}^{K-1}\mb{E}\Big[\|\m{x}_{i,\nu}-\m{x}\|^2\Big],
%     \end{aligned}
% \end{equation}

% where the last inequality uses Lemma~\ref{lem:var:approx:boun}.

% Term $\mc{A}_{22}$ in \eqref{eqn6:lem:dec} can be upper bounded as follows:
% \begin{equation}
% \label{eqn8:lem:dec}
%     \begin{aligned}
%   \mc{A}_{22} & =  \|\m{h}_i(\m{x},\m{y}^+)-\bar{\m{h}}_i(\m{x},\m{y}^+)+\bar{\m{h}}_i(\m{x},\m{y}^+)\|^2\\
%                     &=\Big\|\dfrac{1}{m}\sum \limits_{i=1}^m (\m{h}_i(\m{x},\m{y}^+)-\bar{\m{h}}_i(\m{x},\m{y}^+)+\bar{\m{h}}_i(\m{x},\m{y}^+)\Big\|^2\\
%                     &\leq 2\Big\|\dfrac{1}{m}\sum \limits_{i=1}^m (\m{h}_i(\m{x},\m{y}^+)-\bar{\m{h}}_i(\m{x}^k))\Big\|^2+2\|\bar{\m{h}}(\m{x},\m{y}^+)\|^2\\
%                     &\leq \dfrac{2}{m}\sum \limits_{i=1}^m\|\m{h}_i(\m{x},\m{y}^+)-\bar{\m{h}}_i(\m{x},\m{y}^+)\|^2+ 2\|\bar{\m{h}}(\m{x},\m{y}^+)\|^2,
%     \end{aligned}
% \end{equation}
% where the inequalities use \eqref{eqn:Jens}. 

% Now, using Assumption~\ref{assu:bound:var}, we get
% \begin{align}
% &\mb{E}\left[\mc{A}_{22}\right]\leq 2\bigg(\tilde{\sigma}^2_f+\mb{E}\Big[\|\bar{\m{h}}(\m{x},\m{y}^+)\|^2\Big]\bigg).
%     \end{align}

% Substituting \eqref{eqn7:lem:dec} and \eqref{eqn8:lem:dec} in \eqref{eqn6:lem:dec} gives 
% \begin{equation}
% \label{eqn9:lem:dec}
% \begin{aligned}
%   \mb{E}\left[\mc{A}_2\mid\mc{F}_{i,\nu-1} \right] &\leq  L_f ( \mb{E}\left[\mc{A}_{21}\right] +  \alpha^2 \mb{E}\left[\mc{A}_{22}\right])\\
%   &= 2\alpha^2 L_f ( 6b^2+7\tilde{\sigma}^2_f)+2 \alpha ^2 L_f\mb{E}\Big[\|\bar{\m{h}}(\m{x},\m{y}^+)\|^2\Big]\\
%   &+ \dfrac{6\alpha \bar{L}^2_f L_f}{m}\sum \limits_{i=1}^m \alpha_i\sum \limits_{k=0}^{K-1}\mb{E}\Big[\|\m{x}_{i,\nu}-\m{x}\|^2\Big].
% \end{aligned}
% \end{equation}
% Plugging \eqref{eqn9:lem:dec} and \eqref{eqn5:lem:dec} into \eqref{eqn0:lem:dec}, and using the law of total expectation, complete the proof.
% \end{proof}

% %\subsection{Proof of Theorem~\ref{thm:fednest}}
% \subsection{Error of \fedinn}
% \subsubsection{Proof of Theorem~\ref{thm:fedin}}
% \begin{proof}
% The proof uses the idea of \cite{chen2021closing} for non-federated setting. Note that 
% \begin{align}\label{eqn-1:dec:fedin}
% \nonumber 
%  \mb{E}[\|\m{y}^{+}-\m{y}^*(\m{x}^{+})\|^2] =& \underbrace{ \mb{E}[\|\m{y}^{+}-\m{y}^*(\m{x})\|^2]}_{\mc{B}_1} + \underbrace{ \mb{E}[\|\m{y}^*(\m{x}^{+})-\m{y}^*(\m{x})\|^2]}_{\mc{B}_2} \\
% &\quad +2 \underbrace{ \mb{E}[\langle \m{y}^{+}-\m{y}^*(\m{x}), \m{y}^*(\m{x})-\m{y}^*(\m{x}^{+})\rangle]}_{\mc{B}_3}.
% \end{align}
% %
% Next, we upper bound each term in \eqref{eqn-1:dec:fedin}.

% \textbf{Bounding first term in \eqref{eqn-1:dec:fedin}}:\\
% By a similar argument as in \citep[Theorem~4]{mitra2021linear}, for all $t \in \{0,\ldots,T-1\}$, we obtain
% %\begin{subequations}
% \begin{equation*}%\label{eqn0-1:dec:fedin}
%     \mb{E}[{\Vert\m{y}^{t+1}- \m{y}^\star(\m{x})\Vert}^2] \leq \left(1-  \frac{{\beta} \mu_g}{2} \right) \mb{E}[{\Vert \m{y}^{t}- \m{y}(\m{x}^*) \Vert}^2] +25 {\beta}^2 \sigma^2_{g,1},
% \end{equation*}
% which implies that
% \begin{equation}\label{eqn0:dec:fedin}
%  \mc{B}_1 \leq \left(1-  \frac{{\beta} \mu_g}{2} \right)^T \mb{E}[{\Vert \m{y}- \m{y}(\m{x}^*) \Vert}^2] +25 T {\beta}^2 \sigma^2_{g,1}.
% \end{equation}
% %
% \textbf{Bounding second term in \eqref{eqn-1:dec:fedin}}:\\
% By similar steps as in \eqref{eqn6:lem:dec}--\eqref{eqn9:lem:dec}, we obtain
% \begin{equation}
% \begin{aligned}\label{eqn1:dec:fedin}
% \mc{B}_2 &\leq \frac{1}{L_{\m{y}}^2m^2}\mb{E}\left[\|\sum\limits_{i=1}^{m} \alpha_i \sum\limits_{k=0}^{K-1}  \m{h}_i(\m{x}, \m{y}^+)\|^2\right]  \leq  L_{\m{y}}^2 \mc{A}_2,
% %  L_{\m{y}}^2\alpha^2\mb{E}\left[\mb{E}\left[\|\m{h}(\m{x},\m{y}^+)-\bar{\m{h}}(\m{x},\m{y}^+) + \bar{\m{h}}(\m{x},\m{y}^+)\|^2|\mc{F}'\right]\right]\\
% % &\leq L_{\m{y}}^2 \alpha^2(\mb{E}[\|\bar{\m{h}}(\m{x},\m{y}^+)\|^2] + \tilde\sigma_f^2),
% \end{aligned}
% \end{equation}
% where the first inequality is obtained from Lemma~\ref{lem:neum:bias}.

% \textbf{Bounding third term in \eqref{eqn-1:dec:fedin}}:\\
% Observe that 
% \begin{equation}
% \label{eqn2:dec:fedin}
%     \begin{aligned}
% %\begin{align*}\label{eq.lemma2-new-pf-4-0}
%     \mb{E}[\mc{B}_3]
%     &= \underbrace{-\mb{E}[\langle\m{y}^+\!\!-\m{y}^\star(\m{x}), \nabla \m{y}^\star(\m{x})(\m{x}^+\!\!-\m{x})\rangle]}_{\mc{B}_{31}}\\
%     &\quad \underbrace{-\mb{E}[\langle\m{y}^+\!\!-\m{y}^\star(\m{x}), \m{y}^\star(\m{x}^+)-\m{y}^\star(\m{x})-\nabla \m{y}^\star(\m{x})(\m{x}^+\!\!-\m{x})\rangle]}_{\mc{B}_{32}}.
% \end{aligned}
% \end{equation}
% Let $\bar{\m{h}}(\m{x},\m{y}^+)=\mb{E}[\m{h}(\m{x},\m{y}^+)|{\mc{ F}}']$. We have
% \begin{equation}
% \label{eqn3:dec:fedin}
%     \begin{aligned}
% \mc{B}_{3,1}  =&-\mb{E}[\langle{\m{y}^+\!\!-\m{y}^\star(\m{x}), \mb{E}[\nabla \m{y}^\star(\m{x})(\m{x}^+\!\!-\m{x})\mid \mc{F}']\rangle}]\\
% =&-\mb{E}[\langle{\m{y}^+\!\!-\m{y}^\star(\m{x}), \mb{E}[\nabla \m{y}^\star(\m{x})(\m{x}^+\!\!-\m{x})]\rangle}]\\
% =&-\frac{1}{m}\mb{E}[\langle{\m{y}^+\!\!-\m{y}^\star(\m{x}),   \nabla \m{y}^\star(\m{x}) \sum\limits_{i=1}^{m} \alpha_i \sum\limits_{k=0}^{K-1} \bar{\m{h}}_i(\m{x}_{i,\nu},\m{y}^+) \rangle}]\\
%  \leq & \frac{1}{m}\mb{E}[\|\m{y}^+\!\!-\m{y}^\star(\m{x})\|  \|\nabla \m{y}^\star(\m{x})\sum\limits_{i=1}^{m} \alpha_i \sum\limits_{k=0}^{K-1} \bar{\m{h}}_i(\m{x}_{i,\nu},\m{y}^+)\|]\\
% \leq & \frac{1}{m}L_{\m{y}}\mb{E}[\|\m{y}^+\!\!-\m{y}^\star(\m{x})\|\|\sum\limits_{i=1}^{m} \alpha_i \sum\limits_{k=0}^{K-1} \bar{\m{h}}_i(\m{x}_{i,\nu},\m{y}^+)\|]
% \end{aligned}
% \end{equation}

% Note that
% \begin{equation}
%  \begin{aligned}
% \|\frac{1}{m}\sum\limits_{i=1}^{m} \alpha_i \sum\limits_{k=0}^{K-1} \bar{\m{h}}_i(\m{x}_{i,\nu},\m{y}^+)\|  &=\|\frac{1}{m}\sum\limits_{i=1}^{m} \alpha_i \sum\limits_{k=0}^{K-1} ( \bar{\m{h}}_i(\m{x}_{i,\nu}, \m{y}^+)-  \bar{\m{h}}_i(\m{x}, \m{y}^+)) + \frac{1}{m} \sum\limits_{i=1}^{m} \alpha_i \sum\limits_{k=0}^{K-1} \bar{\m{h}}_i(\m{x}, \m{y}^+)\|^2\\
% % &= \norm[\bigg]{\frac{1}{m}\sum\limits_{i=1}^{m} \alpha_i \sum\limits_{k=0}^{K-1} \left( \bar{\m{h}}_i(\m{x}_{i,\nu}, \m{y}^+) -  \bar{\m{h}}_i(\m{x}, \m{y}^+)\right) + \alpha \bar{\m{h}}_i(\m{x}, \m{y}^+) }^2\\
% &  \leq 4 \|\frac{1}{m}\sum\limits_{i=1}^{m} \alpha_i \sum\limits_{k=0}^{K-1} (\bar{\m{h}}_i(\m{x}_{i,\nu},\m{y}^+)-\bar{\nabla}f _i(\m{x}_{i,\nu},\m{y}^+))\|^2  \\
% &+4\|\frac{1}{m}\sum\limits_{i=1}^{m} \alpha_i \sum\limits_{k=0}^{K-1}(\bar{\nabla}f _i(\m{x}_{i,\nu},\m{y}^+) - \bar{\nabla}f _i(\m{x},\m{y}^+))\|^2\\
%      &+4\| \frac{1}{m}\sum\limits_{i=1}^{m} \alpha_i \sum\limits_{k=0}^{K-1} (\bar{\nabla}f _i(\m{x},\m{y}^+)-   \bar{\m{h}}_i(\m{x},\m{y}^+))\|^2 + 4{\alpha}^2 {\Vert \bar{\m{h}}(\m{x}, \m{y}^+)\Vert}^2\\ 
%     \end{aligned}
% %\label{eqn6:lem:dec}
% \end{equation}     
% which implies that      
% \begin{equation}
%  \begin{aligned}
% \mc{B}_{3,1}   &\leq \underbrace{8b^2 + 4{\alpha}^2 {\Vert \bar{\m{h}}(\m{x}, \m{y}^+)\Vert}^2+  \dfrac{\bar{L}^2_f}{m}\sum \limits_{i=1}^m \frac{\alpha_i}{\alpha}\sum \limits_{k=0}^{K-1}\mb{E}\Big[\|\m{x}_{i,\nu}-\m{x}\|^2\Big]}_{=:\mc{C}}
% % & \overset{(b)} \leq \frac{1}{m}  \sum\limits_{i=1}^{m} {\alpha_i}^2 \norm[\bigg]{ \sum\limits_{k=0}^{K-1} \left(   \m{h}_i(\m{x}_{i,\nu}, \m{y}^+) -  \m{h}_i(\m{x}, \m{y}^+)  \right)}^2 + {\alpha}^2 L_f {\Vert  \m{h}^k  \Vert}^2\\
% % & \overset{(c)} \leq \frac{1 }{m}  \sum\limits_{i=1}^{m} {\alpha_i}^2 \tau_i \sum\limits_{k=0}^{K-1} {\Vert \m{h}_{i,\nu}^k -  \m{h}_i(\m{x}, \m{y}^+)  \Vert }^2 + {\alpha}^2 L_f {\Vert \m{h}^k  \Vert}^2 
% %& \overset{(d)} \leq \frac{\alpha L^3}{m}  \sum\limits_{i=1}^{m} \alpha_i \sum\limits_{k=0}^{K-1} {\Vert  x_{i,\nu}-\m{x}^{k} \Vert }^2 + {\alpha}^2 L {\Vert \nabla f(\m{x}^{k}) \Vert}^2.
%     \end{aligned}
% \label{eqn6:lem:dec}
% \end{equation}

% % \begin{equation}
% % \label{eqn3:dec:fedin}
% %     \begin{aligned}
% % \mb{E}[\|\frac{1}{m}\sum\limits_{i=1}^{m} \alpha_i \sum\limits_{k=0}^{K-1} \bar{\m{h}}_i(\m{x}_{i,\nu},\m{y}^+)\|^2] \leq & \frac{ 2bL_{\m{y}}^2 \alpha^2 }{\gamma } 4 \mb{E}\Big[\|\bar{\m{h}}(\m{x},\m{y}^+)\|^2\Big]\\
% % &+ \frac{ 2bL_{\m{y}}^2 \alpha^2 }{\gamma }  \left( 2 b^2+\dfrac{\bar{L}^2_f}{m}\sum \limits_{i=1}^m \frac{\alpha_i}{\alpha}\sum \limits_{k=0}^{K-1}\mb{E}\Big[\|\m{x}_{i,\nu}-\m{x}\|^2\Big] \right)
% % \end{aligned}
% % \end{equation}
% Hence,
% \begin{equation}
% \label{eqn3:dec:fedin}
%     \begin{aligned}
% B_{3,1} \leq & \gamma\mb{E}[\|\m{y}^+\!\!-\m{y}^\star(\m{x})\|^2] + \frac{L_{\m{y}}^2 }{4\gamma } \mc{C},
% \end{aligned}
% \end{equation}
% where the inequality uses the Young's inequality such that $ab\leq \gamma a^2+\frac{b^2}{4\gamma}$.

% Using Lemma \ref{lem:lips}, we have 
% \begin{equation}
% \label{eqn4:dec:fedin}
% \begin{aligned}
% \mc{B}_{32} \leq & \mb{E}[\|\m{y}^+\!\!-\m{y}^\star(\m{x})\| \|\m{y}^\star(\m{x}^+)-\m{y}^\star(\m{x})-\nabla \m{y}^\star(\m{x})(\m{x}^+\!\!-\m{x})\|]\\
% \leq & \frac{L_{\m{yx}}}{2}\mb{E}\left[\|\m{y}^+\!\!-\m{y}^\star(\m{x})\|\|\m{x}^+\!\!-\m{x}\|^2\right]\\
% \leq & \frac{\eta L_{\m{yx}}}{4}\mb{E}\left[\|\m{y}^+\!\!-\m{y}^\star(\m{x})\|^2\mb{E}[\|\m{x}^+\!\!-\m{x}\|^2|{\mc{ F}}']\right]+ \frac{L_{\m{yx}}}{4\eta m^2}\mb{E}\left[\mb{E}[\|\sum\limits_{i=1}^{m} \alpha_i \sum\limits_{k=0}^{K-1} \bar{\m{h}}_i(\m{x}_{i,\nu},\m{y}^+)\|^2|{\mc{F}}']\right]\\
% \leq & \frac{\eta L_{\m{yx}}\tilde{D}_f^2\alpha^2}{4}\mb{E}[\|\m{y}^+\!\!-\m{y}^\star(\m{x})\|^2] + \frac{L_{\m{yx}}}{4\eta}\mc{A}_2
% \end{aligned}
% \end{equation}
% where the last inequality is due to the fact that $\mb{E}[\|\m{h}(\m{x},\m{y}^+)\|^2|{\mc{ F}}']\leq  \tilde{C}_f^2$ and the variance bound in Lemma \ref{lem:neum:bias}.

% Plugging \eqref{eqn4:dec:fedin} and \eqref{eqn3:dec:fedin} into \eqref{eqn2:dec:fedin}, we have
% \begin{equation}
% \label{eqn5:dec:fedin}
%     \begin{aligned}
%     \mb{E}[\mc{A}_3]
%     &\leq\left(\gamma + \frac{\eta L_{\m{yx}}\tilde{D}_f^2}{4}\alpha^2\right)\mb{E}[\|\m{y}^+\!\!-\m{y}^\star(\m{x})\|^2] \\
%     &+ \left(\frac{L_{\m{y}}^2}{4\gamma}+\frac{L_{\m{yx}}}{4\eta}\right)\mb{E}\left[\|\bar{\m{h}}(\m{x},\m{y}^+)\|^2\right]\\
%     &+
% \end{aligned}
% \end{equation}

% \noindent\textbf{Completing the proof of Theorem~\ref{thm:fedin}}:\\
% Plugging \eqref{eqn5:dec:fedin}, \eqref{eqn0:dec:fedin} into \eqref{eqn-1:dec:fedin}, we get
% \begin{equation}
% \label{eqn6:dec:fedin}
%     \begin{aligned}
%     \mb{E}[\|\m{y}^+-\m{y}^\star(\m{x}^+)\|^2]&\leq c_1 \mb{E}[\|\bar{\m{h}}(\m{x},\m{y}^+)\|^2]+ c_2 \mb{E}[\|\m{y}^+-\m{y}^\star(\m{x})\|^2] + \\
%     &\frac{c_3}{m}\sum \limits_{i=1}^m \alpha_i\sum \limits_{k=0}^{K-1}\mb{E}\Big[\|\m{x}_{i,\nu}-\m{x}\|^2\Big] + c_4 \tilde\sigma_f^2 +c_5 b^2 
% \end{aligned}
% \end{equation}
% where  
% \begin{align*}
%     c_{1}= \gamma + \frac{\alpha L_{\m{yx}}\tilde{C}_f^2}{4}\alpha^2,~~~  c_{2}=\frac{L_{\m{y}}^2\alpha^2}{4\gamma}+\frac{L_{\m{yx}}\alpha^2}{4\alpha},~~~c_{3}=\frac{L_{\m{yx}}\alpha^2}{4\alpha}, ~~~c_4 = 12 \alpha^2,~~~c_5 = 16 \alpha^2 
% \end{align*} 
% This completes the proof.
% \end{proof}

% \subsection{Drifting Errors of \fedout }
% The following lemma provides a bound on the \textit{drift} of each $\m{x}_{i,\nu}$ from $\m{x}$.=

% \begin{lemma}[Drifting Error of \fedout]\label{thm4:lemma2}
% Suppose Assumptions~\ref{assu:f}-\ref{assu:bound:var} holds. Let $\alpha_i\leq \frac{\alpha}{M_f\tau_i}$ for each $i \in \mathcal{S}$ and $\alpha \in (0,1)$. Then, $\forall \nu \in\{0,\ldots, \tau_i-1\}$,  \fedout guarantees:
% \begin{align}\label{eqn1:lemm:drift}
%  \mb{E}\left[\|\m{x}_{i,\nu}-\m{x}\|^2 \mid\mathcal{F}_{i,\nu-1} \right]\leq 20  \tau_i^2 \alpha_i^2  \mb{E}\left[\|\bar{\nabla} f(\m{x}, \m{y})\|^2 \mid \mathcal{F}_{i,\nu-1}\right]+ 45  \tau_i^2 \alpha_i^2  (\tilde{\sigma}_f^2 +2b^2).
% \end{align}
% \end{lemma}
% \begin{proof}
% The result trivially holds for $\tau_i=1$. Let $\tau_i>1$ and define
% \begin{align*}
% \m{v}_{i,\nu}&:= \bar{\m{h}}_i(\m{x}_{i,\nu}, \m{y})- \bar{\nabla} f_i(\m{x}_{i,\nu}, \m{y})- \bar{\m{h}}_i(\m{x},\m{y}) +\bar{\nabla} f_i(\m{x}, \m{y}) +\bar{\m{h}}(\m{x},\m{y}) -\bar{\nabla} f(\m{x}, \m{y}),\\
% \m{w}_{i,\nu}&:= \m{h}_i(\m{x}_{i,\nu}, \m{y})-\bar{\m{h}}_i(\m{x}_{i,\nu},\m{y})+\bar{\m{h}}_i(\m{x},\m{y})-\m{h}_i(\m{x},\m{y})+\m{h}(\m{x},\m{y})-\bar{\m{h}} (\m{x},\m{y}),\\
% \m{z}_{i,\nu}&:=\bar{\nabla} f_i(\m{x}_{i,\nu}, \m{y}) - \bar{\nabla} f_i(\m{x}, \m{y})+  \bar{\nabla} f(\m{x}, \m{y}).
% \end{align*}
% It follows from Step~7 in Algorithm~\ref{alg:fedout} that  
% \begin{equation}
% \begin{aligned}
%         \m{x}_{i,\nu+1}-\m{x}&=(\m{x}_{i,\nu}-\m{x})-\alpha_i (\m{v}_{i,\nu}-\m{w}_{i,\nu}+\m{z}_{i,\nu}),
%     \end{aligned}
% \end{equation}
% which implies that 
% \begin{equation}\label{eqn2:lemm:drift}
% \begin{aligned}
% \mb{E}\big[\|\m{x}_{i,\nu+1}-\m{x}\|^2\big]
% &=\mb{E}\big[\|(\m{x}_{i,\nu}-\m{x}-\alpha_i (\m{v}_{i,\nu}+\m{z}_{i,\nu})\|^2\big]+\alpha_i^2\mb{E}\big[\|{\m{w}_{i,\nu}}\|^2\big]\\&-2\mb{E}\bigg[\mb{E}\Big[\langle \m{x}_{i,\nu}-\m{x}-\alpha_i(\m{v}_{i,\nu}+\m{z}_{i,\nu}),\alpha_i \m{w}_{i,\nu} \rangle|\mathcal{F}_{i,\nu-1}\Big]\bigg] \\ 
% &= \mb{E}\big[\|\m{x}_{i,\nu}-\m{x}-\alpha_i(\m{v}_{i,\nu}+\m{z}_{i,\nu})\|^2\big]+\alpha_i^2\mb{E}\big[\|\m{w}_{i,\nu}\|^2\big].
% \end{aligned}
% \end{equation}
% Here, last equality uses the fact that $\mb{E}[\m{w}_{i,\nu}|\mathcal{F}_{i,\nu-1}]=0$.

% Observe that 
% \begin{equation}
% \label{eqn3:lemm:drift}
% \begin{aligned}
% \mb{E}\Big[\|\m{v}_{i,\nu}\|^2\Big]  &\leq 3  \mb{E}\Big[ \| \m{h}_i(\m{x}_{i,\nu}, \m{y})-\bar{\m{h}}_i(\m{x}_{i,\nu},\m{y}) \|^2 +\|\bar{\m{h}}_i(\m{x},\m{y})-\m{h}_i(\m{x},\m{y})\|^2+\|\m{h}(\m{x},\m{y})-\bar{\m{h}} (\m{x},\m{y})\|^2 \Big]\\
% &\leq  9 b^2,\\
% \mb{E}\Big[\|\m{w}_{i,\nu}\|^2\Big] &\leq 3   \mb{E}\Big[ \|\m{h}_i(\m{x}_{i,\nu},\m{y})-\bar{\m{h}}_i(\m{x}_{i,\nu},\m{y})\|^2+\|\bar{\m{h}}_i(\m{x})-\m{h}_i(\m{x},\m{y})\|^2+\|\m{h}(\m{x},\m{y})-\bar{\m{h}} (\m{x},\m{y})\|^2\Big]\\
%         & \leq 9\tilde{\sigma}_f^2.
%     \end{aligned}
% \end{equation}

% First term in the RHS of \eqref{eqn2:lemm:drift} can be bounded as follows:
% \begin{equation}
% \label{eqn4:lemm:drift}
% \begin{aligned}
% \mb{E}\big[\|\m{x}_{i,\nu+1}-\m{x}\|^2\big] &\leq  (1+\frac{1}{2\tau_i-1})\mb{E}\Big[\|\m{x}_{i,\nu}-\m{x}\|^2\Big]+ 2\tau_i \mb{E}\Big[\|\alpha_i (\m{v}_{i,\nu}+\m{z}_{i,\nu})\|^2\Big]\\
%  &\leq  (1+\frac{1}{2\tau_i-1})\mb{E}\Big[\|\m{x}_{i,\nu}-\m{x}\|^2\Big]+ 2\tau_i \alpha_i^2 \mb{E}\Big[\| \m{z}_{i,\nu}\|^2\Big] + 18 \tau_i \alpha_i^2 b^2 \\
%      % &\leq  (1+\frac{1}{2\tau_i-1})\mb{E}\Big[\|\m{x}_{i,\nu}-\m{x}\|^2\Big]+ 2\tau_i \mb{E}\Big[\|\alpha_i( \bar{\nabla} f_i(\m{x}_{i,\nu}, \m{y})-\bar{\nabla} f_i(\m{x},\m{y}))-\alpha_i \bar{\nabla} f(\m{x},\m{y})\|^2\Big] +\\
% %       &\leq  (1+\frac{1}{2\tau_i-1})\mb{E}\Big[\|\m{x}_{i,\nu}-\m{x}\|^2\Big]+ 10 \tau_i \alpha_i^2M_f^2\mb{E}\Big[\|\m{x}_{i,\nu}-\m{x}\|\Big]+ 10\tau_i \alpha_i^2  \mb{E}\Big[\|\bar{\nabla} f(\m{x},\m{y})\|^2\Big] + 10b^2  \\
%       &\leq  (1+\frac{1}{2\tau_i-1}+4\tau_i \alpha_i^2 M_f^2)\mb{E}\Big[\|\m{x}_{i,\nu}-\m{x}\|^2\Big]+4\tau_i \alpha_i^2  \mb{E}\Big[\|\bar{\nabla} f(\m{x},\m{y})\|^2\Big]+18 \tau_i \alpha_i^2 b^2,
%     \end{aligned}
% \end{equation}
% where the inequality follows from \eqref{eqn:Jens} and Lemma~\ref{lem:lips}.

% Substituting \eqref{eqn4:lemm:drift} and \eqref{eqn3:lemm:drift} into \eqref{eqn2:lemm:drift} gives 
% \begin{equation}
% \label{eqn5:lemm:drift}
%     \begin{aligned}
%         \mb{E}\big[\|\m{x}_{i,\nu+1}-\m{x}\|^2\big]&\leq (1+\frac{1}{2\tau_i-1}+4\tau_i \alpha_i^2 M_f^2)\mb{E}\Big[\|\m{x}_{i,\nu}-\m{x}\|^2\Big]\\
%       & +4\tau_i \alpha_i^2  \mb{E}\Big[\|\bar{\nabla} f(\m{x},\m{y})\|^2\Big]+ 9 \tau_i \alpha_i^2 (\tilde{\sigma}_f^2 +2b^2)\\
%         &\leq (1+\frac{1}{\tau_i-1})\mb{E}\Big[\|\m{x}_{i,\nu}-\m{x}\|^2\Big] \\
%         &+ 4 \tau_i \alpha_i^2  \mb{E}\Big[\|\bar{\nabla} f(\m{x},\m{y})\|^2\Big]+ 9 \tau_i \alpha_i^2 (\tilde{\sigma}_f^2 +2b^2),\\
%     \end{aligned} 
% \end{equation}
% where the last inequality follows by noting $\alpha_i\leq \frac{1}{M_f\tau_i}$. 

% Let 
% $$
% \eta_l = \sum \limits_{j=0}^{\ell-1} \eta_{i}^j~~\textnormal{where}~~\eta_{i}:=1+\frac{1}{\tau_i-1}.
% $$
% Since $\tau_i>1$, we have 
% \begin{equation*}
%   \eta_l  =\frac{\eta^{\ell}_i-1}{\eta_i-1} \leq 5 (\tau_i-1).
% \end{equation*}
% Now, iterating equation \eqref{eqn5:lemm:drift} and using $\m{x}_{i,0}=\m{x}$, we obtain:
% % Here,  the last inequality follows since $\tau_i>1$, and 
% % \begin{equation}
% %     \sum\limits_{j=0}^{\ell-1} \eta^j_i  =\frac{\eta^{\ell}_i-1}{\eta_i-1} \leq 5 (\tau_i-1),~~\textnormal{where}~~~\eta_i=1+\frac{1}{\tau_i-1}.
% % \end{equation}
% This completes the proof.
% % \begin{equation}
% %   \begin{aligned}
% % \Vert \m{x}_{i,\nu} - \m{x} \Vert & \leq 3 \eta^{\ell}_i \underbrace{\Vert \m{x}_{i,0} - \m{x} \Vert}_{= 0} + \left(\sum\limits_{j=0}^{\ell-1}\eta^j_i \right) \eta_i \Vert \bar{\nabla} f (\m{x},\m{y}) \Vert \\
% % &= \left(\sum\limits_{j=0}^{\ell-1} \eta^j_i \right) \eta_i \Vert \bar{\nabla} f (\m{x},\m{y}) \Vert \\
% % & = \left(\frac{\eta^{\ell}_i-1}{\eta_i-1}\right)\eta_i \Vert \bar{\nabla} f (\m{x},\m{y}) \Vert\\
% % & \leq \eta_i \tau_i {\left(1+\frac{1}{\tau_i} \right)}^{\ell} \Vert \bar{\nabla} f (\m{x},\m{y}) \Vert \\
% % & \leq \eta_i \tau_i {\left(1+\frac{1}{\tau_i} \right)}^{\tau_i} \Vert \bar{\nabla} f (\m{x},\m{y}) \Vert \\
% % & \leq \exp{(1)} \eta_i \tau_i \Vert \bar{\nabla} f (\m{x},\m{y}) \Vert \leq 3 \eta_i \tau_i \Vert \bar{\nabla} f (\m{x},\m{y}) \Vert,
% %     \end{aligned}  
% % \end{equation}
% %which is the desired conclusion.
% \end{proof}

% % \begin{lemma}\label{eq:lem:inn1} Suppose Assumptions~\ref{assu:f} and \ref{assu:bound:var} hold. Moreover, suppose $\tau_i\geq 1,\forall i\in\mathcal{S}$. For each $i\in\mathcal{S}$, let  $\beta_i^{k,t}=\frac{\beta^{k,t}}{\tau_i}$, where $\beta^{k,t}\in (0,1)$ satisfies $\beta^{k,t}  
% % < \frac{1}{6\ell_{g,1}}$ ($\beta^{k,t}  
% % < \frac{2}{\ell_{g,1} +\mu_g}$). Then, \fedinn guarantees:
% % \begin{equation}
% %     \mb{E}[{\Vert\m{y}^{k,t+1}- \m{y}^\star(\m{x}^k)\Vert}^2] \leq \left(1-  \frac{\bar{\beta} \mu_g}{2} \right) \mb{E}[{\Vert \m{y}^{k,t}- \m{y}^{k} (\m{x}^*) \Vert}^2] +25 \bar{\beta}^2 \sigma^2_{g,1}.
% % \end{equation}
% % \begin{proof}
% % \end{proof}
% % \end{lemma}

% % \begin{lemma}\label{eq:lem:inn2} 
% %  Under Assumptions~\ref{assu:f} and \ref{assu:bound:var}, we have
% % \begin{equation}
% % \mb{E}[\|\m{y}^*(\m{x}^{k+1})-\m{y}^*(\m{x}^k)\|^2] \leq   L_{\m{y}}^2\alpha_k^2(\mb{E}[\|\bar{\m{h}}(\m{x},\m{y}^+)\|^2] + \tilde\sigma_f^2).
% % \end{equation}
% % \begin{proof}

% % \end{proof}
% % \end{lemma}

% % \begin{lemma}\label{eq:lem:inn3} 
% %  Under Assumptions~\ref{assu:f} and \ref{assu:bound:var}, we have
% % \begin{align*} 
% % \langle \m{y}^{k+1}-\m{y}^*(\m{x}^k), \m{y}^*(\m{x}^k)-\m{y}^*(\m{x}^{k+1})\rangle &\leq c_{1,k}\mb{E}[\|y^{k+1}\!\!-\m{y}^\star(\m{x})\|^2]+ c_{2,k}\mb{E}[\|\bar{\m{h}}(\m{x},\m{y}^+)\|^2] + c_{3,k}\tilde\sigma_f^2.
% % \end{align*}
% % where 
% % \begin{align*}
% %     c_{1,k}= \gamma_k + \frac{\alpha L_{\m{yx}}\tilde{C}_f^2}{4}\alpha_k^2,~~~  c_{2,k}=\frac{L_{\m{y}}^2\alpha_k^2}{4\gamma_k}+\frac{L_{\m{yx}}\alpha_k^2}{4\alpha},~~~c_{3,k}=\frac{L_{\m{yx}}\alpha_k^2}{4\alpha}.
% % \end{align*}
% % \end{lemma}

% % \begin{proof}

% % \end{proof}

% % \begin{lemma}[Descent of outer problem]\label{lem:dec}
% % Suppose Assumption \ref{assu:f}-\ref{assu:bound:var} hold. Let $\bar{h}_f^k:=\mb{E}[h_f^k|x^k, y^{k+1}]$ Then, \fedout guarantees
% %  \begin{align}\label{eq.lemma3}
% %  \mb{E}[f(\m{x}^{k+1})]- \mb{E}[f(\m{x}^k)] \leq&- \frac{\alpha_k}{2} \mb{E}[\|\nabla f(x^k)\|^2] - \left(\frac{\alpha_k}{2}-\frac{L_f\alpha_k^2}{2}\right) \mb{E}[\|\bar{h}_f^k\|^2]\nn\\
% %     &+ L_f^2\alpha_k\mb{E}[\|y^{k+1}-\m{y}^\star(x^k)\|^2] + \alpha_k \|\bar{h}_f^k-\overline{\nabla}f(x^k,y^{k+1})\|^2+ \frac{L_f\alpha_k^2}{2}\tilde\sigma_f^2
% % \end{align} 
% % where constants $L_f, L_f, \sigma_f^2$ are defined in  Lemma~\ref{eqn:newlips}.
% % \end{lemma}

% % outer direction $\m{h}$ inner $\m{p}$

% \subsection{Proof of Theorem ~\ref{thm:fednest}}
% \begin{proof}
% Let  
% \begin{equation}\label{eqn4:dec:fedin}
% \begin{aligned}
% % C_1= \Big(\frac{\alpha_k}{2}-\frac{L_F\alpha_k^2}{2}-\frac{L_f}{L_{\m{y}}} L_{\m{y}}^2\alpha_k^2- \frac{L_f}{L_{\m{y}}}\frac{\alpha_k^2L_{\m{y}}^2}{4\gamma_k}-\frac{L_f}{L_{\m{y}}}\frac{L_{y\m{x}}\alpha_k^2}{4\eta}\Big) \\
% % C_3 =\frac{L_f}{L_\m{y}}\Big(1 + \gamma_k + L_fL_\m{y}\alpha_k + \frac{\eta L_{\m{y}\m{x}}\tilde{C}_f^2}{4}\alpha_k^2 \Big)
% \\
% C_1&= \frac{\alpha_k}{2}-\frac{L_F\alpha_k^2}{2}-\frac{L_f}{L_\m{y}} L_\m{y}^2\alpha_k^2- \frac{L_f}{L_\m{y}} \frac{\alpha_k^2L_\m{y}^2}{4\gamma_k}-\frac{L_f}{L_\m{y}} \frac{L_{\m{y}\m{x}}\alpha_k^2}{4\eta},\\
% C_2&= \frac{L_f}{L_\m{y}}\Big(\big(1 + \gamma_k + L_fL_\m{y}\alpha_k + \frac{\eta L_{\m{y}\m{x}}\tilde{C}_f^2}{4}\alpha_k^2 \big)(1-\rho_g\beta_k)^T -1\Big),\\
% C_3&= \frac{L_f}{L_\m{y}}\Big(\big(1 + \gamma_k + L_fL_\m{y}\alpha_k + \frac{\eta L_{\m{y}\m{x}}\tilde{C}_f^2}{4}\alpha_k^2 \big)(1-\rho_g\beta_k)^T -1\Big),\\
% C_4&= \frac{L_F}{2} + \frac{L_f}{L_\m{y}} L_\m{y}^2 + \frac{L_f}{L_\m{y}}\frac{L_{\m{y}\m{x}}}{4\eta},\\
% C_5&=..\\
% C_6&= \frac{L_F}{2} + \frac{L_f}{L_\m{y}} L_\m{y}^2 + \frac{L_f}{L_\m{y}}\frac{L_{\m{y}\m{x}}}{4\eta},
% \end{aligned}
% \end{equation}
% Then, 
% % We bound the two difference terms in \eqref{eq.diff-Lya} and obtain
% \begin{align*}%\label{eq.thm1-pf-1}
%   \mb{E}[\mb{W}^{k+1}] - \mb{E}[\mb{W}^k] & \leq      - \frac{\alpha_k}{2}\mb{E}[\|\nabla f(\m{x}^k)\|^2] - C_1\mb{E}[\|\bar{\m{h}}(\m{x}^k,\m{y}^{k+1}\|^2] \\
%   &+C_2 \mb{E}[\|\m{y}^k-\m{y}^*(\m{x}^k)\|^2] + \frac{C_3}{m}\sum \limits_{i=1}^m \alpha_i\sum \limits_{k=0}^{K-1}\mb{E}\Big[\|\m{x}_{i,\nu}^k-\m{x}^k\|^2\Big]\\
% %   \leq    &- \frac{\alpha_k}{2}\mb{E}[\|\nabla F(\m{x}^k)\|^2] - C_1 \mb{E}[\|\bar{h}_f^k\|^2]\\
% %     &+ \frac{L_f}{L_\m{y}}\Big(1 + \gamma_k + L_fL_\m{y}\alpha_k + \frac{\eta L_{\m{y}\m{x}}\tilde{C}_f^2}{4}\alpha_k^2 \Big)\mb{E}[\|\m{y}^{k+1}-\m{y}^*(\m{x}^k)\|^2]-\frac{L_f}{L_\m{y}}\mb{E}[\|\m{y}^k-\m{y}^*(\m{x}^k)\|^2]\\
% %     &+ \alpha_kb_k^2 + \Big(\frac{L_F}{2} + \frac{L_f}{L_\m{y}} L_\m{y}^2 +   \frac{L_f}{L_\m{y}}\frac{L_{\m{y}\m{x}}}{4\eta}\Big)\alpha_k^2\tilde\sigma_f^2\\
%     &  C_4 \alpha_k^2\tilde\sigma_f^2+  C_5 \alpha_kb_k^2+  C_6 T\beta_k^2\sigma_{g,1}^2 +\\
% \end{align*}

% To guarantee the descent of $\mb{W}^k$, we set ...


% \begin{align*}
%     \frac{1}{K}\sum_{k=0}^{K-1}\mb{E}[\|\nabla f(\m{x}^k)\|^2] = \mc{O}\left(\frac{\kappa^3}{K} + \frac{\kappa^{2.5}}{\sqrt{K}}\right).
% \end{align*}
% \end{proof}

% \section{Proof for Stochastic Min-Max Problems}\label{sec:app:minmax}
% %
% %

% \section{Proof for Compositional Problems}\label{sec:app:minmax}
% %

% %\subsection{Stochastic}
% \section{Deterministic}
% \begin{lemma}[Descent Lemma]Suppose Assumptions~\ref{assu:f} holds. Further, assume $\tau_i \geq 1, \forall i\in\mathcal{S}$, and $\alpha_i=\frac{\alpha}{\tau_i}, \forall i \in \mathcal{S}$, where $\alpha\in (0,1)$. Then, \fedblo guarantees:
% \begin{equation}
% \begin{aligned}
% \nonumber     
% f(\m{x}^{k+1}, \m{y}^\star(\m{x}^{k+1}))-f(\m{x}^{k}, \m{y}^\star(\m{x}^{k})) &\leq 
% \\
% \\
% -\alpha \left(1-\alpha L\right){\Vert \nabla f(\m{x}^{k},\m{y}^\star(\m{x}^{k})) \Vert}^2 \\
% \nonumber 
% &+ \left(\frac{L}{m} \sum\limits_{i=1}^{m} \alpha_i \sum\limits_{k=0}^{K-1}\Vert x_{i,\nu} - \m{x}^{k} \Vert \right) \Vert \nabla f(\m{x}^{k},\m{y}^\star(\m{x}^{k})) \Vert\\ 
% & \hspace{5mm} + \frac{\alpha L^3 }{m} \sum\limits_{i=1}^{m} \alpha_i  \sum\limits_{k=0}^{K-1}{\Vert x_{i,\nu} - \m{x}^{k} \Vert}^2 + \frac{\alpha L^3 }{m} \sum\limits_{i=1}^{m} \alpha_i  \sum\limits_{k=0}^{K-1}{\Vert \Delta_{i,l} \Vert}^2.
% \end{aligned}
% \label{eqn:f_bound_ct}
% \end{equation}
% \label{lemma:f_bound_ct}
% \end{lemma}


% \begin{proof}
% Using the fact that $\m{x}_{i,0}=\m{x}^k, \forall i\in\mathcal{S}$, we have:
% \begin{equation}
% \begin{aligned}
%     x_{i,\tau_i}&=\m{x}^{k}-\alpha_i\sum\limits_{k=0}^{K-1} \nabla_x f_i(x_{i,\nu}, \m{y}^{t+1}) -\alpha_i \tau_i (\wh{\nabla} f(\m{x}^{k}, \m{y}^{t+1}) - \nabla_x f_i(\m{x}^{k},\m{y}^{t+1}))\\
%     &=\m{x}^{k}-\alpha_i\sum\limits_{k=0}^{K-1}\nabla_x f_i(x_{i,\nu},\m{y}^{t+1}) - \alpha \left(\nabla_x f(\m{x}^{k},\m{y}^{t+1}) - \nabla_x f_i(\m{x}^{k},\m{y}^{t+1}) + \bar{\nabla} f(\m{x}^{k},\m{y}^{t+1}) \right), 
% \end{aligned}
% \end{equation}
% where we used $\alpha_i \tau_i =\alpha$ in the second step. Averaging the above iterates across clients, we obtain: 
% \begin{equation}
% \begin{aligned}
%     \m{x}^{k+1}=\frac{1}{m}\sum\limits_{i=1}^{m}x_{i,\tau_i}&=\m{x}^{k}-\frac{1}{m} \sum\limits_{i=1}^{m} \alpha_i \sum\limits_{k=0}^{K-1} \nabla_x f_i(x_{i,\nu},\m{y}^{t+1}) \\
%     & -\frac{\alpha}{m} \sum\limits_{i=1}^{m} \left(\nabla_x f(\m{x}^{k},\m{y}^{t+1}) - \nabla_x f_i(\m{x}^{k},\m{y}^{t+1}) + \bar{\nabla} f(\m{x}^{k},\m{y}^{t+1})\right)\\  
%     &=\m{x}^{k}-\frac{1}{m}  \sum\limits_{i=1}^{m} \alpha_i \sum\limits_{k=0}^{K-1} \nabla_x f_i(x_{i,\nu},\m{y}^{t+1} )  -\alpha \bar{\nabla} f(\m{x}^{k},\m{y}^{t+1}) ,
% \label{eqn:xbart_ct}
% \end{aligned}
% \end{equation}
% where for the second equality, we used the fact that $\nabla f(y) = \frac{1}{m} \sum\limits_{i=1}^{m} \nabla f_i(\cdot)$. 
% Based on the $L$-smoothness of $f(\cdot)$ and \eqref{eqn:xbart_ct}, we then have
% \begin{equation}
%     \begin{aligned}
%   & f(\m{x}^{k+1}, \m{y}^\star(\m{x}^{k+1}))-f(\m{x}^{k}, \m{y}^\star(\m{x}^{k}))  \leq \langle \m{x}^{k+1} - \m{x}^{k}, \nabla f(\m{x}^{k}, \m{y}^\star(\m{x}^{k})) \rangle + \frac{L}{2} {\Vert \m{x}^{k+1}-\m{x}^{k} \Vert}^2\\
%     & = - \Big \langle \frac{1}{m} \sum\limits_{i=1}^{m} \alpha_i \sum\limits_{k=0}^{K-1}  \nabla_x f_i(x_{i,\nu}, \m{y}^{t+1}) +\alpha \bar{\nabla} f(\m{x}^{k},\m{y}^{t+1}), \nabla f(\m{x}^{k} ,  \m{y}^\star(\m{x}^{k})) \Big \rangle \\
%     & + \frac{L}{2} \norm[\bigg]{\frac{1}{m}\sum\limits_{i=1}^{m} \alpha_i \sum\limits_{k=0}^{K-1} \nabla_x f_i(x_{i,\nu} ,\m{y}^{t+1}) + \alpha \bar{\nabla} f(\m{x}^{k},\m{y}^{t+1}) }^2.
%     \end{aligned}
% \label{eqn:iterimbnd1_ct}
% \end{equation}
% Just as in the proof of Theorem \ref{thm:speed_acc}, we now proceed to separately bound each of the two terms above, starting with the first term, as follows. 
% \begin{equation}
%     \begin{aligned}
%     &- \Big \langle \frac{1}{m} \sum\limits_{i=1}^{m} \alpha_i \sum\limits_{k=0}^{K-1}  \nabla f_i(x_{i,\nu}), \nabla f(\m{x}^{k}) \Big \rangle\\
%     &= - \Big \langle \frac{1}{m}\sum\limits_{i=1}^{m} \alpha_i \sum\limits_{k=0}^{K-1} \left( \nabla f_i(x_{i,\nu})-\nabla f_i(\m{x}^{k}) \right) + \frac{1}{m} \sum\limits_{i=1}^{m} \alpha_i \sum\limits_{k=0}^{K-1} \nabla f_i(\m{x}^{k}), \nabla f(\m{x}^{k}) \Big \rangle \\
%     &= - \Big \langle \frac{1}{m}\sum\limits_{i=1}^{m} \alpha_i \sum\limits_{k=0}^{K-1} \left( \nabla f_i(x_{i,\nu})-\nabla f_i(\m{x}^{k}) \right) + \frac{1}{m} \sum\limits_{i=1}^{m} \underbrace{\alpha_i \tau_i}_{\alpha} \nabla f_i(\m{x}^{k}), \nabla f(\m{x}^{k}) \Big \rangle \\
%     &= - \Big \langle \frac{1}{m}\sum\limits_{i=1}^{m} \alpha_i \sum\limits_{k=0}^{K-1} \left( \nabla f_i(x_{i,\nu})-\nabla f_i(\m{x}^{k}) \right), \nabla f(\m{x}^{k}) \Big \rangle  - \alpha {\Vert \nabla f(\m{x}^{k}) \Vert}^2 \\ 
%   & \overset{(a)} \leq \frac{1}{m} \left(\norm[\bigg]{\sum\limits_{i=1}^{m} \alpha_i \sum\limits_{k=0}^{K-1} \left( \nabla f_i(x_{i,\nu})-\nabla f_i(\m{x}^{k}) \right)}\right) \Vert \nabla f(\m{x}^{k}) \Vert - \alpha {\Vert \nabla f(\m{x}^{k}) \Vert}^2\\
%  & \overset{(b)} \leq \frac{1}{m} \left( {\sum\limits_{i=1}^{m} \alpha_i \sum\limits_{k=0}^{K-1} \Vert \nabla f_i(x_{i,\nu})-\nabla f_i(\m{x}^{k})\Vert}\right) \Vert \nabla f(\m{x}^{k}) \Vert - \alpha {\Vert \nabla f(\m{x}^{k}) \Vert}^2\\
% & \overset{(c)} \leq \frac{ L}{m} \left( {\sum\limits_{i=1}^{m} \alpha_i \sum\limits_{k=0}^{K-1} \Vert x_{i,\nu}-\m{x}^{k}\Vert}\right) \Vert \nabla f(\m{x}^{k}) \Vert - \alpha {\Vert \nabla f(\m{x}^{k}) \Vert}^2,
%     \end{aligned}
% \label{eqn:T1_thm_ct}
% \end{equation}
% where (a) follows from the Cauchy-Schwartz inequality, (b) follows from the triangle inequality, and (c) follows from the $L$-smoothness of each $f_i(\cdot)$. For the second term in \eqref{eqn:iterimbnd1_ct}, observe that 
% \begin{equation}
%     \begin{aligned}
%  \frac{L}{2} \norm[\bigg]{\frac{1}{m}\sum\limits_{i=1}^{m} \alpha_i \sum\limits_{k=0}^{K-1} \nabla f_i(x_{i,\nu})}^2 &= \frac{L}{2}\norm[\bigg]{\frac{1}{m}\sum\limits_{i=1}^{m} \alpha_i \sum\limits_{k=0}^{K-1} \left( \nabla f_i(x_{i,\nu})-\nabla f_i(\m{x}^{k}) \right) + \frac{1}{m} \sum\limits_{i=1}^{m} \alpha_i \sum\limits_{k=0}^{K-1} \nabla f_i(\m{x}^{k})}^2\\
%  &=\frac{ L}{2}\norm[\bigg]{\frac{1}{m}\sum\limits_{i=1}^{m} \alpha_i \sum\limits_{k=0}^{K-1} \left( \nabla f_i(x_{i,\nu})-\nabla f_i(\m{x}^{k}) \right) + \alpha \nabla f(\m{x}^{k})}^2\\
% & \overset{(a)} \leq L \norm[\bigg]{\frac{1}{m}\sum\limits_{i=1}^{m}\alpha_i \sum\limits_{k=0}^{K-1} \left( \nabla f_i(x_{i,\nu})-\nabla f_i(\m{x}^{k}) \right)}^2 + {\alpha}^2 L {\Vert \nabla f(\m{x}^{k}) \Vert}^2 \\
% & \overset{(b)} \leq \frac{L}{m}  \sum\limits_{i=1}^{m} {\alpha_i}^2 \norm[\bigg]{ \sum\limits_{k=0}^{K-1} \left( \nabla f_i(x_{i,\nu})-\nabla f_i(\m{x}^{k}) \right)}^2 + {\alpha}^2 L {\Vert \nabla f(\m{x}^{k}) \Vert}^2\\
% & \overset{(c)} \leq \frac{L }{m}  \sum\limits_{i=1}^{m} {\alpha_i}^2 \tau_i \sum\limits_{k=0}^{K-1} {\Vert  \nabla f_i(x_{i,\nu})-\nabla f_i(\m{x}^{k}) \Vert }^2 + {\alpha}^2 L {\Vert \nabla f(\m{x}^{k}) \Vert}^2 \\
% & \overset{(d)} \leq \frac{\alpha L^3}{m}  \sum\limits_{i=1}^{m} \alpha_i \sum\limits_{k=0}^{K-1} {\Vert  x_{i,\nu}-\m{x}^{k} \Vert }^2 + {\alpha}^2 L {\Vert \nabla f(\m{x}^{k}) \Vert}^2.
%     \end{aligned}
% \label{eqn:T2bound_ct}
% \end{equation}
% For (a), we used \eqref{eqn:rel_triangle} with $\gamma=1$; for (b) and (c), we used Jensen's inequality \eqref{eqn:Jensens}; and for (d), we used $\alpha_i \tau_i =\alpha$, and the $L$-smoothness of $f_i(\cdot)$. Plugging in the bounds \eqref{eqn:T1_thm_ct} and \eqref{eqn:T2bound_ct} in \eqref{eqn:iterimbnd1_ct}, and simplifying, we obtain \eqref{eqn:f_bound_ct}. 
% \end{proof}
